# Supplementary material for: Unveiling the weak radio quasar population at z $\geq$ 4
Source: arXiv:1909.11012 source file (2019-10-14)
Supplement: Supplementary file 1 [file supplementarytable.pdf]

**LIST OF STACKED AGN**

| Name | Right ascension (h m s) | Declination (° ′ ″) | Redshift | Reference |
|---|---|---|---|---|
| SDSS J000046.69+010951.2 | 00 00 46.69 | +01 09 51.24 | 4.25 | Pâris et al. (2012) |
| SDSS J000124.23+111212.6 | 00 01 24.23 | +11 12 12.69 | 4.30 | Pâris et al. (2017) |
| SDSS J000404.71+000039.0 | 00 04 04.71 | +00 00 39.08 | 4.31 | Pâris et al. (2012) |
| SDSS J000457.11−000538.7 | 00 04 57.11 | −00 05 38.78 | 4.05 | Pâris et al. (2012) |
| SDSS J000527.14+025813.2 | 00 05 27.15 | +02 58 13.29 | 4.11 | Pâris et al. (2012) |
| SDSS J000552.33−000655.6 | 00 05 52.33 | −00 06 55.65 | 5.86 | Pâris et al. (2012) |
| SDSS J000554.03+003042.0 | 00 05 54.03 | +00 30 42.04 | 4.14 | Pâris et al. (2017) |
| SDSS J000637.99−003656.2 | 00 06 38.00 | −00 36 56.30 | 4.44 | Pâris et al. (2012) |
| SDSS J000749.16+004119.6 | 00 07 49.17 | +00 41 19.61 | 4.78 | Schneider et al. (2007) |
| J000754.08−031730.82 | 00 07 54.08 | −03 17 30.82 | 4.76 | Wang et al. (2016) |
| PSO J002.1073−06.4345 | 00 08 25.77 | −06 26 04.42 | 5.93 | Jiang et al. (2015) |
| SDSS J001207.78+094720.2 | 00 12 07.79 | +09 47 20.23 | 4.75 | Pâris et al. (2014) |
| SDSS J001214.66+120344.8 | 00 12 14.66 | +12 03 44.89 | 4.11 | Pâris et al. (2017) |
| SDSS J001357.16−083334.7 | 00 13 57.17 | −08 33 34.74 | 4.19 | Pâris et al. (2017) |
| HRQC J001529.86−004904.3 | 00 15 29.86 | −00 49 04.30 | 4.93 | McGreer et al. (2013) |
| SDSS J001537.51+021908.8 | 00 15 37.51 | +02 19 08.88 | 4.23 | Pâris et al. (2012) |
| SDSS J001714.67−100055.4 | 00 17 14.68 | −10 00 55.43 | 5.01 | Schneider et al. (2005) |
| SDSS J001813.88+142455.6 | 00 18 13.89 | +14 24 55.68 | 4.23 | Pâris et al. (2017) |
| SDSS J001918.43+150611.3 | 00 19 18.44 | +15 06 11.37 | 4.14 | Schneider et al. (2005) |
| SDSS J001950.05−004040.8 | 00 19 50.06 | −00 40 40.83 | 4.34 | Schneider et al. (2005) |
| SDSS J002330.66−001836.6 | 00 23 30.67 | −00 18 36.61 | 5.04 | Pâris et al. (2012) |
| SDSS J002417.61+000846.2 | 00 24 17.62 | +00 08 46.22 | 4.00 | Schneider et al. (2007) |
| J002526.84−014532.51 | 00 25 26.84 | −01 45 32.51 | 5.07 | Wang et al. (2016) |
| PSO J007.0273+04.9571 | 00 28 06.56 | +04 57 25.70 | 5.99 | Bañados et al. (2014) |
| SDSS J002825.02+010604.2 | 00 28 25.02 | +01 06 04.29 | 4.12 | Pâris et al. (2017) |
| PC 0027+0525 | 00 29 50.00 | +05 42 04.00 | 4.10 | Schneider, Schmidt, & Gunn (1997) |
| PC 0027+0521 | 00 30 04.53 | +05 38 14.00 | 4.21 | Schneider, Schmidt, & Gunn (1994a) |
| SDSS J003117.70+001705.0 | 00 31 17.70 | +00 17 05.06 | 4.34 | Pâris et al. (2012) |
| J003125.86+071036.92 | 00 31 25.86 | +07 10 36.92 | 5.33 | Wang et al. (2016) |
| SDSS J003304.82−003102.4 | 00 33 04.82 | −00 31 02.41 | 4.53 | Pâris et al. (2017) |
| CFHQS J00331−0125 | 00 33 11.40 | −01 25 25.00 | 6.13 | Willott et al. (2007) |
| SDSS J003341.89+012705.6 | 00 33 41.90 | +01 27 05.67 | 4.28 | Pâris et al. (2012) |
| SDSS J003401.28−080359.4 | 00 34 01.29 | −08 03 59.48 | 4.03 | Pâris et al. (2017) |
| SDSS J003430.48+055127.1 | 00 34 30.49 | +05 51 27.11 | 4.07 | Pâris et al. (2014) |
| SDSS J003525.29+004002.7 | 00 35 25.29 | +00 40 02.73 | 4.75 | Schneider et al. (2007) |
| SDSS J003605.64+010344.9 | 00 36 05.65 | +01 03 44.97 | 4.70 | Pâris et al. (2012) |
| SDSS J003618.84−004629.9 | 00 36 18.84 | −00 46 29.93 | 4.04 | Pâris et al. (2017) |
| SDSSp J003714.12−005603.9 | 00 37 14.12 | −00 56 03.90 | 4.35 | Anderson et al. (2001) |
| SDSS J003716.52+032327.7 | 00 37 16.53 | +03 23 27.75 | 4.07 | Pâris et al. (2017) |
| PSO J009.3573−08.1190 | 00 37 25.76 | −08 07 08.46 | 5.72 | Bañados et al. (2016) |
| SDSS J003813.59+005731.8 | 00 38 13.59 | +00 57 31.84 | 4.05 | Pâris et al. (2012) |
| PSO J009.7355−10.4316 | 00 38 56.52 | −10 25 53.90 | 5.95 | Bañados et al. (2016) |
| PC 0036+0032 | 00 38 59.67 | +00 48 59.00 | 4.51 | Schneider, Schmidt, & Gunn (1997) |
| SDSS J004018.69+050127.4 | 00 40 18.70 | +05 01 27.42 | 4.47 | Pâris et al. (2012) |
| SDSS J004046.20+033655.2 | 00 40 46.20 | +03 36 55.30 | 4.11 | Pâris et al. (2017) |
| SDSS J004054.65−091526.8 | 00 40 54.65 | −09 15 26.81 | 4.98 | Collinge et al. (2005) |
| SDSS J004503.87−030153.9 | 00 45 03.88 | −03 01 53.91 | 4.04 | Pâris et al. (2017) |
| SDSS J004716.34−003550.2 | 00 47 16.34 | −00 35 50.22 | 4.19 | Schneider et al. (2007) |
| SDSS J004905.94−003134.3 | 00 49 05.94 | −00 31 34.32 | 4.17 | Schneider et al. (2007) |
| SDSS J004905.95+002237.3 | 00 49 05.96 | +00 22 37.38 | 4.42 | Pâris et al. (2012) |
| SDSS J005006.35−005319.2 | 00 50 06.35 | −00 53 19.29 | 4.31 | Schneider et al. (2005) |
| SDSS J005421.42−010921.7 | 00 54 21.43 | −01 09 21.71 | 5.02 | Schneider et al. (2007) |

| | | | | |
|---|---|---|---|---|
| CFHQS J00550+0146 | 00 55 02.93 | +01 46 19.00 | 6.02 | Willott et al. (2009) |
| J005527.18+122840.67 | 00 55 27.18 | +12 28 40.67 | 4.70 | Wang et al. (2016) |
| SDSS J005554.26+094143.6 | 00 55 54.27 | +09 41 43.68 | 4.01 | Pâris et al. (2014) |
| HRQC J005703.20+001032.3 | 00 57 03.20 | +00 10 32.30 | 4.84 | McGreer et al. (2013) |
| PSS J0059+0003 | 00 59 22.65 | +00 03 01.41 | 4.16 | Kennefick et al. (1995a) |
| SDSS J010252.91+115948.3 | 01 02 52.92 | +11 59 48.36 | 4.15 | Pâris et al. (2014) |
| SDSS J010326.89+005538.6 | 01 03 26.90 | +00 55 38.66 | 4.16 | Pâris et al. (2017) |
| SDSS J010523.75−054402.4 | 01 05 23.75 | −05 44 02.44 | 4.01 | Pâris et al. (2017) |
| BRI 0103+0032 | 01 06 19.24 | +00 48 23.31 | 4.44 | Smith et al. (1994b) |
| PC 0104+0215 | 01 06 49.67 | +02 31 01.00 | 4.17 | Schneider, Schmidt, & Gunn (1989a) |
| J010806.60+071120.6 | 01 08 06.60 | +07 11 20.60 | 5.53 | Yang et al. (2017) |
| HRQC J010829.96−010015.6 | 01 08 29.96 | −01 00 15.60 | 5.11 | McGreer et al. (2013) |
| SDSS J010846.30+003659.5 | 01 08 46.30 | +00 36 59.57 | 4.03 | Pâris et al. (2012) |
| SDSS J011010.22+002419.5 | 01 10 10.23 | +00 24 19.59 | 4.68 | Pâris et al. (2012) |
| SDSS J011246.51−023858.1 | 01 12 46.52 | −02 38 58.16 | 4.12 | Pâris et al. (2012) |
| SDSS J011333.19−000021.2 | 01 13 33.19 | −00 00 21.23 | 4.20 | Pâris et al. (2012) |
| SDSS J011352.01+005233.9 | 01 13 52.02 | +00 52 33.97 | 4.22 | Pâris et al. (2012) |
| J011353.75+055951.1 | 01 13 53.75 | +05 59 51.10 | 5.00 | Yang et al. (2017) |
| HRQC J011544.78+001514.9 | 01 15 44.78 | +00 15 14.90 | 5.10 | McGreer et al. (2013) |
| J011546.27−025312.24 | 01 15 46.27 | −02 53 12.24 | 5.07 | Wang et al. (2016) |
| J011614.30+053817.70 | 01 16 14.30 | +05 38 17.70 | 5.33 | Wang et al. (2016) |
| SDSS J011702.89+074713.5 | 01 17 02.89 | +07 47 13.53 | 4.33 | Pâris et al. (2017) |
| PSS J0118+0320 | 01 18 52.67 | +03 20 50.00 | 4.23 | Djorgovski et al. (2001) |
| SDSS J011951.63+072045.6 | 01 19 51.64 | +07 20 45.66 | 4.04 | Pâris et al. (2014) |
| SDSS J012019.99+000735.6 | 01 20 19.99 | +00 07 35.61 | 4.09 | Schneider et al. (2005) |
| SDSS J012135.57+001205.8 | 01 21 35.57 | +00 12 05.81 | 4.70 | Pâris et al. (2017) |
| SDSS J012247.34+121624.0 | 01 22 47.34 | +12 16 24.00 | 4.82 | Yi et al. (2017) |
| SDSS J012405.70−004407.8 | 01 24 05.71 | −00 44 07.87 | 4.07 | Schneider et al. (2007) |
| SDSS J012509.42−104300.8 | 01 25 09.42 | −10 43 00.88 | 4.49 | Schneider et al. (2005) |
| SDSS J012700.69−004559.1 | 01 27 00.69 | −00 45 59.18 | 4.11 | Schneider et al. (2007) |
| HRQC J012820.81−001636.9 | 01 28 20.81 | −00 16 36.90 | 4.74 | McGreer et al. (2013) |
| HRQC J012907.44−002845.5 | 01 29 07.44 | −00 28 45.50 | 5.01 | McGreer et al. (2013) |
| SDSS J012919.91+021311.8 | 01 29 19.92 | +02 13 11.89 | 4.13 | Pâris et al. (2014) |
| SDSS J01299−0035 | 01 29 58.53 | −00 35 39.00 | 5.78 | Jiang et al. (2009) |
| PSS J0131+0633 | 01 31 12.20 | +06 33 40.00 | 4.42 | Péroux et al. (2001) |
| PSO J023.0071−02.2675 | 01 32 01.70 | −02 16 03.11 | 5.90 | Bañados et al. (2016) |
| J013224.89−030718.45 | 01 32 24.89 | −03 07 18.45 | 4.83 | Wang et al. (2016) |
| SDSS J013242.76−094301.5 | 01 32 42.77 | −09 43 01.60 | 4.26 | Schneider et al. (2005) |
| SDSS J01334+0106 | 01 33 26.87 | +01 06 38.00 | 5.30 | Chiu et al. (2005) |
| PSS J0133+0400 | 01 33 40.32 | +04 00 59.77 | 4.17 | Péroux et al. (2001) |
| CFHQS J0136+0226 | 01 36 03.20 | +02 26 06.00 | 6.21 | Willott et al. (2010a) |
| SDSS J013650.51+025821.7 | 01 36 50.51 | +02 58 21.79 | 4.13 | Pâris et al. (2012) |
| SDSS J013829.60−095247.4 | 01 38 29.61 | −09 52 47.42 | 4.17 | Schneider et al. (2005) |
| SDSS J013852.56+074153.9 | 01 38 52.57 | +07 41 53.92 | 4.03 | Pâris et al. (2012) |
| SDSS J014047.09+050459.3 | 01 40 47.09 | +05 04 59.31 | 4.09 | Pâris et al. (2017) |
| SDSS J014328.37−100019.4 | 01 43 28.38 | −10 00 19.40 | 4.50 | Schneider et al. (2005) |
| SDSS J014452.68−011044.2 | 01 44 52.69 | −01 10 44.28 | 4.02 | Pâris et al. (2012) |
| SDSS J014542.48−005118.7 | 01 45 42.49 | −00 51 18.78 | 4.15 | Pâris et al. (2012) |
| SDSS J014609.33−092918.2 | 01 46 09.34 | −09 29 18.24 | 4.16 | Schneider et al. (2005) |
| J014741.53−030247.88 | 01 47 41.53 | −03 02 47.88 | 4.75 | Wang et al. (2016) |
| ULAS J0148+0600 | 01 48 37.64 | +06 00 20.10 | 5.96 | Jiang et al. (2015) |
| SDSS J014852.49+070650.8 | 01 48 52.50 | +07 06 50.89 | 4.05 | Pâris et al. (2012) |
| SDSS J015012.22+001622.7 | 01 50 12.23 | +00 16 22.78 | 4.46 | Pâris et al. (2012) |
| PSS J0152+0735 | 01 52 11.06 | +07 35 50.13 | 4.07 | Constantin et al. (2002) |
| SDSS J015252.54−022654.8 | 01 52 52.55 | −02 26 54.84 | 4.01 | Pâris et al. (2012) |
| SDSS J015321.05+122352.9 | 01 53 21.06 | +12 23 52.99 | 4.06 | Pâris et al. (2014) |
| SDSS J015430.39+063901.4 | 01 54 30.40 | +06 39 01.44 | 4.07 | Pâris et al. (2012) |

| | | | | |
|---|---|---|---|---|
| SDSS J015447.97−000951.8 | 01 54 47.97 | −00 09 51.85 | 4.05 | Pâris et al. (2012) |
| SDSS J015518.78−004056.2 | 01 55 18.78 | −00 40 56.24 | 4.25 | Pâris et al. (2012) |
| J015533.28+041506.74 | 01 55 33.28 | +04 15 06.74 | 5.37 | Wang et al. (2016) |
| J015618.99−044139.88 | 01 56 18.99 | −04 41 39.88 | 4.94 | Wang et al. (2016) |
| SDSS J015704.09+122858.2 | 01 57 04.10 | +12 28 58.30 | 4.17 | Schneider et al. (2005) |
| HRQC J015705.11−011248.8 | 01 57 05.11 | −01 12 48.80 | 4.79 | McGreer et al. (2013) |
| SDSS J015722.90+020239.4 | 01 57 22.90 | +02 02 39.50 | 4.50 | Pâris et al. (2012) |
| HRQC J015823.92−003636.3 | 01 58 23.92 | −00 36 36.30 | 4.89 | McGreer et al. (2013) |
| SDSS J015934.80+001730.8 | 01 59 34.81 | +00 17 30.88 | 4.16 | Pâris et al. (2012) |
| HRQC J020001.00+001212.9 | 02 00 01.00 | +00 12 12.90 | 4.68 | McGreer et al. (2013) |
| SDSS J020150.31−070013.2 | 02 01 50.31 | −07 00 13.21 | 4.08 | Pâris et al. (2014) |
| SDSS J020152.53−094733.3 | 02 01 52.53 | −09 47 33.40 | 4.03 | Pâris et al. (2017) |
| SDSS J020231.14−042246.8 | 02 02 31.15 | −04 22 46.85 | 4.27 | Pâris et al. (2017) |
| J0202−0251 | 02 02 58.21 | −02 51 53.60 | 6.03 | Matsuoka et al. (2018b) |
| SDSS J020326.46−003954.0 | 02 03 26.47 | −00 39 54.04 | 4.16 | Schneider et al. (2007) |
| ULAS J02035+0012 | 02 03 32.40 | +00 12 29.00 | 5.86 | Venemans et al. (2007) |
| J0206−0255 | 02 06 11.20 | −02 55 37.80 | 6.03 | Matsuoka et al. (2018b) |
| SDSSp J020651.37+121624.4 | 02 06 51.37 | +12 16 24.40 | 4.81 | Anderson et al. (2001) |
| SDSS J020730.12+031853.6 | 02 07 30.13 | +03 18 53.68 | 4.06 | Pâris et al. (2012) |
| HRQC J020804.31−011234.3 | 02 08 04.31 | −01 12 34.30 | 5.23 | McGreer et al. (2013) |
| SDSS J020810.73−093016.3 | 02 08 10.73 | −09 30 16.34 | 4.08 | Pâris et al. (2017) |
| SDSS J020925.25−000249.9 | 02 09 25.25 | −00 02 49.92 | 4.20 | Pâris et al. (2012) |
| PSS J0209+0517 | 02 09 44.62 | +05 17 13.66 | 4.18 | Péroux et al. (2001) |
| CFHQS J021013−045620 | 02 10 13.20 | −04 56 21.00 | 6.44 | Willott et al. (2010b) |
| HRQC J021056.67+000304.7 | 02 10 56.67 | +00 03 04.70 | 5.05 | McGreer et al. (2013) |
| SDSS J021102.72−000910.3 | 02 11 02.73 | −00 09 10.36 | 4.92 | Pâris et al. (2012) |
| J0211−0203 | 02 11 44.53 | −02 03 03.90 | 6.37 | Chehade et al. (2018) |
| SDSS J021310.20+011009.1 | 02 13 10.20 | +01 10 09.15 | 4.21 | Pâris et al. (2012) |
| IMS J021315−043341 | 02 13 15.00 | −04 33 40.50 | 4.88 | Kim et al. (2019) |
| J0213−0626 | 02 13 16.94 | −06 26 15.20 | 6.72 | Chehade et al. (2018) |
| SDSS J021338.63−051616.1 | 02 13 38.64 | −05 16 16.14 | 4.53 | Pâris et al. (2017) |
| SDSS J021350.50+022338.5 | 02 13 50.51 | +02 23 38.51 | 4.11 | Pâris et al. (2017) |
| SDSS J021352.44+030623.1 | 02 13 52.44 | +03 06 23.18 | 4.09 | Pâris et al. (2012) |
| SDSS J021419.41−010716.9 | 02 14 19.42 | −01 07 16.96 | 4.60 | Schneider et al. (2007) |
| IMS J021523−052946 | 02 15 23.29 | −05 29 45.90 | 5.13 | Kim et al. (2019) |
| SDSS J021527.28−060359.9 | 02 15 27.29 | −06 03 59.94 | 4.07 | Pâris et al. (2014) |
| SDSS J021615.48+071709.4 | 02 16 15.48 | +07 17 09.48 | 4.02 | Pâris et al. (2012) |
| CFHQS J02164−0455 | 02 16 27.80 | −04 55 34.00 | 6.01 | Willott et al. (2009) |
| SDSS J021639.97+064008.2 | 02 16 39.97 | +06 40 08.26 | 4.18 | Pâris et al. (2012) |
| SDSS J021712.98−054109.8 | 02 17 12.98 | −05 41 09.80 | 4.56 | Pâris et al. (2017) |
| J0217−0208 | 02 17 21.59 | −02 08 52.60 | 6.20 | Matsuoka et al. (2018b) |
| IMS J021811−064843 | 02 18 10.80 | −06 48 42.60 | 4.87 | Kim et al. (2019) |
| HRQC J021821.08−002745.7 | 02 18 21.08 | −00 27 45.70 | 5.11 | McGreer et al. (2013) |
| SXDF 0888 | 02 18 44.48 | −04 48 24.82 | 4.56 | Hiroi et al. (2012) |
| SDSS J021942.62−001136.9 | 02 19 42.62 | −00 11 36.97 | 4.51 | Pâris et al. (2017) |
| SXDF 1238 | 02 20 22.04 | −05 04 29.39 | 4.16 | Hiroi et al. (2012) |
| SDSS J022027.90+000636.9 | 02 20 27.90 | +00 06 36.93 | 4.08 | Pâris et al. (2012) |
| J0220−0432 | 02 20 29.72 | −04 32 04.00 | 5.90 | Chehade et al. (2018) |
| IMS J022112−034232 | 02 21 12.32 | −03 42 31.80 | 4.98 | Kim et al. (2019) |
| SDSS J022112.62−034252.2 | 02 21 12.62 | −03 42 52.27 | 5.01 | Pâris et al. (2017) |
| CFHQS J0221−0802 | 02 21 22.73 | −08 02 52.00 | 6.16 | Willott et al. (2010a) |
| SDSS J022316.02+005822.4 | 02 23 16.03 | +00 58 22.46 | 4.41 | Pâris et al. (2012) |
| XWAS J022339.3−045341 | 02 23 39.26 | −04 53 40.70 | 4.25 | Esquej et al. (2013) |
| PSO J036.5078+03.0498 | 02 26 01.87 | +03 02 59.42 | 6.54 | Venemans et al. (2015a) |
| Q J02261+0017 | 02 26 06.60 | +00 17 43.00 | 4.00 | Hall et al. (2000) |
| Q J02262+0021 | 02 26 12.02 | +00 21 57.41 | 4.62 | Hall et al. (2000) |
| XWAS J022657.6−033336 | 02 26 57.64 | −03 33 35.44 | 4.36 | Esquej et al. (2013) |

| | | | | |
|---|---|---|---|---|
| CFHQS J02277−0605 | 02 27 43.33 | −06 05 30.00 | 6.20 | Willott et al. (2009) |
| SDSS J022848.45−013635.1 | 02 28 48.45 | −01 36 35.18 | 4.01 | Pâris et al. (2012) |
| ALH023002+004647 | 02 30 02.27 | +00 46 46.80 | 5.41 | Matute et al. (2013) |
| HRQC J023006.05+002625.1 | 02 30 06.05 | +00 26 25.10 | 4.62 | McGreer et al. (2013) |
| SDSS J023058.67−041358.1 | 02 30 58.68 | −04 13 58.11 | 4.01 | Pâris et al. (2017) |
| SDSS J023137.64−072854.4 | 02 31 37.65 | −07 28 54.45 | 5.42 | Schneider et al. (2005) |
| SDSS J023226.13−053729.4 | 02 32 26.14 | −05 37 29.47 | 4.55 | Pâris et al. (2017) |
| SDSS J023519.65−042855.7 | 02 35 19.66 | −04 28 55.78 | 4.15 | Pâris et al. (2012) |
| J0235−0532 | 02 35 42.42 | −05 32 41.60 | 6.09 | Matsuoka et al. (2018b) |
| HRQC J023633.84−010839.1 | 02 36 33.84 | −01 08 39.10 | 4.97 | McGreer et al. (2013) |
| SDSS J023923.47−081005.0 | 02 39 23.48 | −08 10 05.09 | 4.02 | Pâris et al. (2017) |
| SDSS J02395−0045 | 02 39 30.20 | −00 45 05.00 | 5.82 | Jiang et al. (2009) |
| SDSS J023935.26+010256.8 | 02 39 35.26 | +01 02 56.86 | 4.07 | Pâris et al. (2012) |
| SDSS J024010.01−030059.6 | 02 40 10.02 | −03 00 59.67 | 4.01 | Pâris et al. (2012) |
| J024152.92+043553.46 | 02 41 52.92 | +04 35 53.46 | 5.22 | Wang et al. (2016) |
| BRI 0241−0146 | 02 44 01.87 | −01 34 04.00 | 4.01 | Constantin et al. (2002) |
| SDSS J024443.24+003145.1 | 02 44 43.25 | +00 31 45.12 | 4.03 | Pâris et al. (2012) |
| SDSS J024447.79−081606.0 | 02 44 47.79 | −08 16 06.03 | 4.07 | Schneider et al. (2005) |
| J024601.95+035054.12 | 02 46 01.95 | +03 50 54.12 | 4.96 | Wang et al. (2016) |
| J024643.78+061045.74 | 02 46 43.78 | +06 10 45.74 | 4.57 | Wang et al. (2016) |
| BR 0245−0608 | 02 47 56.60 | −05 55 59.00 | 4.24 | Storrie-Lombardi et al. (1996) |
| SDSS J025019.78+004650.2 | 02 50 19.78 | +00 46 50.25 | 4.77 | Pâris et al. (2017) |
| SDSS J025039.17−065405.1 | 02 50 39.18 | −06 54 05.13 | 4.48 | Schneider et al. (2005) |
| PSO J042.6690−02.9174 | 02 50 40.58 | −02 55 02.82 | 5.89 | Bañados et al. (2016) |
| J025121.33+033317.42 | 02 51 21.33 | +03 33 17.42 | 5.00 | Wang et al. (2016) |
| SDSS J025159.41−084258.1 | 02 51 59.41 | −08 42 58.11 | 4.26 | Schneider et al. (2005) |
| SDSS J025204.28+003137.0 | 02 52 04.29 | +00 31 37.10 | 4.15 | Pâris et al. (2017) |
| HRQC J025211.24+004431.8 | 02 52 11.24 | +00 44 31.80 | 4.76 | McGreer et al. (2013) |
| SDSS J025311.60+000051.2 | 02 53 11.61 | +00 00 51.22 | 4.21 | Pâris et al. (2012) |
| SDSS J025518.58+004847.5 | 02 55 18.58 | +00 48 47.55 | 4.01 | Schneider et al. (2005) |
| HRQC J025617.73+001904.2 | 02 56 17.73 | +00 19 04.20 | 4.80 | McGreer et al. (2013) |
| SDSS J025635.54−010357.7 | 02 56 35.55 | −01 03 57.80 | 4.10 | Pâris et al. (2017) |
| HRQC J025645.74+000200.1 | 02 56 45.74 | +00 02 00.10 | 4.95 | McGreer et al. (2013) |
| SDSS J025647.05−085041.3 | 02 56 47.05 | −08 50 41.38 | 4.23 | Schneider et al. (2005) |
| SDSS J025754.12+012006.9 | 02 57 54.13 | +01 20 07.00 | 4.24 | Pâris et al. (2017) |
| RD J030117+002025 | 03 01 17.13 | +00 20 26.00 | 5.50 | Stern et al. (2000) |
| BR J0302−0156 | 03 02 53.07 | −01 56 06.00 | 4.25 | Storrie-Lombardi et al. (2001) |
| HRQC J030315.05−000347.6 | 03 03 15.05 | −00 03 47.60 | 4.72 | McGreer et al. (2013) |
| SDSS J03035−0019 | 03 03 31.40 | −00 19 12.00 | 6.07 | Jiang et al. (2008) |
| SDSS J031036.97−001457.0 | 03 10 36.97 | −00 14 57.02 | 4.72 | Schneider et al. (2007) |
| SDSS J031213.98−062658.8 | 03 12 13.98 | −06 26 58.85 | 4.03 | Schneider et al. (2005) |
| PSS J0315+0524 | 03 15 48.47 | +05 24 59.00 | 4.23 | Djorgovski et al. (2001) |
| J032407.69+042613.29 | 03 24 07.69 | +04 26 13.29 | 4.72 | Wang et al. (2016) |
| SDSSp J032459.10−005705.1 | 03 24 59.10 | −00 57 05.10 | 4.80 | Fan et al. (2001b) |
| SDSS J032608.12−003340.1 | 03 26 08.13 | −00 33 40.11 | 4.16 | Schneider et al. (2005) |
| HRQC J032707.86+000344.1 | 03 27 07.86 | +00 03 44.10 | 4.88 | McGreer et al. (2013) |
| SDSS J033119.66−074143.1 | 03 31 19.67 | −07 41 43.14 | 4.74 | Schneider et al. (2005) |
| HRQC J033231.34−000217.3 | 03 32 31.34 | −00 02 17.30 | 4.68 | McGreer et al. (2013) |
| SDSS J033305.32−053708.9 | 03 33 05.32 | −05 37 08.91 | 4.22 | Schneider et al. (2005) |
| SDSSp J033414.10+004056.6 | 03 34 14.10 | +00 40 56.60 | 4.33 | Fan et al. (2001b) |
| SDSS J033829.30+002156.2 | 03 38 29.31 | +00 21 56.26 | 5.03 | Schneider et al. (2005) |
| Q J03385+0018 | 03 38 30.00 | +00 18 40.00 | 4.96 | Djorgovski et al. (2003) |
| SDSS J034109.35−064805.1 | 03 41 09.35 | −06 48 05.12 | 4.07 | Schneider et al. (2005) |
| SDSS J034541.50−072315.3 | 03 45 41.51 | −07 23 15.36 | 4.05 | Schneider et al. (2005) |
| HRQC J034612.30−004512.7 | 03 46 12.30 | −00 45 12.70 | 4.80 | McGreer et al. (2013) |
| HRQC J034959.40+003403.5 | 03 49 59.40 | +00 34 03.50 | 5.20 | McGreer et al. (2013) |
| HRQC J035043.92+001717.7 | 03 50 43.92 | +00 17 17.70 | 4.75 | McGreer et al. (2013) |

| | | | | |
|---|---|---|---|---|
| SDSS J035214.33−001941.0 | 03 52 14.34 | −00 19 41.09 | 4.19 | Schneider et al. (2007) |
| SDSS J03538+0104 | 03 53 49.73 | +01 04 04.00 | 6.05 | Jiang et al. (2008) |
| SDSS J072559.05+432303.8 | 07 25 59.06 | +43 23 03.82 | 4.03 | Schneider et al. (2007) |
| SDSS J072737.89+411424.6 | 07 27 37.90 | +41 14 24.61 | 4.29 | Pâris et al. (2017) |
| SDSS J073103.12+445949.4 | 07 31 03.13 | +44 59 49.43 | 4.98 | Schneider et al. (2007) |
| SDSS J073146.99+364346.4 | 07 31 47.00 | +36 43 46.48 | 4.04 | Schneider et al. (2005) |
| J073231.28+325618.33 | 07 32 31.28 | +32 56 18.33 | 4.76 | Wang et al. (2016) |
| SDSS J073354.91+321241.4 | 07 33 54.92 | +32 12 41.42 | 4.45 | Schneider et al. (2005) |
| SDSS J073703.71+454405.0 | 07 37 03.71 | +45 44 05.06 | 4.37 | Schneider et al. (2007) |
| SDSS J073748.60+263205.1 | 07 37 48.61 | +26 32 05.16 | 4.55 | Schneider et al. (2005) |
| SDSS J073900.39+480504.3 | 07 39 00.39 | +48 05 04.31 | 4.50 | Schneider et al. (2007) |
| SDSS J073900.51+432227.3 | 07 39 00.52 | +43 22 27.37 | 4.13 | Pâris et al. (2012) |
| SDSS J073936.45+222635.0 | 07 39 36.46 | +22 26 35.09 | 4.19 | Pâris et al. (2017) |
| SDSS J074000.35+463929.0 | 07 40 00.35 | +46 39 29.05 | 4.27 | Pâris et al. (2017) |
| ChaMP J074115.5+310815 | 07 41 15.54 | +31 08 15.41 | 4.48 | Trichas et al. (2012) |
| SDSS J074211.16+250730.7 | 07 42 11.16 | +25 07 30.74 | 4.52 | Schneider et al. (2005) |
| SDSS J074349.44+353034.7 | 07 43 49.45 | +35 30 34.74 | 4.14 | Pâris et al. (2012) |
| SDSS J074354.28+464130.2 | 07 43 54.29 | +46 41 30.20 | 4.37 | Pâris et al. (2017) |
| SDSS J074534.32+373532.0 | 07 45 34.33 | +37 35 32.07 | 4.12 | Pâris et al. (2012) |
| SDSS J074611.43+454902.1 | 07 46 11.44 | +45 49 02.15 | 4.19 | Pâris et al. (2017) |
| SDSS J074640.16+344624.8 | 07 46 40.17 | +34 46 24.83 | 4.01 | Schneider et al. (2005) |
| SDSS J074653.43+470517.7 | 07 46 53.44 | +47 05 17.79 | 4.79 | Schneider et al. (2007) |
| SDSS J074743.29+331637.4 | 07 47 43.29 | +33 16 37.47 | 4.02 | Pâris et al. (2012) |
| PSS J0747+4434 | 07 47 49.74 | +44 34 17.06 | 4.44 | Péroux et al. (2001) |
| SDSS J074853.86+170829.8 | 07 48 53.87 | +17 08 29.89 | 4.65 | Schneider et al. (2007) |
| SDSS J074907.57+355543.8 | 07 49 07.58 | +35 55 43.84 | 4.26 | Schneider et al. (2005) |
| SDSS J075052.59+300334.1 | 07 50 52.60 | +30 03 34.18 | 4.06 | Pâris et al. (2017) |
| SDSS J075103.96+424211.6 | 07 51 03.96 | +42 42 11.60 | 4.17 | Schneider et al. (2005) |
| SDSS J075111.06+300518.9 | 07 51 11.06 | +30 05 19.00 | 4.24 | Pâris et al. (2017) |
| SDSS J075204.16+252200.7 | 07 52 04.16 | +25 22 00.74 | 4.19 | Schneider et al. (2005) |
| SDSS J075239.74+465050.6 | 07 52 39.75 | +46 50 50.61 | 4.09 | Pâris et al. (2017) |
| SDSS J075313.81+330327.6 | 07 53 13.82 | +33 03 27.66 | 4.01 | Schneider et al. (2005) |
| SDSS J075347.41+281805.1 | 07 53 47.41 | +28 18 05.19 | 4.03 | Pâris et al. (2017) |
| SDSS J075412.18+253229.7 | 07 54 12.19 | +25 32 29.79 | 4.02 | Schneider et al. (2005) |
| SDSS J075437.47+122224.9 | 07 54 37.48 | +12 22 24.98 | 4.14 | Pâris et al. (2012) |
| SDSS J075443.65+331829.9 | 07 54 43.65 | +33 18 29.91 | 4.10 | Pâris et al. (2017) |
| PC 0751+5623 | 07 55 43.93 | +56 15 08.00 | 4.28 | Schneider, Schmidt, & Gunn (1989a) |
| SDSS J075553.78+180807.2 | 07 55 53.79 | +18 08 07.26 | 4.05 | Schneider et al. (2007) |
| SDSS J075612.88+291844.8 | 07 56 12.88 | +29 18 44.88 | 4.23 | Pâris et al. (2017) |
| SDSS J075618.13+410408.6 | 07 56 18.14 | +41 04 08.61 | 5.06 | Schneider et al. (2005) |
| SDSS J075652.07+450258.8 | 07 56 52.07 | +45 02 58.86 | 4.74 | Pâris et al. (2017) |
| SDSS J075703.74+201411.0 | 07 57 03.74 | +20 14 11.02 | 4.30 | Schneider et al. (2007) |
| SDSS J075732.89+441424.6 | 07 57 32.89 | +44 14 24.66 | 4.18 | Schneider et al. (2005) |
| SDSS J075847.85+483210.3 | 07 58 47.86 | +48 32 10.37 | 4.49 | Pâris et al. (2017) |
| SDSS J075903.20+524900.2 | 07 59 03.21 | +52 49 00.21 | 4.32 | Pâris et al. (2017) |
| SDSS J075907.57+180054.7 | 07 59 07.58 | +18 00 54.71 | 4.78 | Schneider et al. (2007) |
| SDSS J075946.29+381709.6 | 07 59 46.29 | +38 17 09.69 | 4.19 | Pâris et al. (2017) |
| SDSS J080023.01+305101.2 | 08 00 23.01 | +30 51 01.26 | 4.67 | Schneider et al. (2005) |
| SDSS J080143.37+324139.4 | 08 01 43.38 | +32 41 39.47 | 4.21 | Pâris et al. (2012) |
| SDSS J080159.25+433625.0 | 08 01 59.26 | +43 36 25.02 | 4.17 | Schneider et al. (2005) |
| SDSS J080207.15+180447.2 | 08 02 07.16 | +18 04 47.25 | 4.13 | Pâris et al. (2014) |
| DELS J080305.42+313834.2 | 08 03 05.42 | +31 38 34.20 | 6.38 | Wang et al. (2018) |
| J080306.19+403958.96 | 08 03 06.19 | +40 39 58.96 | 4.79 | Wang et al. (2016) |
| SDSS J080549.93+482345.7 | 08 05 49.94 | +48 23 45.79 | 4.20 | Pâris et al. (2017) |
| SDSS J080550.66+113725.7 | 08 05 50.66 | +11 37 25.71 | 4.07 | Pâris et al. (2012) |
| SDSS J080557.40+064428.5 | 08 05 57.40 | +06 44 28.53 | 4.01 | Schneider et al. (2007) |
| SDSS J080610.60+143712.9 | 08 06 10.61 | +14 37 13.00 | 4.74 | Schneider et al. (2010) |

| | | | | |
|---|---|---|---|---|
| SDSS J080657.51+311459.4 | 08 06 57.51 | +31 14 59.46 | 4.08 | Pâris et al. (2017) |
| SDSS J080715.11+132805.1 | 08 07 15.12 | +13 28 05.18 | 4.87 | Schneider et al. (2010) |
| SDSS J080723.51+544221.2 | 08 07 23.52 | +54 42 21.23 | 4.00 | Schneider et al. (2007) |
| PSS J0808+5215 | 08 08 49.43 | +52 15 15.31 | 4.47 | Djorgovski et al. (2001) |
| SDSS J081045.68+275041.7 | 08 10 45.68 | +27 50 41.70 | 4.28 | Pâris et al. (2014) |
| SDSS J0810+5105 | 08 10 54.31 | +51 05 40.10 | 5.82 | Jiang et al. (2016) |
| SDSS J081054.87+460357.8 | 08 10 54.88 | +46 03 57.86 | 4.09 | Pâris et al. (2017) |
| SDSS J081159.33+123638.5 | 08 11 59.33 | +12 36 38.57 | 4.85 | Schneider et al. (2010) |
| SDSS J081241.13+442129.0 | 08 12 41.13 | +44 21 29.04 | 4.34 | Schneider et al. (2005) |
| J081248.82+044056.54 | 08 12 48.82 | +04 40 56.54 | 5.29 | Wang et al. (2016) |
| SDSS J081400.53+392241.5 | 08 14 00.54 | +39 22 41.52 | 4.01 | Pâris et al. (2017) |
| SDSS J081424.79+343233.3 | 08 14 24.79 | +34 32 33.36 | 4.12 | Pâris et al. (2017) |
| SDSS J081518.56+291153.9 | 08 15 18.57 | +29 11 53.90 | 4.26 | Pâris et al. (2017) |
| SDSS J081653.54+361423.9 | 08 16 53.54 | +36 14 23.94 | 4.03 | Pâris et al. (2012) |
| SDSS J081740.52+135134.5 | 08 17 40.53 | +13 51 34.58 | 4.37 | Schneider et al. (2010) |
| SDSS J081748.07+185557.2 | 08 17 48.08 | +18 55 57.27 | 4.26 | Schneider et al. (2007) |
| SDSS J081755.59+312422.6 | 08 17 55.59 | +31 24 22.69 | 4.37 | Pâris et al. (2017) |
| SDSS J081806.87+071920.2 | 08 18 06.88 | +07 19 20.29 | 4.60 | Schneider et al. (2007) |
| SDSS J081813.05+263136.9 | 08 18 13.06 | +26 31 36.93 | 4.18 | Schneider et al. (2005) |
| SDSS J081813.14+072054.9 | 08 18 13.15 | +07 20 54.94 | 4.18 | Schneider et al. (2007) |
| SDSS J081818.51+384446.3 | 08 18 18.52 | +38 44 46.36 | 4.11 | Pâris et al. (2012) |
| SDSS J08184+1722 | 08 18 27.40 | +17 22 52.00 | 6.00 | Fan et al. (2006) |
| SDSS J081850.17+251032.5 | 08 18 50.17 | +25 10 32.56 | 4.08 | Schneider et al. (2007) |
| SDSS J081957.42+223727.0 | 08 19 57.42 | +22 37 27.09 | 4.13 | Pâris et al. (2014) |
| SDSS J082009.09+451559.0 | 08 20 09.10 | +45 15 59.05 | 4.15 | Pâris et al. (2017) |
| SDSS J082021.37+390327.1 | 08 20 21.38 | +39 03 27.20 | 4.30 | Schneider et al. (2005) |
| SDSS J082039.66+372137.3 | 08 20 39.67 | +37 21 37.31 | 4.28 | Schneider et al. (2005) |
| SDSS J082100.46+262032.7 | 08 21 00.47 | +26 20 32.77 | 4.04 | Pâris et al. (2014) |
| SDSS J082120.84+360809.6 | 08 21 20.85 | +36 08 09.66 | 4.70 | Schneider et al. (2005) |
| SDSS J082151.94+103743.0 | 08 21 51.94 | +10 37 43.03 | 4.01 | Schneider et al. (2010) |
| SDSS J082153.30+175628.2 | 08 21 53.31 | +17 56 28.25 | 4.36 | Schneider et al. (2010) |
| SDSS J082155.57+260103.2 | 08 21 55.58 | +26 01 03.30 | 4.64 | Pâris et al. (2017) |
| SDSS J082212.34+160436.9 | 08 22 12.35 | +16 04 36.95 | 4.48 | Pâris et al. (2017) |
| SDSS J082234.47+361534.7 | 08 22 34.47 | +36 15 34.80 | 4.61 | Pâris et al. (2017) |
| SDSS J082340.47+342753.0 | 08 23 40.47 | +34 27 53.04 | 4.24 | Schneider et al. (2005) |
| SDSS J082357.59+135032.2 | 08 23 57.59 | +13 50 32.25 | 4.50 | Schneider et al. (2010) |
| SDSS J082454.01+130216.9 | 08 24 54.02 | +13 02 16.98 | 5.15 | Schneider et al. (2010) |
| SDSS J082500.52+141542.5 | 08 25 00.53 | +14 15 42.52 | 4.38 | Schneider et al. (2010) |
| SDSS J082503.64+393325.5 | 08 25 03.65 | +39 33 25.57 | 4.02 | Pâris et al. (2017) |
| SDSS J082522.99+291516.5 | 08 25 23.00 | +29 15 16.53 | 4.04 | Pâris et al. (2012) |
| SDSS J082721.45+294028.5 | 08 27 21.45 | +29 40 28.51 | 4.03 | Pâris et al. (2012) |
| SDSS J082800.57+245111.8 | 08 28 00.57 | +24 51 11.87 | 4.78 | Pâris et al. (2014) |
| SDSS J082809.15+125600.9 | 08 28 09.16 | +12 56 00.91 | 4.29 | Schneider et al. (2010) |
| ULAS J0828+2633 | 08 28 13.41 | +26 33 55.49 | 6.05 | Warren (in prep.) |
| SDSS J082858.28+330210.9 | 08 28 58.28 | +33 02 10.91 | 4.01 | Pâris et al. (2017) |
| PSO J127.2817+03.0657 | 08 29 07.62 | +03 03 56.52 | 5.85 | Bañados et al. (2016) |
| DELS J082931.97+411740.4 | 08 29 31.97 | +41 17 40.40 | 6.77 | Wang et al. (2018) |
| J082933.10+250645.6 | 08 29 33.10 | +25 06 45.60 | 5.35 | Yang et al. (2017) |
| SDSS J083005.13+074054.2 | 08 30 05.14 | +07 40 54.27 | 4.36 | Schneider et al. (2007) |
| SDSS J083018.00+533630.1 | 08 30 18.00 | +53 36 30.14 | 4.12 | Pâris et al. (2017) |
| SDSS J083046.28+474646.5 | 08 30 46.28 | +47 46 46.52 | 4.32 | Pâris et al. (2017) |
| SDSS J083100.67+434426.9 | 08 31 00.68 | +43 44 26.98 | 4.43 | Pâris et al. (2017) |
| SDSS J083103.01+523533.5 | 08 31 03.01 | +52 35 33.58 | 4.47 | Pâris et al. (2017) |
| SDSS J083122.57+404623.3 | 08 31 22.58 | +40 46 23.40 | 4.82 | Schneider et al. (2005) |
| SDSS J083138.97+393235.3 | 08 31 38.97 | +39 32 35.40 | 4.17 | Schneider et al. (2005) |
| SDSS J083139.12+303809.2 | 08 31 39.12 | +30 38 09.28 | 4.04 | Pâris et al. (2012) |
| SDSS J083201.54+263641.9 | 08 32 01.54 | +26 36 41.92 | 4.56 | Schneider et al. (2007) |

| | | | | |
|---|---|---|---|---|
| SDSS J083209.07+084749.1 | 08 32 09.07 | +08 47 49.14 | 4.37 | Pâris et al. (2017) |
| SDSS J083212.37+530327.3 | 08 32 12.37 | +53 03 27.34 | 4.05 | Pâris et al. (2017) |
| SDSS J083316.18+210007.9 | 08 33 16.19 | +21 00 07.93 | 4.15 | Pâris et al. (2012) |
| SDSS J08332+2726 | 08 33 17.67 | +27 26 29.00 | 5.02 | Chiu et al. (2005) |
| SDSS J083353.25+302318.5 | 08 33 53.26 | +30 23 18.52 | 4.09 | Schneider et al. (2005) |
| J0834+0211 | 08 34 00.88 | +02 11 46.90 | 6.15 | Chehade et al. (2018) |
| SDSS J083429.44+214024.6 | 08 34 29.45 | +21 40 24.65 | 4.51 | Schneider et al. (2007) |
| SDSS J083513.12+193706.1 | 08 35 13.13 | +19 37 06.11 | 4.63 | Schneider et al. (2010) |
| SDSS J083513.15+070729.3 | 08 35 13.15 | +07 07 29.35 | 4.05 | Schneider et al. (2007) |
| SDSS J0835+3217 | 08 35 25.76 | +32 17 52.62 | 5.89 | Jiang et al. (2016) |
| SDSS J083526.19+322747.5 | 08 35 26.19 | +32 27 47.56 | 5.89 | Jiang et al. (2016) |
| SDSS J083548.46+310951.8 | 08 35 48.47 | +31 09 51.86 | 4.32 | Pâris et al. (2012) |
| SDSS J083552.62+163343.9 | 08 35 52.63 | +16 33 43.99 | 4.25 | Schneider et al. (2010) |
| SDSS J083554.36+053753.0 | 08 35 54.36 | +05 37 53.06 | 5.07 | Pâris et al. (2014) |
| SDSS J083616.19+214847.8 | 08 36 16.19 | +21 48 47.84 | 4.60 | Schneider et al. (2007) |
| SDSS J083654.36+312216.9 | 08 36 54.36 | +31 22 17.00 | 4.03 | Pâris et al. (2014) |
| SDSS J083655.80+064104.6 | 08 36 55.81 | +06 41 04.63 | 4.44 | Schneider et al. (2007) |
| SDSS J083706.10+364236.5 | 08 37 06.10 | +36 42 36.55 | 4.02 | Pâris et al. (2012) |
| DELS J083737.84+492900.4 | 08 37 37.84 | +49 29 00.40 | 6.71 | Wang et al. (2018) |
| SDSS J083824.32+460443.7 | 08 38 24.32 | +46 04 43.77 | 4.02 | Schneider et al. (2005) |
| SDSS J083838.97+444735.7 | 08 38 38.98 | +44 47 35.71 | 4.01 | Pâris et al. (2017) |
| SDSS J083839.16+285852.7 | 08 38 39.17 | +28 58 52.72 | 4.37 | Pâris et al. (2017) |
| SDSS J083841.55+390217.1 | 08 38 41.56 | +39 02 17.19 | 4.34 | Schneider et al. (2005) |
| SDSS J083920.54+352459.5 | 08 39 20.54 | +35 24 59.54 | 4.79 | Pâris et al. (2017) |
| SDSS J083941.44+031817.1 | 08 39 41.45 | +03 18 17.14 | 4.23 | Schneider et al. (2005) |
| DELS J083946.88+390011.5 | 08 39 46.88 | +39 00 11.50 | 6.95 | Wang et al. (2018) |
| VIK J0839+0015 | 08 39 55.36 | +00 15 54.21 | 5.84 | Venemans et al. (2015b) |
| SDSS J0840+5624 | 08 40 35.10 | +56 24 20.22 | 5.84 | Fan et al. (2006) |
| SDSS J084045.40+090809.4 | 08 40 45.40 | +09 08 09.48 | 4.53 | Schneider et al. (2007) |
| SDSS J084051.22+404806.7 | 08 40 51.23 | +40 48 06.77 | 4.43 | Schneider et al. (2005) |
| SDSS J084104.98+183307.9 | 08 41 04.98 | +18 33 07.99 | 4.22 | Schneider et al. (2010) |
| SDSS J08413+2905 | 08 41 19.53 | +29 05 05.00 | 5.96 | Goto (2006) |
| SDSS J084121.24+224242.7 | 08 41 21.25 | +22 42 42.70 | 4.54 | Pâris et al. (2017) |
| SDSS J084203.02+433410.0 | 08 42 03.03 | +43 34 10.09 | 4.45 | Schneider et al. (2005) |
| SDSS J084229.23+121848.2 | 08 42 29.23 | +12 18 48.20 | 6.08 | De Rosa et al. (2011) |
| SDSS J084353.54+131953.5 | 08 43 53.55 | +13 19 53.60 | 4.08 | Schneider et al. (2010) |
| J0844−0132 | 08 44 08.61 | −01 32 16.50 | 6.18 | Chehade et al. (2018) |
| J0844−0052 | 08 44 31.60 | −00 52 54.60 | 6.25 | Matsuoka et al. (2018b) |
| SDSS J084438.04+584825.5 | 08 44 38.04 | +58 48 25.51 | 4.66 | Schneider et al. (2010) |
| SDSS J084451.72+051827.7 | 08 44 51.72 | +05 18 27.73 | 4.47 | Schneider et al. (2005) |
| SDSS J084516.23+401928.4 | 08 45 16.23 | +40 19 28.45 | 4.68 | Pâris et al. (2017) |
| SDSS J084520.35+060808.6 | 08 45 20.35 | +06 08 08.62 | 4.19 | Schneider et al. (2005) |
| SDSS J084555.52+220920.4 | 08 45 55.53 | +22 09 20.46 | 4.28 | Schneider et al. (2007) |
| SDSS J084556.42+314528.3 | 08 45 56.42 | +31 45 28.34 | 4.46 | Schneider et al. (2007) |
| SDSS J084627.84+080051.7 | 08 46 27.84 | +08 00 51.72 | 5.00 | Schneider et al. (2007) |
| SDSS J084631.52+241108.3 | 08 46 31.53 | +24 11 08.37 | 4.73 | Schneider et al. (2007) |
| SDSS J084634.23+475910.1 | 08 46 34.24 | +47 59 10.15 | 4.32 | Pâris et al. (2017) |
| SDSS J084718.93+235502.4 | 08 47 18.93 | +23 55 02.41 | 4.01 | Schneider et al. (2007) |
| SDSS J08480+3427 | 08 48 02.80 | +34 27 15.00 | 4.73 | Chiu et al. (2005) |
| SDSS J084811.52−001417.9 | 08 48 11.52 | −00 14 17.96 | 4.12 | Schneider et al. (2005) |
| SDSS J084926.36+182431.6 | 08 49 26.37 | +18 24 31.68 | 4.06 | Pâris et al. (2017) |
| IMS J085024−041850 | 08 50 23.81 | −04 18 49.60 | 4.80 | Kim et al. (2019) |
| SDSS J085031.57+355428.6 | 08 50 31.58 | +35 54 28.66 | 4.05 | Schneider et al. (2005) |
| SDSS J0850+3246 | 08 50 48.25 | +32 46 47.94 | 5.87 | Jiang et al. (2015) |
| SDSS J085143.72+233208.9 | 08 51 43.73 | +23 32 08.97 | 4.48 | Schneider et al. (2007) |
| SDSS J085151.26+020755.9 | 08 51 51.26 | +02 07 55.96 | 4.28 | Pâris et al. (2017) |
| SDSS J085210.88+535948.8 | 08 52 10.88 | +53 59 48.90 | 4.21 | Pâris et al. (2017) |

| | | | | |
|---|---|---|---|---|
| IMS J085225−051413 | 08 52 24.73 | −05 14 13.40 | 4.82 | Kim et al. (2019) |
| PSS J0852+5045 | 08 52 27.28 | +50 45 10.80 | 4.21 | Djorgovski et al. (2001) |
| SDSS J085237.31+055934.9 | 08 52 37.31 | +05 59 34.99 | 4.16 | Pâris et al. (2017) |
| SDSS J085313.22+175502.8 | 08 53 13.23 | +17 55 02.82 | 4.07 | Pâris et al. (2014) |
| IMS J085324−045626 | 08 53 23.68 | −04 56 25.60 | 4.83 | Kim et al. (2019) |
| J0853+0139 | 08 53 48.84 | +01 39 11.00 | 6.01 | Matsuoka et al. (2018b) |
| SDSS J085405.10+171037.9 | 08 54 05.11 | +17 10 37.90 | 4.43 | Pâris et al. (2017) |
| SDSS J085405.43+172028.7 | 08 54 05.44 | +17 20 28.72 | 4.07 | Schneider et al. (2010) |
| SDSS J085430.17+004213.6 | 08 54 30.18 | +00 42 13.66 | 4.08 | Schneider et al. (2005) |
| SDSS J085430.37+205650.8 | 08 54 30.37 | +20 56 50.84 | 5.17 | Schneider et al. (2010) |
| SDSS J085546.23+082051.3 | 08 55 46.24 | +08 20 51.31 | 4.30 | Pâris et al. (2017) |
| SDSS J085606.89+393924.0 | 08 56 06.90 | +39 39 24.06 | 4.14 | Schneider et al. (2005) |
| SDSS J085625.92+092523.6 | 08 56 25.92 | +09 25 23.65 | 4.33 | Schneider et al. (2007) |
| SDSS J085634.92+525206.2 | 08 56 34.93 | +52 52 06.23 | 4.80 | Pâris et al. (2017) |
| SDSS J085637.69+100855.4 | 08 56 37.70 | +10 08 55.46 | 4.54 | Pâris et al. (2017) |
| SDSS J085644.99+391217.1 | 08 56 45.00 | +39 12 17.16 | 4.25 | Pâris et al. (2017) |
| SDSS J085653.19+174400.7 | 08 56 53.19 | +17 44 00.74 | 4.19 | Schneider et al. (2010) |
| SDSS J085653.58+201541.7 | 08 56 53.58 | +20 15 41.78 | 4.09 | Schneider et al. (2010) |
| SDSS J085707.94+321031.9 | 08 57 07.94 | +32 10 31.98 | 4.80 | Schneider et al. (2007) |
| J0857+0056 | 08 57 38.53 | +00 56 12.70 | 6.35 | Matsuoka et al. (2018b) |
| J0858+0000 | 08 58 13.51 | +00 00 57.10 | 5.99 | Chehade et al. (2018) |
| SDSS J085818.89+495509.3 | 08 58 18.90 | +49 55 09.32 | 4.01 | Pâris et al. (2017) |
| HSC J0859+0022 | 08 59 07.19 | +00 22 55.90 | 6.39 | Matsuoka et al. (2016) |
| SDSS J085931.29+252019.5 | 08 59 31.29 | +25 20 19.59 | 4.78 | Schneider et al. (2007) |
| J085942.62+443115.97 | 08 59 42.62 | +44 31 15.97 | 4.57 | Wang et al. (2016) |
| SDSS J090029.54+430053.6 | 09 00 29.54 | +43 00 53.69 | 4.40 | Schneider et al. (2005) |
| SDSS J09009+2745 | 09 00 59.53 | +27 45 58.00 | 4.96 | Chiu et al. (2005) |
| SDSS J090100.61+472536.2 | 09 01 00.61 | +47 25 36.20 | 4.60 | Schneider et al. (2005) |
| SDSS J090106.43+291128.5 | 09 01 06.43 | +29 11 28.58 | 4.01 | Schneider et al. (2007) |
| SDSS J090111.36+453540.0 | 09 01 11.36 | +45 35 40.05 | 4.04 | Schneider et al. (2005) |
| SDSS J090136.19+315508.4 | 09 01 36.19 | +31 55 08.41 | 4.59 | Pâris et al. (2017) |
| SDSS J090158.85+610931.7 | 09 01 58.85 | +61 09 31.70 | 4.09 | Schneider et al. (2010) |
| SDSS J090234.76+432154.4 | 09 02 34.76 | +43 21 54.41 | 4.20 | Schneider et al. (2005) |
| SDSS J090242.07−002125.9 | 09 02 42.08 | −00 21 25.92 | 4.43 | Schneider et al. (2005) |
| SDSS J090245.76+085115.9 | 09 02 45.76 | +08 51 15.92 | 5.22 | Schneider et al. (2007) |
| J0902+0155 | 09 02 54.87 | +01 55 10.90 | 6.01 | Matsuoka et al. (2018b) |
| SDSS J090301.33+180238.5 | 09 03 01.33 | +18 02 38.58 | 4.08 | Pâris et al. (2014) |
| J0903+0211 | 09 03 14.68 | +02 11 28.30 | 5.92 | Matsuoka et al. (2018b) |
| SDSS J090324.68+494345.1 | 09 03 24.68 | +49 43 45.18 | 4.24 | Pâris et al. (2017) |
| SDSS J090329.21+225933.6 | 09 03 29.21 | +22 59 33.62 | 4.31 | Schneider et al. (2010) |
| SDSS J090419.53+321025.8 | 09 04 19.54 | +32 10 25.89 | 4.42 | Pâris et al. (2017) |
| SDSS J090425.10+102932.5 | 09 04 25.10 | +10 29 32.50 | 4.16 | Pâris et al. (2017) |
| SDSS J090425.43+335302.7 | 09 04 25.43 | +33 53 02.72 | 4.04 | Schneider et al. (2007) |
| SDSS J090440.64+535038.8 | 09 04 40.64 | +53 50 38.88 | 4.30 | Schneider et al. (2005) |
| SDSS J090442.50+415906.0 | 09 04 42.51 | +41 59 06.03 | 4.09 | Schneider et al. (2005) |
| SDSS J090529.51+254018.2 | 09 05 29.52 | +25 40 18.23 | 4.29 | Pâris et al. (2017) |
| SDSS J090532.14−001430.4 | 09 05 32.15 | −00 14 30.44 | 4.26 | Schneider et al. (2005) |
| J0905+0300 | 09 05 44.65 | +03 00 58.80 | 6.27 | Matsuoka et al. (2018b) |
| SDSS J090609.81+164500.7 | 09 06 09.82 | +16 45 00.78 | 4.06 | Schneider et al. (2010) |
| SDSS J090632.85+503028.7 | 09 06 32.86 | +50 30 28.72 | 4.73 | Pâris et al. (2017) |
| SDSS J090634.84+023433.8 | 09 06 34.84 | +02 34 33.84 | 4.50 | Schneider et al. (2005) |
| SDSS J090712.28+201417.6 | 09 07 12.28 | +20 14 17.69 | 4.23 | Schneider et al. (2010) |
| SDSS J090820.70+262650.4 | 09 08 20.71 | +26 26 50.49 | 4.34 | Pâris et al. (2017) |
| SDSS J090833.30+283540.0 | 09 08 33.31 | +28 35 40.09 | 4.02 | Pâris et al. (2017) |
| SDSS J090855.35+333637.5 | 09 08 55.35 | +33 36 37.51 | 4.59 | Pâris et al. (2017) |
| SDSS J090911.93+421516.9 | 09 09 11.94 | +42 15 16.97 | 4.74 | Schneider et al. (2005) |
| J0909+0440 | 09 09 21.50 | +04 40 42.90 | 6.15 | Chehade et al. (2018) |

| | | | | |
|---|---|---|---|---|
| SDSS J090925.12+323926.0 | 09 09 25.12 | +32 39 26.06 | 4.53 | Pâris et al. (2017) |
| 2SLAQ J090950.05−011212.4 | 09 09 50.05 | −01 12 12.34 | 4.73 | Croom et al. (2009) |
| DELS J091013.63+165629.8 | 09 10 13.63 | +16 56 29.80 | 6.72 | Wang et al. (2018) |
| SDSS J091030.73+320853.6 | 09 10 30.73 | +32 08 53.68 | 4.08 | Schneider et al. (2007) |
| SDSS J091042.86+355627.1 | 09 10 42.86 | +35 56 27.19 | 4.09 | Schneider et al. (2005) |
| SDSS J091044.99+174431.2 | 09 10 45.00 | +17 44 31.27 | 4.10 | Schneider et al. (2010) |
| SDSS J091049.75+185212.6 | 09 10 49.76 | +18 52 12.63 | 4.06 | Schneider et al. (2010) |
| DELS J091054.53−041406.8 | 09 10 54.53 | −04 14 06.80 | 6.63 | Wang et al. (2018) |
| SDSS J091055.04+202836.9 | 09 10 55.05 | +20 28 36.91 | 4.39 | Schneider et al. (2010) |
| SDSS J091112.25+255425.6 | 09 11 12.26 | +25 54 25.69 | 4.81 | Pâris et al. (2017) |
| J0911+0152 | 09 11 14.27 | +01 52 19.40 | 6.07 | Matsuoka et al. (2018b) |
| SDSS J091132.56+411105.1 | 09 11 32.56 | +41 11 05.13 | 4.25 | Schneider et al. (2005) |
| SDSS J091139.61+231327.6 | 09 11 39.61 | +23 13 27.69 | 4.63 | Pâris et al. (2014) |
| SDSS J091244.76+011624.5 | 09 12 44.76 | +01 16 24.57 | 4.12 | Pâris et al. (2017) |
| SDSS J091406.91+020605.8 | 09 14 06.91 | +02 06 05.85 | 4.26 | Pâris et al. (2012) |
| SDSS J091417.84+325955.2 | 09 14 17.84 | +32 59 55.28 | 4.67 | Schneider et al. (2007) |
| PC 0910+5625 | 09 14 39.33 | +56 13 21.00 | 4.04 | Schmidt, Schneider, & Gunn (1987) |
| SDSS J091445.89+301738.3 | 09 14 45.89 | +30 17 38.30 | 4.28 | Schneider et al. (2007) |
| SDSS J091524.69+243313.3 | 09 15 24.70 | +24 33 13.33 | 4.14 | Pâris et al. (2014) |
| DLS J091527.53+291750.4 | 09 15 27.53 | +29 17 50.40 | 4.34 | Glikman et al. (2010) |
| SDSS J091543.64+492416.6 | 09 15 43.64 | +49 24 16.65 | 5.19 | Pâris et al. (2017) |
| SDSS J091623.32+521730.2 | 09 16 23.32 | +52 17 30.27 | 4.05 | Schneider et al. (2005) |
| SDSS J091635.42+264510.9 | 09 16 35.43 | +26 45 10.90 | 4.03 | Pâris et al. (2017) |
| SDSS J091657.50+281828.1 | 09 16 57.50 | +28 18 28.17 | 4.09 | Schneider et al. (2007) |
| SDSS J091724.82+495438.8 | 09 17 24.83 | +49 54 38.82 | 4.78 | Pâris et al. (2017) |
| SDSS J091729.33+314320.2 | 09 17 29.33 | +31 43 20.22 | 4.35 | Pâris et al. (2017) |
| SDSS J091757.95+383040.1 | 09 17 57.96 | +38 30 40.16 | 5.11 | Pâris et al. (2014) |
| SDSS J091814.00+181459.7 | 09 18 14.00 | +18 14 59.75 | 4.15 | Pâris et al. (2017) |
| J0918+0139 | 09 18 33.17 | +01 39 23.30 | 6.19 | Chehade et al. (2018) |
| 2SLAQ J091859.97−005236.6 | 09 18 59.97 | −00 52 36.56 | 4.55 | Croom et al. (2009) |
| SDSS J091903.19+404344.5 | 09 19 03.19 | +40 43 44.59 | 4.01 | Schneider et al. (2005) |
| SDSS J091922.61+515337.5 | 09 19 22.62 | +51 53 37.51 | 4.01 | Pâris et al. (2017) |
| SDSS J091952.53+052159.0 | 09 19 52.54 | +05 21 59.04 | 4.16 | Schneider et al. (2005) |
| SDSS J092008.27+435300.9 | 09 20 08.27 | +43 53 00.94 | 4.93 | Pâris et al. (2017) |
| SDSS J092038.48+564235.8 | 09 20 38.48 | +56 42 35.86 | 4.17 | Schneider et al. (2005) |
| J0921+0007 | 09 21 20.56 | +00 07 22.90 | 6.56 | Chehade et al. (2018) |
| SDSS J092129.83+094815.8 | 09 21 29.83 | +09 48 15.87 | 4.22 | Schneider et al. (2005) |
| DLS J092151.96+292457.2 | 09 21 51.96 | +29 24 57.20 | 4.32 | Glikman et al. (2010) |
| SDSS J092210.25+045751.9 | 09 22 10.26 | +04 57 52.00 | 4.06 | Pâris et al. (2017) |
| SDSS J092216.81+265359.0 | 09 22 16.81 | +26 53 59.06 | 5.05 | Pâris et al. (2017) |
| SDSS J092222.86+314612.1 | 09 22 22.87 | +31 46 12.19 | 4.08 | Pâris et al. (2017) |
| SDSS J092236.49+173943.0 | 09 22 36.50 | +17 39 43.01 | 4.12 | Pâris et al. (2014) |
| SDSS J092250.37+420908.8 | 09 22 50.37 | +42 09 08.84 | 4.09 | Schneider et al. (2005) |
| SDSS J092255.55+515409.9 | 09 22 55.56 | +51 54 09.94 | 4.09 | Pâris et al. (2017) |
| SDSS J092256.20+561849.3 | 09 22 56.20 | +56 18 49.33 | 4.20 | Pâris et al. (2017) |
| SDSS J092303.52+024739.6 | 09 23 03.53 | +02 47 39.68 | 4.65 | Schneider et al. (2005) |
| SDSS J092336.06+231545.8 | 09 23 36.07 | +23 15 45.86 | 4.07 | Pâris et al. (2014) |
| DLS J092336.82+300949.9 | 09 23 36.78 | +30 09 49.58 | 5.07 | Glikman et al. (2010) |
| J0923+0402 | 09 23 47.12 | +04 02 54.40 | 6.60 | Matsuoka et al. (2018a) |
| SDSS J092358.55+393045.4 | 09 23 58.56 | +39 30 45.41 | 4.04 | Pâris et al. (2014) |
| SDSS J092443.21+252616.7 | 09 24 43.22 | +25 26 16.74 | 4.03 | Pâris et al. (2017) |
| SDSS J092526.75+425736.7 | 09 25 26.76 | +42 57 36.73 | 4.26 | Schneider et al. (2005) |
| SDSS J092548.06+104800.2 | 09 25 48.07 | +10 48 00.23 | 4.08 | Pâris et al. (2017) |
| SDSS J092554.13+194349.8 | 09 25 54.14 | +19 43 49.88 | 4.05 | Pâris et al. (2017) |
| PSS J0926+3055 | 09 26 36.33 | +30 55 05.00 | 4.19 | Djorgovski et al. (2001) |
| SDSS J09273+2001 | 09 27 21.80 | +20 01 24.00 | 5.79 | Fan et al. (2006) |
| SDSS J092819.28+534024.1 | 09 28 19.29 | +53 40 24.15 | 4.44 | Pâris et al. (2017) |

| | | | | |
|---|---|---|---|---|
| SDSS J092925.93+214228.3 | 09 29 25.94 | +21 42 28.36 | 4.14 | Pâris et al. (2014) |
| SDSS J092953.61+160604.0 | 09 29 53.62 | +16 06 04.08 | 4.19 | Schneider et al. (2010) |
| SDSS J093035.94+335717.6 | 09 30 35.94 | +33 57 17.60 | 4.00 | Pâris et al. (2017) |
| SDSS J093223.66−000830.6 | 09 32 23.66 | −00 08 30.61 | 4.13 | Pâris et al. (2012) |
| SDSS J093249.75+122205.8 | 09 32 49.76 | +12 22 05.81 | 5.02 | Pâris et al. (2014) |
| SDSS J093258.65+480429.6 | 09 32 58.66 | +48 04 29.65 | 4.35 | Pâris et al. (2017) |
| SDSS J093306.88+332556.6 | 09 33 06.88 | +33 25 56.64 | 4.59 | Schneider et al. (2007) |
| SDSS J093333.85+051839.9 | 09 33 33.86 | +05 18 39.98 | 4.51 | Schneider et al. (2005) |
| SDSS J093343.58+260915.8 | 09 33 43.59 | +26 09 15.86 | 4.20 | Pâris et al. (2017) |
| SDSS J093412.85+294524.3 | 09 34 12.86 | +29 45 24.37 | 4.72 | Schneider et al. (2007) |
| SDSS J093453.22+465717.6 | 09 34 53.23 | +46 57 17.67 | 4.53 | Pâris et al. (2017) |
| SDSS J093508.50+080114.5 | 09 35 08.50 | +08 01 14.53 | 4.66 | Pâris et al. (2017) |
| SDSS J093509.47+475256.3 | 09 35 09.47 | +47 52 56.34 | 4.01 | Pâris et al. (2017) |
| SDSS J093513.97+464736.1 | 09 35 13.98 | +46 47 36.19 | 4.02 | Pâris et al. (2017) |
| SDSS J093521.38+612339.2 | 09 35 21.39 | +61 23 39.27 | 4.03 | Pâris et al. (2017) |
| J093523.31−020754.4 | 09 35 23.31 | −02 07 54.40 | 5.32 | Yang et al. (2017) |
| SDSS J093523.31+411518.5 | 09 35 23.32 | +41 15 18.57 | 4.81 | Schneider et al. (2005) |
| SDSS J093533.92+173506.1 | 09 35 33.92 | +17 35 06.17 | 4.00 | Schneider et al. (2010) |
| SDSS J093554.46+525616.4 | 09 35 54.46 | +52 56 16.45 | 4.02 | Schneider et al. (2005) |
| SDSS J093621.50+493032.7 | 09 36 21.51 | +49 30 32.78 | 4.22 | Pâris et al. (2017) |
| SDSS J093628.26+083401.6 | 09 36 28.26 | +08 34 01.64 | 4.25 | Pâris et al. (2014) |
| SDSS J093632.62+102011.8 | 09 36 32.63 | +10 20 11.87 | 4.11 | Pâris et al. (2014) |
| SDSS J093651.36+310358.3 | 09 36 51.36 | +31 03 58.30 | 4.65 | Pâris et al. (2017) |
| SDSS J093652.60+401546.2 | 09 36 52.61 | +40 15 46.22 | 4.56 | Schneider et al. (2005) |
| SDSS J093654.09+240336.8 | 09 36 54.09 | +24 03 36.80 | 4.55 | Pâris et al. (2017) |
| SDSS J093740.40+151835.9 | 09 37 40.40 | +15 18 35.95 | 4.12 | Schneider et al. (2010) |
| SDSS J093746.47+114038.3 | 09 37 46.48 | +11 40 38.40 | 4.32 | Schneider et al. (2007) |
| SDSS J093824.81+460006.2 | 09 38 24.82 | +46 00 06.23 | 4.11 | Pâris et al. (2017) |
| SDSS J093917.57+272713.1 | 09 39 17.57 | +27 27 13.19 | 4.40 | Schneider et al. (2007) |
| SDSSp J093931.91+003955.0 | 09 39 31.91 | +00 39 55.00 | 4.49 | Schneider et al. (2001) |
| SDSS J093949.42+335548.3 | 09 39 49.42 | +33 55 48.38 | 4.12 | Pâris et al. (2017) |
| SDSS J093953.54+290602.6 | 09 39 53.54 | +29 06 02.67 | 4.26 | Schneider et al. (2007) |
| SDSS J094036.88+064417.9 | 09 40 36.89 | +06 44 17.93 | 4.02 | Pâris et al. (2014) |
| SDSS J094056.01+584830.1 | 09 40 56.02 | +58 48 30.19 | 4.68 | Pâris et al. (2017) |
| SDSS J094108.35+594725.7 | 09 41 08.36 | +59 47 25.75 | 4.86 | Pâris et al. (2017) |
| PS1 J094146.16−011748.03 | 09 41 46.16 | −01 17 48.03 | 4.95 | Yang et al. (2018) |
| SDSS J094225.03+272411.1 | 09 42 25.03 | +27 24 11.19 | 4.01 | Pâris et al. (2017) |
| SDSS J094256.17+203629.4 | 09 42 56.17 | +20 36 29.43 | 4.05 | Schneider et al. (2010) |
| SDSS J094326.47+254402.1 | 09 43 26.48 | +25 44 02.14 | 4.32 | Schneider et al. (2010) |
| SDSS J094349.65+095400.9 | 09 43 49.65 | +09 54 00.96 | 4.17 | Schneider et al. (2005) |
| SDSS J094358.38+052422.6 | 09 43 58.38 | +05 24 22.63 | 4.59 | Pâris et al. (2017) |
| SDSS J094408.29+315703.6 | 09 44 08.30 | +31 57 03.66 | 4.61 | Pâris et al. (2017) |
| SDSS J094408.82+434427.0 | 09 44 08.82 | +43 44 27.05 | 4.56 | Pâris et al. (2017) |
| SDSS J094409.52+100656.6 | 09 44 09.52 | +10 06 56.69 | 4.77 | Schneider et al. (2005) |
| SDSS J094417.69+450800.0 | 09 44 17.70 | +45 08 00.05 | 4.82 | Schneider et al. (2005) |
| SDSS J094456.28+053117.8 | 09 44 56.29 | +05 31 17.87 | 4.04 | Pâris et al. (2012) |
| SDSS J094552.12+462411.5 | 09 45 52.12 | +46 24 11.58 | 4.03 | Pâris et al. (2014) |
| SDSS J094604.79+183539.7 | 09 46 04.79 | +18 35 39.71 | 4.80 | Schneider et al. (2010) |
| SDSS J094704.48−001821.0 | 09 47 04.49 | −00 18 21.09 | 4.04 | Pâris et al. (2012) |
| SDSS J094706.93+255638.0 | 09 47 06.94 | +25 56 38.08 | 4.05 | Pâris et al. (2017) |
| SDSS J094712.40+011928.5 | 09 47 12.40 | +01 19 28.52 | 4.28 | Pâris et al. (2012) |
| SDSS J094743.63+165051.1 | 09 47 43.63 | +16 50 51.11 | 4.03 | Pâris et al. (2014) |
| BR 0945−0411 | 09 47 49.60 | −04 25 15.00 | 4.15 | Kennefick, Djorgovski, & Meylan (1996) |
| SDSS J094758.92+512325.9 | 09 47 58.93 | +51 23 25.93 | 4.04 | Pâris et al. (2017) |
| SDSS J094839.41+325603.8 | 09 48 39.41 | +32 56 03.87 | 4.20 | Pâris et al. (2017) |
| SDSS J094855.36+210631.5 | 09 48 55.36 | +21 06 31.57 | 5.17 | Pâris et al. (2017) |
| SDSS J094859.98+493220.1 | 09 48 59.99 | +49 32 20.14 | 4.61 | Pâris et al. (2017) |

| | | | | |
|---|---|---|---|---|
| SDSS J094917.16+602104.4 | 09 49 17.17 | +60 21 04.50 | 4.29 | Pâris et al. (2017) |
| SDSS J094932.26+033531.7 | 09 49 32.27 | +03 35 31.79 | 4.11 | Pâris et al. (2017) |
| SDSS J095000.16+620318.5 | 09 50 00.17 | +62 03 18.59 | 4.07 | Pâris et al. (2017) |
| SDSS J095014.73+233118.9 | 09 50 14.73 | +23 31 18.96 | 4.23 | Pâris et al. (2017) |
| SDSS J095015.44+521812.5 | 09 50 15.45 | +52 18 12.58 | 4.10 | Pâris et al. (2017) |
| SDSS J095018.29+301347.7 | 09 50 18.29 | +30 13 47.71 | 4.43 | Pâris et al. (2017) |
| SDSS J095028.08+110035.2 | 09 50 28.09 | +11 00 35.28 | 4.95 | Pâris et al. (2014) |
| SDSS J095040.70+374930.7 | 09 50 40.70 | +37 49 30.76 | 4.37 | Pâris et al. (2017) |
| SDSS J095129.48+251433.6 | 09 51 29.49 | +25 14 33.66 | 4.07 | Schneider et al. (2010) |
| SDSS J095133.97+191024.7 | 09 51 33.97 | +19 10 24.74 | 4.51 | Schneider et al. (2010) |
| SDSS J095146.71+125715.6 | 09 51 46.71 | +12 57 15.69 | 4.19 | Pâris et al. (2014) |
| SDSS J095151.18+594556.1 | 09 51 51.19 | +59 45 56.16 | 4.87 | Pâris et al. (2017) |
| SDSS J095158.83+391834.3 | 09 51 58.83 | +39 18 34.37 | 4.25 | Schneider et al. (2005) |
| SDSS J095220.80+552829.2 | 09 52 20.81 | +55 28 29.21 | 4.20 | Pâris et al. (2017) |
| SDSS J095307.61+524953.8 | 09 53 07.61 | +52 49 53.81 | 4.28 | Pâris et al. (2017) |
| SDSS J095314.79+632652.6 | 09 53 14.79 | +63 26 52.60 | 4.07 | Pâris et al. (2017) |
| SDSS J095336.63+383709.5 | 09 53 36.63 | +38 37 09.57 | 4.06 | Pâris et al. (2017) |
| BR 0951−0450 | 09 53 55.80 | −05 04 19.00 | 4.37 | Kennefick, Djorgovski, & Meylan (1996) |
| SDSS J095358.65+275907.4 | 09 53 58.65 | +27 59 07.42 | 4.13 | Schneider et al. (2010) |
| SDSS J095405.23+050514.1 | 09 54 05.23 | +05 05 14.12 | 4.08 | Schneider et al. (2005) |
| BRI 0952−0115 | 09 55 00.07 | −01 30 07.00 | 4.43 | Storrie-Lombardi et al. (1996) |
| PSS J0955+5940 | 09 55 11.33 | +59 40 30.68 | 4.36 | Djorgovski et al. (2001) |
| SDSS J095612.59+202320.3 | 09 56 12.60 | +20 23 20.38 | 4.05 | Schneider et al. (2010) |
| PC 0953+4749 | 09 56 25.16 | +47 34 42.52 | 4.49 | Schneider, Schmidt, & Gunn (1994b) |
| SDSS J095632.03+321612.6 | 09 56 32.04 | +32 16 12.66 | 4.61 | Schneider et al. (2007) |
| SDSS J095653.08+375613.7 | 09 56 53.09 | +37 56 13.76 | 4.27 | Pâris et al. (2012) |
| SDSS J095707.67+061059.5 | 09 57 07.68 | +06 10 59.54 | 5.14 | Schneider et al. (2005) |
| J095712.20+101618.5 | 09 57 12.20 | +10 16 18.50 | 5.14 | Yang et al. (2017) |
| SDSS J095723.14+231849.4 | 09 57 23.14 | +23 18 49.41 | 4.02 | Schneider et al. (2010) |
| SDSS J095727.86+051905.2 | 09 57 27.87 | +05 19 05.28 | 5.19 | Pâris et al. (2012) |
| J0957+0053 | 09 57 40.39 | +00 53 33.60 | 6.05 | Chehade et al. (2018) |
| PSS J0957+3308 | 09 57 44.47 | +33 08 20.76 | 4.18 | Djorgovski et al. (2001) |
| COSM J09578+0151 | 09 57 52.00 | +01 51 20.00 | 4.17 | Trump et al. (2009) |
| SDSS J095807.03+171259.0 | 09 58 07.03 | +17 12 59.10 | 4.08 | Schneider et al. (2010) |
| SDSS J095814.02+352448.8 | 09 58 14.03 | +35 24 48.83 | 5.12 | Pâris et al. (2017) |
| SDSS J095817.74+245515.3 | 09 58 17.75 | +24 55 15.37 | 4.18 | Schneider et al. (2010) |
| SDSS J095818.19+224957.5 | 09 58 18.19 | +22 49 57.52 | 4.30 | Schneider et al. (2010) |
| COSM J09589+0210 | 09 58 56.73 | +02 10 47.00 | 4.25 | Trump et al. (2009) |
| SDSS J0959+1032A | 09 59 03.83 | +10 32 45.26 | 4.02 | Hennawi et al. (2010) |
| SDSS J095905.12+103325.0 | 09 59 05.13 | +10 33 25.02 | 4.03 | Schneider et al. (2007) |
| COSM J09591+0226 | 09 59 06.53 | +02 26 39.00 | 4.17 | Trump et al. (2009) |
| COSM J095908.1+022707 | 09 59 08.11 | +02 27 07.69 | 5.07 | Masters et al. (2012) |
| SDSS J095920.22+050008.7 | 09 59 20.22 | +05 00 08.73 | 4.20 | Pâris et al. (2012) |
| SDSS J095937.11+131215.5 | 09 59 37.11 | +13 12 15.52 | 4.06 | Schneider et al. (2007) |
| COSM J100024.2+022509 | 10 00 24.24 | +02 25 09.97 | 4.66 | Masters et al. (2012) |
| COSM J100025.8+014533 | 10 00 25.77 | +01 45 33.12 | 4.14 | Masters et al. (2012) |
| SDSS J100026.44+274125.6 | 10 00 26.44 | +27 41 25.64 | 4.33 | Schneider et al. (2010) |
| SDSS J100043.77+210326.6 | 10 00 43.78 | +21 03 26.67 | 5.07 | Schneider et al. (2010) |
| COSM J100051.6+023457 | 10 00 51.59 | +02 34 57.63 | 5.30 | Masters et al. (2012) |
| COSM J100106.4+015306 | 10 01 06.46 | +01 53 06.34 | 4.72 | Masters et al. (2012) |
| COSM J100154.1+024754 | 10 01 54.16 | +02 47 54.10 | 4.12 | Masters et al. (2012) |
| SDSS J100154.87+630817.9 | 10 01 54.87 | +63 08 17.93 | 4.15 | Pâris et al. (2017) |
| COSM J100156.5+015218 | 10 01 56.55 | +01 52 18.94 | 4.45 | Masters et al. (2012) |
| SDSS J100159.83+593724.3 | 10 01 59.84 | +59 37 24.37 | 4.02 | Pâris et al. (2017) |
| SDSS J100236.37+095048.3 | 10 02 36.37 | +09 50 48.31 | 4.13 | Pâris et al. (2017) |
| SDSS J100251.20+223135.1 | 10 02 51.20 | +22 31 35.11 | 4.75 | Schneider et al. (2010) |
| ID 38736 | 10 02 55.80 | +01 30 58.00 | 4.18 | Boutsia et al. (2018) |

| | | | | |
|---|---|---|---|---|
| SDSS J100320.90+022930.0 | 10 03 20.90 | +02 29 30.08 | 4.41 | Pâris et al. (2012) |
| J1004+0239 | 10 04 01.36 | +02 39 30.70 | 6.41 | Chehade et al. (2018) |
| SDSS J100413.14+630437.3 | 10 04 13.14 | +63 04 37.31 | 4.13 | Pâris et al. (2017) |
| SDSS J100416.12+434739.1 | 10 04 16.13 | +43 47 39.12 | 4.84 | Schneider et al. (2005) |
| SDSS J100444.30+202520.0 | 10 04 44.31 | +20 25 20.05 | 4.99 | Schneider et al. (2010) |
| SDSS J100449.58+404554.0 | 10 04 49.59 | +40 45 54.01 | 4.87 | Schneider et al. (2007) |
| SDSS J100515.29+195343.9 | 10 05 15.30 | +19 53 43.95 | 4.39 | Pâris et al. (2014) |
| SDSS J100528.95+142235.9 | 10 05 28.95 | +14 22 35.93 | 4.07 | Pâris et al. (2014) |
| SDSS J100544.33−011247.4 | 10 05 44.34 | −01 12 47.45 | 4.39 | Pâris et al. (2012) |
| SDSS J100550.37+252304.0 | 10 05 50.37 | +25 23 04.07 | 4.02 | Schneider et al. (2010) |
| SDSS J100602.66+382523.0 | 10 06 02.66 | +38 25 23.09 | 4.43 | Schneider et al. (2007) |
| J100614.61−031030.4 | 10 06 14.61 | −03 10 30.40 | 5.55 | Yang et al. (2017) |
| SDSS J100624.21+002256.3 | 10 06 24.22 | +00 22 56.36 | 4.38 | Pâris et al. (2017) |
| SDSS J100626.67+050613.0 | 10 06 26.68 | +05 06 13.02 | 4.12 | Schneider et al. (2005) |
| SDSS J100647.27+133235.9 | 10 06 47.27 | +13 32 36.00 | 4.33 | Pâris et al. (2014) |
| SDSS J100720.21+385858.2 | 10 07 20.22 | +38 58 58.21 | 4.06 | Pâris et al. (2012) |
| SDSS J100743.71+601329.4 | 10 07 43.71 | +60 13 29.44 | 4.01 | Pâris et al. (2017) |
| SDSS J100746.97+190846.3 | 10 07 46.98 | +19 08 46.37 | 4.26 | Pâris et al. (2017) |
| SDSS J100750.95+424118.1 | 10 07 50.95 | +42 41 18.18 | 4.19 | Pâris et al. (2012) |
| SDSS J100757.18+061836.1 | 10 07 57.19 | +06 18 36.14 | 4.23 | Schneider et al. (2005) |
| SDSS J100805.56+164929.8 | 10 08 05.56 | +16 49 29.86 | 4.20 | Schneider et al. (2010) |
| SDSS J100812.88+342956.3 | 10 08 12.89 | +34 29 56.34 | 4.36 | Schneider et al. (2007) |
| SDSS J100903.37+174950.3 | 10 09 03.37 | +17 49 50.40 | 4.05 | Pâris et al. (2017) |
| SDSS J101006.54+073129.7 | 10 10 06.55 | +07 31 29.73 | 4.53 | Schneider et al. (2005) |
| SDSS J101014.23+413701.6 | 10 10 14.24 | +41 37 01.65 | 4.07 | Pâris et al. (2017) |
| SDSS J101049.63+132746.8 | 10 10 49.64 | +13 27 46.81 | 4.15 | Schneider et al. (2007) |
| SDSS J101052.99+531144.7 | 10 10 52.99 | +53 11 44.71 | 4.53 | Pâris et al. (2017) |
| SDSS J101125.00−021950.1 | 10 11 25.00 | −02 19 50.16 | 4.24 | Pâris et al. (2012) |
| SDSS J101252.85+172823.3 | 10 12 52.86 | +17 28 23.34 | 4.26 | Schneider et al. (2010) |
| SDSS J101253.72+284530.4 | 10 12 53.72 | +28 45 30.46 | 4.55 | Schneider et al. (2010) |
| SDSS J101328.46+381501.2 | 10 13 28.47 | +38 15 01.22 | 4.09 | Pâris et al. (2012) |
| SDSS J101336.33+424026.4 | 10 13 36.33 | +42 40 26.40 | 5.03 | Pâris et al. (2017) |
| SDSS J101341.52+274541.6 | 10 13 41.53 | +27 45 41.66 | 4.04 | Schneider et al. (2010) |
| SDSS J101343.10+133150.3 | 10 13 43.11 | +13 31 50.34 | 4.11 | Schneider et al. (2007) |
| SDSS J101413.72+115203.5 | 10 14 13.72 | +11 52 03.58 | 4.35 | Pâris et al. (2014) |
| SDSS J101417.64+133415.4 | 10 14 17.64 | +13 34 15.49 | 4.56 | Schneider et al. (2007) |
| SDSS J101429.71+610354.9 | 10 14 29.71 | +61 03 54.94 | 4.18 | Pâris et al. (2017) |
| SDSS J101439.51+413830.6 | 10 14 39.52 | +41 38 30.60 | 4.36 | Pâris et al. (2012) |
| SDSS J101440.95+283847.7 | 10 14 40.95 | +28 38 47.71 | 4.56 | Schneider et al. (2010) |
| BRI 1013+0035 | 10 15 49.01 | +00 20 20.01 | 4.40 | Smith, Thompson, & Djorgovski (1994a) |
| SDSS J101635.60+375500.5 | 10 16 35.61 | +37 55 00.56 | 4.29 | Schneider et al. (2007) |
| SDSS J101650.55+130043.0 | 10 16 50.56 | +13 00 43.05 | 4.86 | Schneider et al. (2007) |
| SDSS J101706.01+184013.9 | 10 17 06.02 | +18 40 14.00 | 4.47 | Schneider et al. (2010) |
| SDSS J101708.06+332744.8 | 10 17 08.06 | +33 27 44.82 | 4.04 | Pâris et al. (2017) |
| SDSS J101719.39+040004.1 | 10 17 19.40 | +04 00 04.17 | 4.09 | Schneider et al. (2005) |
| SDSS J101759.63+032739.9 | 10 17 59.63 | +03 27 39.93 | 4.92 | Schneider et al. (2005) |
| SDSS J101813.63+320302.1 | 10 18 13.63 | +32 03 02.20 | 4.00 | Pâris et al. (2017) |
| SDSS J101840.46+285000.7 | 10 18 40.46 | +28 50 00.70 | 4.78 | Schneider et al. (2010) |
| SDSS J101844.41+452504.7 | 10 18 44.42 | +45 25 04.75 | 4.44 | Schneider et al. (2005) |
| SDSS J101852.02+112308.0 | 10 18 52.02 | +11 23 08.07 | 4.13 | Schneider et al. (2007) |
| SDSS J101853.91+443213.5 | 10 18 53.92 | +44 32 13.59 | 4.33 | Pâris et al. (2012) |
| SDSS J101931.71+345917.5 | 10 19 31.71 | +34 59 17.55 | 4.53 | Schneider et al. (2007) |
| SDSS J102016.61+011402.2 | 10 20 16.61 | +01 14 02.22 | 4.23 | Pâris et al. (2012) |
| SDSS J10213−0309 | 10 21 19.13 | −03 09 38.00 | 4.70 | Zheng et al. (2000) |
| SDSS J102140.44+165712.2 | 10 21 40.45 | +16 57 12.28 | 4.01 | Schneider et al. (2010) |
| SDSS J102155.52+533525.9 | 10 21 55.52 | +53 35 25.91 | 4.38 | Pâris et al. (2017) |
| J102201.91+080122.2 | 10 22 01.91 | +08 01 22.20 | 5.30 | Yang et al. (2017) |

| | | | | |
|---|---|---|---|---|
| SDSS J102210.04+225225.4 | 10 22 10.05 | +22 52 25.45 | 5.47 | Schneider et al. (2010) |
| SDSS J102231.91+021420.4 | 10 22 31.91 | +02 14 20.41 | 4.07 | Schneider et al. (2005) |
| SDSS J102234.54+200344.5 | 10 22 34.54 | +20 03 44.59 | 4.15 | Schneider et al. (2010) |
| SDSS J102332.06+633508.2 | 10 23 32.06 | +63 35 08.23 | 4.88 | Pâris et al. (2017) |
| SDSS J102346.94+470856.2 | 10 23 46.95 | +47 08 56.23 | 4.70 | Schneider et al. (2005) |
| SDSS J102408.14+490307.5 | 10 24 08.15 | +49 03 07.60 | 4.01 | Schneider et al. (2005) |
| SDSS J102418.99+210135.6 | 10 24 19.00 | +21 01 35.66 | 4.20 | Pâris et al. (2014) |
| SDSS J102530.36+170852.9 | 10 25 30.36 | +17 08 52.99 | 4.07 | Pâris et al. (2017) |
| SDSS J102622.87+471907.1 | 10 26 22.88 | +47 19 07.19 | 4.93 | Pâris et al. (2017) |
| PSS J1026+3828 | 10 26 56.60 | +38 28 43.86 | 4.19 | Djorgovski et al. (2001) |
| SDSS J102815.76+223924.1 | 10 28 15.76 | +22 39 24.20 | 4.40 | Schneider et al. (2010) |
| SDSS J102824.85+190428.8 | 10 28 24.86 | +19 04 28.87 | 4.08 | Pâris et al. (2014) |
| SDSS J102833.45+074618.9 | 10 28 33.46 | +07 46 18.96 | 5.15 | Pâris et al. (2012) |
| SDSS J102925.45+184627.7 | 10 29 25.46 | +18 46 27.76 | 4.08 | Schneider et al. (2010) |
| SDSS J102932.07+165354.7 | 10 29 32.07 | +16 53 54.76 | 4.51 | Schneider et al. (2010) |
| SDSS J102941.55+173413.5 | 10 29 41.55 | +17 34 13.59 | 4.05 | Schneider et al. (2010) |
| SDSS J103014.06−012343.4 | 10 30 14.07 | −01 23 43.46 | 4.01 | Pâris et al. (2012) |
| SDSS J103026.79+212301.2 | 10 30 26.79 | +21 23 01.21 | 4.33 | Schneider et al. (2010) |
| SDSS J10304+0524 | 10 30 27.13 | +05 24 55.00 | 6.31 | Fan et al. (2001a) |
| PSO J157.9070−02.6599 | 10 31 37.69 | −02 39 35.67 | 5.88 | Bañados et al. (2016) |
| SDSS J103208.57+144029.0 | 10 32 08.57 | +14 40 29.01 | 4.90 | Pâris et al. (2014) |
| SDSS J103215.30+334132.2 | 10 32 15.31 | +33 41 32.21 | 4.17 | Schneider et al. (2007) |
| CLASX J10335+5733 | 10 33 34.00 | +57 33 35.00 | 4.21 | Trouille et al. (2008) |
| SDSS J103335.55+123342.0 | 10 33 35.56 | +12 33 42.06 | 4.46 | Schneider et al. (2007) |
| SDSS J103356.20+355745.1 | 10 33 56.21 | +35 57 45.14 | 4.03 | Schneider et al. (2007) |
| CLASXS 346 | 10 34 14.40 | +57 22 26.00 | 5.40 | Steffen et al. (2004) |
| SDSS J103428.86+393343.4 | 10 34 28.87 | +39 33 43.44 | 4.33 | Pâris et al. (2012) |
| SDSS J103432.72−002702.5 | 10 34 32.72 | −00 27 02.56 | 4.37 | Pâris et al. (2017) |
| SDSS J103446.54+110214.4 | 10 34 46.54 | +11 02 14.47 | 4.29 | Schneider et al. (2007) |
| SDSS J103454.57+100015.4 | 10 34 54.57 | +10 00 15.44 | 4.38 | Pâris et al. (2014) |
| SDSS J103528.78+160212.6 | 10 35 28.78 | +16 02 12.67 | 4.14 | Pâris et al. (2017) |
| SDSS J103557.74+005149.4 | 10 35 57.75 | +00 51 49.49 | 4.15 | Pâris et al. (2012) |
| SDSS J103600.66+270000.1 | 10 36 00.66 | +27 00 00.15 | 4.34 | Pâris et al. (2017) |
| SDSS J103612.76+345113.9 | 10 36 12.76 | +34 51 13.92 | 4.09 | Pâris et al. (2012) |
| BR 1033−0327 | 10 36 23.73 | −03 43 19.00 | 4.51 | Rabbette et al. (1998) |
| PSO J159.2257−02.5438 | 10 36 54.19 | −02 32 37.94 | 6.38 | Bañados et al. (2016) |
| SDSS J103702.51+451748.8 | 10 37 02.52 | +45 17 48.87 | 4.09 | Schneider et al. (2007) |
| SDSS J103711.05+313433.5 | 10 37 11.05 | +31 34 33.51 | 4.91 | Pâris et al. (2017) |
| SDSS J103732.38+070426.2 | 10 37 32.39 | +07 04 26.25 | 4.13 | Schneider et al. (2005) |
| SDSS J103750.57+590132.4 | 10 37 50.57 | +59 01 32.44 | 4.40 | Pâris et al. (2017) |
| SDSS J103843.93+612114.8 | 10 38 43.93 | +61 21 14.82 | 4.09 | Pâris et al. (2017) |
| SDSS J103856.41+245757.0 | 10 38 56.42 | +24 57 57.07 | 4.03 | Schneider et al. (2010) |
| SDSS J103900.09+285442.3 | 10 39 00.09 | +28 54 42.36 | 4.14 | Schneider et al. (2007) |
| PSS J1039+3445 | 10 39 19.28 | +34 45 04.50 | 4.41 | Schneider et al. (2007) |
| SDSS J103941.50+341319.6 | 10 39 41.51 | +34 13 19.70 | 4.20 | Schneider et al. (2007) |
| SDSS J103945.22+220131.6 | 10 39 45.22 | +22 01 31.70 | 4.61 | Schneider et al. (2010) |
| SDSS J103945.90+084834.6 | 10 39 45.90 | +08 48 34.69 | 4.34 | Schneider et al. (2005) |
| SDSS J104021.67+313146.2 | 10 40 21.67 | +31 31 46.29 | 4.10 | Pâris et al. (2017) |
| SDSS J104040.13−001540.8 | 10 40 40.14 | −00 15 40.88 | 4.33 | Schneider et al. (2005) |
| SDSS J104041.09+162233.8 | 10 40 41.10 | +16 22 33.87 | 4.80 | Schneider et al. (2010) |
| SDSS J104056.01+453209.1 | 10 40 56.01 | +45 32 09.10 | 4.23 | Schneider et al. (2007) |
| SDSS J104057.68+514505.8 | 10 40 57.69 | +51 45 05.83 | 4.05 | Schneider et al. (2005) |
| SDSS J104120.82+272308.2 | 10 41 20.82 | +27 23 08.29 | 4.85 | Schneider et al. (2010) |
| SDSS J104121.11+334901.6 | 10 41 21.11 | +33 49 01.63 | 4.12 | Pâris et al. (2017) |
| SDSS J104128.65+592214.1 | 10 41 28.65 | +59 22 14.13 | 4.02 | Pâris et al. (2017) |
| SDSS J104134.96+241728.8 | 10 41 34.97 | +24 17 28.87 | 4.67 | Schneider et al. (2010) |
| SDSS J104214.52+075321.3 | 10 42 14.53 | +07 53 21.38 | 4.13 | Pâris et al. (2014) |

| | | | | |
|---|---|---|---|---|
| SDSS J104229.22+400947.9 | 10 42 29.23 | +40 09 47.97 | 4.26 | Schneider et al. (2007) |
| SDSS J104236.51+555152.0 | 10 42 36.51 | +55 51 52.03 | 4.10 | Pâris et al. (2017) |
| SDSS J104242.40+310713.1 | 10 42 42.41 | +31 07 13.20 | 4.70 | Schneider et al. (2007) |
| SDSS J104248.01+404652.4 | 10 42 48.01 | +40 46 52.42 | 4.05 | Schneider et al. (2007) |
| SDSS J104325.55+404849.4 | 10 43 25.56 | +40 48 49.49 | 4.91 | Pâris et al. (2017) |
| SDSS J104335.19+101034.5 | 10 43 35.19 | +10 10 34.58 | 5.09 | Pâris et al. (2014) |
| SDSS J104400.34+112722.9 | 10 44 00.35 | +11 27 22.92 | 4.07 | Schneider et al. (2007) |
| SDSS J104406.35+182043.8 | 10 44 06.35 | +18 20 43.85 | 4.80 | Pâris et al. (2017) |
| SDSS J104420.10+393643.9 | 10 44 20.11 | +39 36 43.92 | 4.33 | Schneider et al. (2007) |
| SDSS J10445−0125 | 10 44 33.13 | −01 25 02.00 | 5.75 | Fan et al. (2000b) |
| SDSS J104448.78+423509.3 | 10 44 48.79 | +42 35 09.36 | 4.17 | Schneider et al. (2007) |
| SDSS J104504.28+204853.1 | 10 45 04.28 | +20 48 53.12 | 4.39 | Schneider et al. (2010) |
| SDSS J104632.15+404727.6 | 10 46 32.16 | +40 47 27.61 | 4.14 | Pâris et al. (2017) |
| SDSS J104635.24+095539.6 | 10 46 35.24 | +09 55 39.61 | 4.35 | Schneider et al. (2007) |
| SDSS J104636.12+250703.5 | 10 46 36.13 | +25 07 03.58 | 4.02 | Schneider et al. (2010) |
| CLANS J10467+5912 | 10 46 46.60 | +59 12 43.00 | 4.74 | Trouille et al. (2008) |
| SDSS J104650.29+295206.7 | 10 46 50.29 | +29 52 06.80 | 4.30 | Pâris et al. (2017) |
| SDSS J104657.07+165007.2 | 10 46 57.08 | +16 50 07.25 | 4.07 | Schneider et al. (2010) |
| CLANS J10475+5902 | 10 47 33.93 | +59 02 31.00 | 4.50 | Trouille et al. (2008) |
| SDSS J104757.70+325023.5 | 10 47 57.70 | +32 50 23.51 | 4.11 | Schneider et al. (2010) |
| SDSS J104801.31+072952.8 | 10 48 01.32 | +07 29 52.87 | 4.07 | Schneider et al. (2005) |
| SDSS J104814.89−010259.6 | 10 48 14.89 | −01 02 59.61 | 4.31 | Pâris et al. (2017) |
| SDSS J104837.40−002813.6 | 10 48 37.40 | −00 28 13.65 | 4.03 | Schneider et al. (2005) |
| SDSS J10487+4637 | 10 48 45.07 | +46 37 18.00 | 6.23 | Fan et al. (2003) |
| PSS J1048+4407 | 10 48 46.63 | +44 07 10.79 | 4.35 | Kennefick, Djorgovski, & de Carvalho (1995b) |
| SDSS J105005.11+462735.5 | 10 50 05.12 | +46 27 35.51 | 4.84 | Pâris et al. (2017) |
| SDSS J105009.10+192736.8 | 10 50 09.10 | +19 27 36.84 | 4.19 | Pâris et al. (2017) |
| SDSS J105020.40+262002.3 | 10 50 20.41 | +26 20 02.33 | 4.86 | Schneider et al. (2010) |
| SDSS J105036.45+580424.9 | 10 50 36.45 | +58 04 24.95 | 5.16 | Pâris et al. (2017) |
| SDSS J105049.19+212333.9 | 10 50 49.20 | +21 23 33.94 | 4.21 | Pâris et al. (2017) |
| SDSS J105049.27+441144.7 | 10 50 49.28 | +44 11 44.78 | 4.31 | Pâris et al. (2017) |
| SDSS J105122.46+310749.3 | 10 51 22.47 | +31 07 49.31 | 4.26 | Schneider et al. (2010) |
| SDSS J105123.03+354534.3 | 10 51 23.04 | +35 45 34.31 | 4.91 | Schneider et al. (2007) |
| SDSS J105132.34+283406.5 | 10 51 32.34 | +28 34 06.54 | 4.18 | Schneider et al. (2010) |
| SDSS J105141.60+105825.3 | 10 51 41.61 | +10 58 25.37 | 4.18 | Pâris et al. (2014) |
| SDSS J105151.27−003826.3 | 10 51 51.27 | −00 38 26.35 | 4.03 | Pâris et al. (2012) |
| SDSS J105210.79+062008.7 | 10 52 10.80 | +06 20 08.71 | 4.58 | Pâris et al. (2017) |
| RX J10524+5719 | 10 52 25.93 | +57 19 06.00 | 4.45 | Schneider et al. (1998) |
| SDSS J105237.44+164108.9 | 10 52 37.45 | +16 41 08.91 | 4.80 | Schneider et al. (2010) |
| SDSS J105254.59−000625.7 | 10 52 54.60 | −00 06 25.80 | 4.17 | Pâris et al. (2017) |
| SDSS J105254.92+172414.7 | 10 52 54.92 | +17 24 14.79 | 4.21 | Pâris et al. (2017) |
| SDSS J105255.46+383650.1 | 10 52 55.46 | +38 36 50.17 | 4.49 | Schneider et al. (2007) |
| SDSS J105322.96+580412.4 | 10 53 22.97 | +58 04 12.48 | 5.27 | Pâris et al. (2017) |
| DLS J1053−0528 | 10 53 46.00 | −05 28 59.00 | 4.02 | Glikman et al. (2007) |
| DLS J105348.89−053319.4 | 10 53 48.89 | −05 33 19.40 | 4.20 | Glikman et al. (2010) |
| SDSS J105353.52+221813.5 | 10 53 53.52 | +22 18 13.55 | 4.06 | Schneider et al. (2010) |
| SDSS J105402.17+292902.6 | 10 54 02.17 | +29 29 02.66 | 4.81 | Pâris et al. (2017) |
| SDSS J105412.25+175459.4 | 10 54 12.26 | +17 54 59.42 | 4.15 | Schneider et al. (2010) |
| SDSS J105443.63+102218.6 | 10 54 43.64 | +10 22 18.64 | 4.26 | Pâris et al. (2017) |
| SDSS J105445.43+163337.3 | 10 54 45.43 | +16 33 37.39 | 5.14 | Schneider et al. (2010) |
| SDSS J105447.04+365936.5 | 10 54 47.04 | +36 59 36.53 | 4.29 | Pâris et al. (2012) |
| SDSS J105457.52+351421.8 | 10 54 57.53 | +35 14 21.87 | 4.07 | Schneider et al. (2007) |
| SDSS J105502.95+402435.3 | 10 55 02.96 | +40 24 35.37 | 4.85 | Schneider et al. (2007) |
| DLS J105507.12−053014.9 | 10 55 07.12 | −05 30 14.90 | 4.40 | Glikman et al. (2010) |
| DLS J105523.03−054850.7 | 10 55 23.03 | −05 48 50.70 | 4.12 | Glikman et al. (2010) |
| SDSS J105553.24+095404.7 | 10 55 53.25 | +09 54 04.72 | 4.01 | Schneider et al. (2010) |
| SDSS J105602.38+003222.0 | 10 56 02.38 | +00 32 22.09 | 4.05 | Schneider et al. (2005) |

| | | | | |
|---|---|---|---|---|
| SDSS J105623.84+532532.8 | 10 56 23.85 | +53 25 32.86 | 4.14 | Pâris et al. (2017) |
| SDSS J105641.96+321521.9 | 10 56 41.97 | +32 15 21.92 | 4.10 | Schneider et al. (2010) |
| CXOMP J10569−0343 | 10 56 55.13 | −03 43 22.00 | 4.05 | Silverman et al. (2005) |
| SDSS J105658.75+173558.3 | 10 56 58.75 | +17 35 58.32 | 4.42 | Pâris et al. (2014) |
| SDSS J105705.37+191042.8 | 10 57 05.38 | +19 10 42.83 | 4.14 | Schneider et al. (2010) |
| SDSS J105727.78+205551.9 | 10 57 27.79 | +20 55 51.98 | 4.05 | Schneider et al. (2010) |
| SDSS J105814.57+421637.3 | 10 58 14.58 | +42 16 37.34 | 4.27 | Pâris et al. (2012) |
| SDSS J105833.81+443153.2 | 10 58 33.81 | +44 31 53.21 | 4.10 | Pâris et al. (2017) |
| SDSS J105857.08+110128.6 | 10 58 57.09 | +11 01 28.60 | 4.34 | Schneider et al. (2007) |
| PSS J1058+1245 | 10 58 58.33 | +12 45 56.00 | 4.33 | Djorgovski et al. (2001) |
| SDSS J105902.73+010404.0 | 10 59 02.73 | +01 04 04.05 | 4.09 | Schneider et al. (2005) |
| SDSS J105904.58+454822.9 | 10 59 04.59 | +45 48 22.94 | 4.89 | Schneider et al. (2007) |
| SDSS J105919.22+023428.7 | 10 59 19.22 | +02 34 28.75 | 4.74 | Schneider et al. (2005) |
| SDSS J105926.40+130643.9 | 10 59 26.41 | +13 06 43.95 | 4.12 | Schneider et al. (2007) |
| SDSS J105936.68+411337.0 | 10 59 36.69 | +41 13 37.00 | 4.77 | Pâris et al. (2017) |
| SDSS J110012.52+145105.3 | 11 00 12.53 | +14 51 05.36 | 4.29 | Schneider et al. (2007) |
| SDSS J110041.94+580001.3 | 11 00 41.94 | +58 00 01.36 | 4.78 | Pâris et al. (2017) |
| SDSS J110045.23+112239.1 | 11 00 45.24 | +11 22 39.14 | 4.74 | Schneider et al. (2007) |
| SDSS J110131.37−004248.3 | 11 01 31.38 | −00 42 48.38 | 4.81 | Pâris et al. (2017) |
| SDSS J110134.35+053133.8 | 11 01 34.36 | +05 31 33.87 | 5.00 | Schneider et al. (2005) |
| SDSS J110136.06+095101.4 | 11 01 36.07 | +09 51 01.45 | 4.90 | Pâris et al. (2014) |
| SDSS J110142.45+213725.1 | 11 01 42.46 | +21 37 25.19 | 4.13 | Schneider et al. (2010) |
| SDSS J110150.89+240922.4 | 11 01 50.89 | +24 09 22.43 | 4.64 | Schneider et al. (2010) |
| SDSS J110217.14+381048.3 | 11 02 17.15 | +38 10 48.36 | 4.88 | Schneider et al. (2007) |
| SDSS J110234.98+125404.3 | 11 02 34.98 | +12 54 04.37 | 4.13 | Schneider et al. (2007) |
| SDSS J110241.09+520707.3 | 11 02 41.09 | +52 07 07.35 | 4.24 | Pâris et al. (2017) |
| SDSS J110307.76+270417.6 | 11 03 07.77 | +27 04 17.67 | 4.07 | Schneider et al. (2010) |
| SDSS J110320.57+091948.1 | 11 03 20.57 | +09 19 48.15 | 4.28 | Schneider et al. (2005) |
| SDSS J110339.25+524834.4 | 11 03 39.26 | +52 48 34.43 | 4.12 | Pâris et al. (2017) |
| SDSS J110342.08+103727.7 | 11 03 42.09 | +10 37 27.73 | 4.03 | Schneider et al. (2005) |
| SDSS J110343.75+010049.6 | 11 03 43.75 | +01 00 49.67 | 4.38 | Pâris et al. (2014) |
| SDSS J110350.30+245146.6 | 11 03 50.30 | +24 51 46.68 | 4.84 | Schneider et al. (2010) |
| SDSS J110358.79+352516.2 | 11 03 58.79 | +35 25 16.24 | 4.05 | Pâris et al. (2012) |
| DELS J110421.59+213428.8 | 11 04 21.59 | +21 34 28.80 | 6.74 | Wang et al. (2018) |
| SDSS J110421.84+571918.6 | 11 04 21.85 | +57 19 18.69 | 4.00 | Pâris et al. (2017) |
| SDSS J110523.24+103918.1 | 11 05 23.25 | +10 39 18.19 | 4.24 | Pâris et al. (2014) |
| SDSS J110530.99+370317.8 | 11 05 30.99 | +37 03 17.86 | 4.12 | Pâris et al. (2012) |
| SDSS J110540.31+505245.4 | 11 05 40.32 | +50 52 45.50 | 4.11 | Pâris et al. (2017) |
| SDSS J110603.42+152549.1 | 11 06 03.43 | +15 25 49.15 | 4.12 | Pâris et al. (2014) |
| SDSS J110621.97+615049.6 | 11 06 21.98 | +61 50 49.70 | 4.07 | Pâris et al. (2017) |
| SDSS J110628.68+554055.0 | 11 06 28.68 | +55 40 55.02 | 4.56 | Pâris et al. (2017) |
| SDSS J110638.62+074558.6 | 11 06 38.63 | +07 45 58.69 | 4.31 | Schneider et al. (2005) |
| SDSS J110657.82+081643.3 | 11 06 57.83 | +08 16 43.35 | 4.29 | Schneider et al. (2005) |
| SDSS J110706.46+251505.0 | 11 07 06.47 | +25 15 05.02 | 4.38 | Pâris et al. (2017) |
| SDSS J110721.81+590932.2 | 11 07 21.82 | +59 09 32.27 | 4.10 | Pâris et al. (2017) |
| SDSS J110727.46+060011.6 | 11 07 27.46 | +06 00 11.70 | 4.09 | Pâris et al. (2017) |
| SDSS J110729.94+430635.9 | 11 07 29.95 | +43 06 35.99 | 4.23 | Pâris et al. (2017) |
| SDSS J110745.24+242836.4 | 11 07 45.24 | +24 28 36.43 | 4.67 | Schneider et al. (2010) |
| SDSS J110811.21+171551.2 | 11 08 11.22 | +17 15 51.29 | 4.24 | Schneider et al. (2010) |
| SDSS J110813.86−005944.5 | 11 08 13.86 | −00 59 44.53 | 4.03 | Pâris et al. (2017) |
| SDSS J110819.15−005823.9 | 11 08 19.15 | −00 58 23.96 | 4.60 | Schneider et al. (2005) |
| SDSS J110826.31+003706.7 | 11 08 26.32 | +00 37 06.77 | 4.40 | Schneider et al. (2005) |
| SDSS J110828.12+312550.8 | 11 08 28.13 | +31 25 50.85 | 4.10 | Pâris et al. (2017) |
| SDSS J110909.26+420851.5 | 11 09 09.27 | +42 08 51.54 | 4.02 | Schneider et al. (2007) |
| PSO J167.4726+56.9521 | 11 09 53.43 | +56 57 07.61 | 5.95 | Bañados et al. (2016) |
| SDSS J111008.61+024458.0 | 11 10 08.62 | +02 44 58.07 | 4.12 | Schneider et al. (2005) |
| SDSS J111012.62+433112.7 | 11 10 12.62 | +43 31 12.74 | 4.05 | Schneider et al. (2007) |

| | | | | |
|---|---|---|---|---|
| SDSS J111021.83+142001.8 | 11 10 21.84 | +14 20 01.89 | 4.16 | Schneider et al. (2007) |
| SDSS J111040.94+275522.6 | 11 10 40.95 | +27 55 22.68 | 4.37 | Schneider et al. (2010) |
| SDSS J111047.12+312732.4 | 11 10 47.12 | +31 27 32.45 | 4.11 | Schneider et al. (2007) |
| SDSS J111126.65+350921.4 | 11 11 26.66 | +35 09 21.47 | 4.11 | Schneider et al. (2007) |
| SDSS J111224.18+004630.3 | 11 12 24.18 | +00 46 30.35 | 4.04 | Schneider et al. (2005) |
| SDSS J111346.78+443301.5 | 11 13 46.79 | +44 33 01.50 | 4.42 | Schneider et al. (2007) |
| SDSS J111358.32+025333.6 | 11 13 58.32 | +02 53 33.65 | 4.87 | Schneider et al. (2005) |
| SDSS J111401.47−005321.2 | 11 14 01.48 | −00 53 21.22 | 4.60 | Schneider et al. (2005) |
| SDSS J111408.63+440227.3 | 11 14 08.63 | +44 02 27.37 | 4.27 | Pâris et al. (2017) |
| SDSS J111505.37−020239.1 | 11 15 05.37 | −02 02 39.12 | 4.25 | Pâris et al. (2012) |
| SDSS J111511.65+144512.0 | 11 15 11.65 | +14 45 12.09 | 4.26 | Schneider et al. (2007) |
| SDSS J111516.08+460234.6 | 11 15 16.09 | +46 02 34.65 | 4.17 | Schneider et al. (2007) |
| SDSS J111523.24+082918.4 | 11 15 23.24 | +08 29 18.46 | 4.64 | Schneider et al. (2005) |
| SDSS J111525.88−000223.0 | 11 15 25.89 | −00 02 23.04 | 4.20 | Pâris et al. (2012) |
| SDSS J111551.07+355209.6 | 11 15 51.07 | +35 52 09.60 | 4.26 | Pâris et al. (2017) |
| SDSS J111636.12+370410.3 | 11 16 36.12 | +37 04 10.36 | 4.04 | Schneider et al. (2007) |
| SDSS J111649.52+353434.3 | 11 16 49.53 | +35 34 34.38 | 4.47 | Schneider et al. (2007) |
| SDSS J111712.58+202704.2 | 11 17 12.59 | +20 27 04.22 | 4.04 | Pâris et al. (2014) |
| SDSS J111714.11+540919.7 | 11 17 14.12 | +54 09 19.75 | 4.70 | Schneider et al. (2005) |
| SDSS J111741.26+261039.2 | 11 17 41.26 | +26 10 39.26 | 4.64 | Schneider et al. (2010) |
| SDSS J111753.84+120141.5 | 11 17 53.85 | +12 01 41.51 | 4.03 | Schneider et al. (2007) |
| SDSS J111812.91+441122.3 | 11 18 12.91 | +44 11 22.30 | 4.02 | Pâris et al. (2017) |
| SDSS J111826.87+374431.0 | 11 18 26.87 | +37 44 31.06 | 4.67 | Pâris et al. (2012) |
| SDSS J111845.36−025007.9 | 11 18 45.37 | −02 50 07.94 | 4.11 | Pâris et al. (2012) |
| PSS J1118+3702 | 11 18 56.16 | +37 02 55.90 | 4.04 | Djorgovski et al. (2001) |
| SDSS J111920.64+345248.1 | 11 19 20.64 | +34 52 48.12 | 4.98 | Pâris et al. (2017) |
| SDSS J111936.19+201900.2 | 11 19 36.20 | +20 19 00.29 | 4.06 | Schneider et al. (2010) |
| DELS J104819.09−010940.21 | 10 48 19.09 | −01 09 40.21 | 6.63 | Wang et al. (2017) |
| SDSS J111957.09+281354.1 | 11 19 57.10 | +28 13 54.18 | 4.13 | Schneider et al. (2010) |
| ULAS J112001.48+064124.3 | 11 20 01.48 | +06 41 24.30 | 7.09 | Mortlock et al. (2011) |
| SDSS J112006.49+135559.1 | 11 20 06.49 | +13 55 59.18 | 4.05 | Schneider et al. (2007) |
| SDSS J112116.22+180230.1 | 11 21 16.22 | +18 02 30.11 | 4.25 | Schneider et al. (2010) |
| SDSS J112142.98+094825.3 | 11 21 42.99 | +09 48 25.38 | 4.10 | Schneider et al. (2005) |
| PS1 J112143.65−071839.69 | 11 21 43.65 | −07 18 39.69 | 5.71 | Yang et al. (2018) |
| SDSS J112207.75+315618.8 | 11 22 07.76 | +31 56 18.84 | 4.24 | Schneider et al. (2007) |
| SDSS J11227−0229 | 11 22 43.00 | −02 29 05.00 | 4.80 | Zheng et al. (2000) |
| SDSS J112250.04+134236.4 | 11 22 50.04 | +13 42 36.45 | 5.19 | Pâris et al. (2014) |
| SDSS J112253.50+005329.7 | 11 22 53.51 | +00 53 29.79 | 4.55 | Schneider et al. (2005) |
| SDSS J112311.13−004418.5 | 11 23 11.13 | −00 44 18.50 | 5.00 | Richards et al. (2006) |
| SDSS J112314.55+455512.0 | 11 23 14.56 | +45 55 12.03 | 4.30 | Schneider et al. (2007) |
| SDSS J112317.83+253506.4 | 11 23 17.83 | +25 35 06.43 | 4.53 | Pâris et al. (2017) |
| SDSS J112321.52+262929.8 | 11 23 21.52 | +26 29 29.80 | 4.05 | Schneider et al. (2010) |
| SDSS J112356.89+272109.4 | 11 23 56.90 | +27 21 09.50 | 4.57 | Schneider et al. (2010) |
| SDSS J112401.65+153434.2 | 11 24 01.65 | +15 34 34.28 | 4.78 | Schneider et al. (2007) |
| SDSS J112420.57−010743.6 | 11 24 20.57 | −01 07 43.66 | 4.77 | Pâris et al. (2012) |
| SDSS J112430.11+503835.3 | 11 24 30.12 | +50 38 35.32 | 4.01 | Pâris et al. (2017) |
| SDSS J112450.67+363710.3 | 11 24 50.68 | +36 37 10.39 | 4.81 | Schneider et al. (2007) |
| SDSS J112516.11+444844.9 | 11 25 16.11 | +44 48 44.91 | 5.11 | Pâris et al. (2017) |
| SDSS J112534.93+380149.3 | 11 25 34.94 | +38 01 49.33 | 4.62 | Schneider et al. (2007) |
| SDSS J112612.81+613500.7 | 11 26 12.82 | +61 35 00.77 | 4.02 | Pâris et al. (2017) |
| SDSS J112637.96+173458.5 | 11 26 37.97 | +17 34 58.55 | 5.22 | Schneider et al. (2010) |
| SDSS J112646.97+110842.7 | 11 26 46.97 | +11 08 42.71 | 4.26 | Pâris et al. (2017) |
| SDSS J112714.90+355613.7 | 11 27 14.90 | +35 56 13.79 | 4.75 | Schneider et al. (2007) |
| SDSS J112733.69+343008.8 | 11 27 33.69 | +34 30 08.81 | 4.04 | Pâris et al. (2017) |
| SDSS J112740.36+153514.4 | 11 27 40.36 | +15 35 14.41 | 4.06 | Schneider et al. (2007) |
| SDSS J112753.03+340306.8 | 11 27 53.04 | +34 03 06.87 | 4.63 | Schneider et al. (2010) |
| SDSS J112813.77+594213.7 | 11 28 13.78 | +59 42 13.73 | 4.32 | Pâris et al. (2017) |

| | | | | |
|---|---|---|---|---|
| PSO J172.1770+26.8866 | 11 28 42.48 | +26 53 12.00 | 5.77 | Bañados et al. (2016) |
| SDSS J112844.11+395336.2 | 11 28 44.11 | +39 53 36.23 | 4.71 | Schneider et al. (2007) |
| SDSS J112844.27+010428.7 | 11 28 44.28 | +01 04 28.71 | 4.09 | Pâris et al. (2012) |
| SDSS J112857.81+575910.1 | 11 28 57.82 | +57 59 10.12 | 5.00 | Pâris et al. (2017) |
| SDSS J112907.57+600240.9 | 11 29 07.58 | +60 02 40.99 | 4.28 | Pâris et al. (2017) |
| SDSS J112920.30+275124.4 | 11 29 20.30 | +27 51 24.44 | 4.35 | Schneider et al. (2010) |
| SDSS J112932.90+541854.8 | 11 29 32.91 | +54 18 54.85 | 4.38 | Schneider et al. (2005) |
| SDSS J112934.39+213702.4 | 11 29 34.39 | +21 37 02.45 | 4.02 | Schneider et al. (2010) |
| SDSS J112951.75+394700.9 | 11 29 51.75 | +39 47 00.91 | 4.62 | Pâris et al. (2017) |
| SDSS J112956.09−014212.4 | 11 29 56.09 | −01 42 12.44 | 4.87 | Schneider et al. (2005) |
| SDSS J113102.85+513225.2 | 11 31 02.85 | +51 32 25.24 | 4.20 | Schneider et al. (2005) |
| SDSS J113120.08+383156.2 | 11 31 20.08 | +38 31 56.27 | 4.03 | Pâris et al. (2017) |
| SDSS J113142.31+384854.6 | 11 31 42.31 | +38 48 54.65 | 4.05 | Schneider et al. (2007) |
| SDSS J113156.05+094504.5 | 11 31 56.05 | +09 45 04.55 | 4.08 | Schneider et al. (2005) |
| SDSS J113156.13+211526.5 | 11 31 56.14 | +21 15 26.51 | 4.20 | Schneider et al. (2010) |
| SDSS J113210.90+374027.5 | 11 32 10.91 | +37 40 27.52 | 4.07 | Pâris et al. (2012) |
| SDSS J113243.73+093152.3 | 11 32 43.73 | +09 31 52.30 | 4.03 | Schneider et al. (2005) |
| SDSS J113246.50+120901.6 | 11 32 46.50 | +12 09 01.70 | 5.17 | Schneider et al. (2007) |
| J113308.78+160355.7 | 11 33 08.78 | +16 03 55.70 | 5.61 | Yang et al. (2017) |
| SDSS J113402.44+252027.0 | 11 34 02.45 | +25 20 27.01 | 4.09 | Pâris et al. (2017) |
| J113414.23+082853.3 | 11 34 14.23 | +08 28 53.30 | 5.69 | Yang et al. (2017) |
| SDSS J113415.21+392826.0 | 11 34 15.21 | +39 28 26.07 | 4.80 | Schneider et al. (2007) |
| SDSS J113418.80+393852.6 | 11 34 18.80 | +39 38 52.67 | 4.11 | Pâris et al. (2012) |
| SDSS J113421.07+035200.8 | 11 34 21.08 | +03 52 00.86 | 4.15 | Schneider et al. (2005) |
| SDSS J113437.42+230303.6 | 11 34 37.43 | +23 03 03.67 | 4.14 | Schneider et al. (2010) |
| SDSS J113453.21+304735.6 | 11 34 53.21 | +30 47 35.61 | 4.64 | Schneider et al. (2007) |
| DELS J113508.93+501133.0 | 11 35 09.93 | +50 11 33.00 | 6.58 | Wang et al. (2018) |
| SDSS J113534.55+344433.8 | 11 35 34.55 | +34 44 33.85 | 4.03 | Schneider et al. (2007) |
| SDSS J113559.94+002422.5 | 11 35 59.95 | +00 24 22.59 | 4.06 | Pâris et al. (2017) |
| SDSS J113600.10+422553.9 | 11 36 00.10 | +42 25 53.93 | 4.21 | Schneider et al. (2007) |
| SDSS J113612.62+511010.8 | 11 36 12.63 | +51 10 10.81 | 4.09 | Schneider et al. (2005) |
| SDSS J113635.07+043919.1 | 11 36 35.07 | +04 39 19.19 | 4.28 | Schneider et al. (2005) |
| SDSS J113639.76+553402.9 | 11 36 39.76 | +55 34 02.96 | 4.10 | Pâris et al. (2017) |
| SDSS J113700.46+453321.6 | 11 37 00.47 | +45 33 21.60 | 4.36 | Pâris et al. (2017) |
| SDSS J113703.19+104312.1 | 11 37 03.19 | +10 43 12.12 | 4.48 | Schneider et al. (2005) |
| SDSS J11372+3549 | 11 37 17.73 | +35 49 57.00 | 6.01 | Fan et al. (2006) |
| SDSS J113736.71−001944.8 | 11 37 36.72 | −00 19 44.90 | 4.54 | Pâris et al. (2012) |
| SDSS J113736.88+543149.5 | 11 37 36.88 | +54 31 49.59 | 4.05 | Pâris et al. (2017) |
| SDSS J113745.67+012715.1 | 11 37 45.67 | +01 27 15.14 | 4.06 | Schneider et al. (2005) |
| SDSS J113833.42+582753.5 | 11 38 33.42 | +58 27 53.50 | 4.03 | Pâris et al. (2017) |
| SDSS J113846.57+135129.1 | 11 38 46.58 | +13 51 29.14 | 4.34 | Schneider et al. (2007) |
| SDSS J113906.95−014941.5 | 11 39 06.96 | −01 49 41.57 | 4.69 | Pâris et al. (2012) |
| PSS J1140+6205 | 11 40 08.66 | +62 05 30.29 | 4.52 | Djorgovski et al. (2001) |
| SDSS J114015.98+155928.9 | 11 40 15.98 | +15 59 28.98 | 4.05 | Schneider et al. (2007) |
| SDSS J114050.28+281221.1 | 11 40 50.29 | +28 12 21.12 | 4.67 | Pâris et al. (2017) |
| SDSS J114137.73+435326.4 | 11 41 37.74 | +43 53 26.45 | 4.18 | Schneider et al. (2007) |
| SDSS J114148.79+543224.5 | 11 41 48.80 | +54 32 24.55 | 4.34 | Schneider et al. (2005) |
| SDSS J114225.31+110217.4 | 11 42 25.31 | +11 02 17.40 | 4.60 | Schneider et al. (2005) |
| SDSS J114312.30+421140.2 | 11 43 12.30 | +42 11 40.25 | 4.59 | Schneider et al. (2007) |
| SDSS J114331.58+263831.7 | 11 43 31.58 | +26 38 31.80 | 4.07 | Pâris et al. (2017) |
| SDSS J1143+3808 | 11 43 38.35 | +38 08 28.82 | 5.80 | Jiang et al. (2016) |
| SDSS J114348.02+495724.2 | 11 43 48.03 | +49 57 24.20 | 4.03 | Schneider et al. (2005) |
| SDSS J114358.19+181540.7 | 11 43 58.19 | +18 15 40.73 | 4.27 | Schneider et al. (2010) |
| SDSS J114447.65+370434.6 | 11 44 47.66 | +37 04 34.62 | 4.01 | Schneider et al. (2007) |
| SDSS J114448.54+055709.7 | 11 44 48.55 | +05 57 09.78 | 4.79 | Schneider et al. (2005) |
| SDSS J114506.07+561823.6 | 11 45 06.08 | +56 18 23.60 | 4.05 | Pâris et al. (2017) |
| SDSS J114514.18+394715.9 | 11 45 14.19 | +39 47 15.98 | 4.07 | Schneider et al. (2007) |

| | | | | |
|---|---|---|---|---|
| SDSS J114614.44+571235.4 | 11 46 14.44 | +57 12 35.48 | 4.01 | Pâris et al. (2017) |
| J1146−0154 | 11 46 32.66 | −01 54 38.30 | 6.16 | Chehade et al. (2018) |
| BR 1144−0723 | 11 46 35.67 | −07 40 05.00 | 4.16 | Rabbette et al. (1998) |
| J1146+0124 | 11 46 48.42 | +01 24 20.10 | 6.27 | Chehade et al. (2018) |
| J1146−0005 | 11 46 58.89 | −00 05 37.70 | 6.30 | Chehade et al. (2018) |
| J114706.41−010958.2 | 11 47 06.41 | −01 09 58.20 | 5.31 | Yang et al. (2017) |
| SDSS J114708.00+591618.8 | 11 47 08.00 | +59 16 18.84 | 4.13 | Pâris et al. (2017) |
| SDSS J114716.29+293201.9 | 11 47 16.29 | +29 32 01.98 | 4.03 | Pâris et al. (2017) |
| SDSS J114723.38+161453.4 | 11 47 23.38 | +16 14 53.46 | 4.02 | Schneider et al. (2010) |
| SDSS J114736.03+115945.1 | 11 47 36.03 | +11 59 45.14 | 4.32 | Schneider et al. (2007) |
| ULAS J1148+0702 | 11 48 03.29 | +07 02 08.30 | 6.29 | Jiang et al. (2016) |
| SDSS J114814.60+180436.4 | 11 48 14.61 | +18 04 36.45 | 4.43 | Pâris et al. (2017) |
| RD J1148+5253 | 11 48 16.20 | +52 53 39.00 | 5.70 | Mahabal et al. (2005) |
| SDSS J114816.64+525150.3 | 11 48 16.65 | +52 51 50.31 | 6.44 | Pâris et al. (2017) |
| SDSS J114826.16+302019.3 | 11 48 26.17 | +30 20 19.31 | 5.13 | Schneider et al. (2010) |
| VIK J1148+0056 | 11 48 33.18 | +00 56 42.26 | 5.84 | Venemans et al. (2015b) |
| SDSS J114843.87+220429.1 | 11 48 43.88 | +22 04 29.15 | 4.26 | Schneider et al. (2010) |
| SDSS J114914.88+281308.7 | 11 49 14.89 | +28 13 08.74 | 4.56 | Schneider et al. (2010) |
| SDSS J114923.12+184857.2 | 11 49 23.12 | +18 48 57.23 | 4.28 | Pâris et al. (2017) |
| SDSS J114935.52+044026.6 | 11 49 35.52 | +04 40 26.66 | 4.01 | Schneider et al. (2005) |
| SDSS J114935.83+424034.2 | 11 49 35.84 | +42 40 34.23 | 4.14 | Pâris et al. (2017) |
| SDSS J114939.14+503400.6 | 11 49 39.14 | +50 34 00.65 | 4.30 | Schneider et al. (2007) |
| J114946.45+074850.6 | 11 49 46.45 | +07 48 50.60 | 5.66 | Yang et al. (2017) |
| SDSS J114958.53+375115.0 | 11 49 58.54 | +37 51 15.02 | 4.37 | Schneider et al. (2007) |
| SDSS J115053.15+242230.1 | 11 50 53.15 | +24 22 30.17 | 4.04 | Pâris et al. (2017) |
| SDSS J115151.31+181611.3 | 11 51 51.32 | +18 16 11.37 | 4.20 | Schneider et al. (2010) |
| SDSS J115158.26+030341.8 | 11 51 58.26 | +03 03 41.84 | 4.70 | Schneider et al. (2005) |
| SDSS J115207.34+030701.7 | 11 52 07.34 | +03 07 01.70 | 4.92 | Pâris et al. (2017) |
| VIK J1152+0055 | 11 52 21.27 | +00 55 36.69 | 6.37 | Matsuoka et al. (2016) |
| SDSS J115240.97+113513.7 | 11 52 40.97 | +11 35 13.76 | 4.25 | Schneider et al. (2007) |
| SDSS J115242.85+024649.8 | 11 52 42.85 | +02 46 49.85 | 4.01 | Pâris et al. (2012) |
| SDSS J115305.60+270347.9 | 11 53 05.61 | +27 03 47.92 | 4.15 | Pâris et al. (2017) |
| SDSS J115321.68+101113.0 | 11 53 21.68 | +10 11 13.02 | 4.16 | Schneider et al. (2005) |
| SDSS J115324.26+033210.8 | 11 53 24.27 | +03 32 10.84 | 4.12 | Pâris et al. (2012) |
| SDSS J115338.03+214453.9 | 11 53 38.04 | +21 44 53.97 | 4.15 | Pâris et al. (2017) |
| SDSS J115355.01+371828.3 | 11 53 55.01 | +37 18 28.35 | 4.16 | Pâris et al. (2012) |
| SDSS J115407.43+353315.3 | 11 54 07.44 | +35 33 15.36 | 4.07 | Schneider et al. (2007) |
| SDSS J115419.91+233357.2 | 11 54 19.92 | +23 33 57.27 | 5.01 | Schneider et al. (2010) |
| SDSS J115424.73+134145.7 | 11 54 24.73 | +13 41 45.79 | 5.01 | Schneider et al. (2007) |
| SDSS J115515.39+264057.0 | 11 55 15.39 | +26 40 57.06 | 4.19 | Schneider et al. (2010) |
| SDSS J115547.83+022716.0 | 11 55 47.84 | +02 27 16.09 | 4.32 | Schneider et al. (2005) |
| SDSS J115649.04+104228.1 | 11 56 49.04 | +10 42 28.20 | 4.05 | Pâris et al. (2017) |
| SDSS J115652.70+132622.3 | 11 56 52.71 | +13 26 22.40 | 4.06 | Schneider et al. (2007) |
| SDSS J115744.95+221754.9 | 11 57 44.95 | +22 17 54.92 | 4.67 | Schneider et al. (2010) |
| SDSS J115748.38+063711.9 | 11 57 48.39 | +06 37 11.93 | 5.14 | Pâris et al. (2014) |
| SDSS J115754.24−013815.8 | 11 57 54.25 | −01 38 15.82 | 4.38 | Pâris et al. (2017) |
| SDSS J115757.96+485655.7 | 11 57 57.97 | +48 56 55.78 | 4.29 | Schneider et al. (2007) |
| SDSS J115809.37+634253.1 | 11 58 09.38 | +63 42 53.16 | 4.46 | Pâris et al. (2017) |
| SDSS J115851.51+231917.4 | 11 58 51.52 | +23 19 17.50 | 4.03 | Pâris et al. (2017) |
| PSS J1159+1337 | 11 59 06.52 | +13 37 37.74 | 4.05 | Constantin et al. (2002) |
| SDSS J115921.85+144708.4 | 11 59 21.86 | +14 47 08.44 | 4.13 | Schneider et al. (2007) |
| SDSS J115922.20+262915.5 | 11 59 22.21 | +26 29 15.53 | 4.88 | Schneider et al. (2010) |
| SDSS J115923.69+084311.5 | 11 59 23.70 | +08 43 11.55 | 4.38 | Pâris et al. (2014) |
| SDSS J120003.65+381811.9 | 12 00 03.66 | +38 18 11.93 | 4.23 | Schneider et al. (2007) |
| SDSS J120004.34+080949.8 | 12 00 04.34 | +08 09 49.80 | 4.42 | Schneider et al. (2007) |
| SDSS J120021.14+361926.1 | 12 00 21.15 | +36 19 26.13 | 4.37 | Schneider et al. (2007) |
| PC 1158+4635 | 12 00 36.73 | +46 18 50.30 | 4.75 | Schneider, Schmidt, & Gunn (1989b) |

| | | | | |
|---|---|---|---|---|
| SDSS J120053.05+425640.3 | 12 00 53.05 | +42 56 40.35 | 4.10 | Schneider et al. (2007) |
| SDSS J120055.61+181733.0 | 12 00 55.62 | +18 17 33.01 | 5.00 | Schneider et al. (2010) |
| SDSS J120058.03+371238.0 | 12 00 58.03 | +37 12 38.04 | 4.78 | Schneider et al. (2007) |
| SDSS J120102.01+073648.1 | 12 01 02.01 | +07 36 48.19 | 4.46 | Schneider et al. (2007) |
| J1201+0133 | 12 01 03.02 | +01 33 56.40 | 6.06 | Matsuoka et al. (2018b) |
| SDSS J120110.31+211758.4 | 12 01 10.31 | +21 17 58.48 | 4.58 | Pâris et al. (2017) |
| SDSS J120131.56+053510.1 | 12 01 31.57 | +05 35 10.14 | 4.80 | Schneider et al. (2005) |
| SDSS J120206.48+361037.2 | 12 02 06.49 | +36 10 37.23 | 4.03 | Pâris et al. (2012) |
| SDSS J120207.78+323538.7 | 12 02 07.78 | +32 35 38.80 | 5.26 | Pâris et al. (2017) |
| HSC J1202−0057 | 12 02 46.37 | −00 57 01.70 | 5.93 | Matsuoka et al. (2016) |
| SDSS J120247.22+071722.1 | 12 02 47.23 | +07 17 22.14 | 4.48 | Schneider et al. (2007) |
| SDSS J120256.44+072038.9 | 12 02 56.44 | +07 20 38.98 | 4.81 | Schneider et al. (2007) |
| SDSS J120312.63−001118.8 | 12 03 12.63 | −00 11 18.80 | 4.57 | Wu et al. (2012) |
| SDSS J120418.13+080019.5 | 12 04 18.13 | +08 00 19.53 | 4.06 | Pâris et al. (2014) |
| SDSS J120441.73−002149.6 | 12 04 41.73 | −00 21 49.63 | 5.09 | Schneider et al. (2005) |
| HSC J1205−0000 | 12 05 05.10 | −00 00 27.97 | 6.85 | Matsuoka et al. (2016) |
| SDSS J120516.55+075100.4 | 12 05 16.56 | +07 51 00.47 | 4.89 | Pâris et al. (2017) |
| SDSS J120518.96+605009.8 | 12 05 18.97 | +60 50 09.87 | 4.17 | Pâris et al. (2017) |
| BR 1202−0725 | 12 05 23.13 | −07 42 33.00 | 4.69 | Rabbette et al. (1998) |
| SDSS J120523.94+245408.6 | 12 05 23.94 | +24 54 08.67 | 4.03 | Pâris et al. (2014) |
| SDSS J120546.38+264026.1 | 12 05 46.39 | +26 40 26.19 | 4.54 | Pâris et al. (2017) |
| SDSS J120610.60+371747.6 | 12 06 10.60 | +37 17 47.61 | 4.32 | Schneider et al. (2007) |
| SDSS J120622.41+462136.2 | 12 06 22.41 | +46 21 36.25 | 4.00 | Pâris et al. (2017) |
| SDSS J120640.72+033415.1 | 12 06 40.73 | +03 34 15.12 | 4.39 | Schneider et al. (2005) |
| SDSS J120715.45+595343.3 | 12 07 15.45 | +59 53 43.30 | 4.50 | Pâris et al. (2017) |
| SDSS J120725.27+321530.4 | 12 07 25.28 | +32 15 30.47 | 4.60 | Schneider et al. (2010) |
| SDSS J120728.25+445513.2 | 12 07 28.25 | +44 55 13.23 | 4.28 | Schneider et al. (2007) |
| SDSS J120730.84+153338.1 | 12 07 30.85 | +15 33 38.12 | 4.45 | Schneider et al. (2007) |
| ULAS J1207+0630 | 12 07 37.44 | +06 30 10.20 | 6.04 | Jiang et al. (2015) |
| HSC J1207−0005 | 12 07 54.14 | −00 05 53.30 | 6.01 | Matsuoka et al. (2016) |
| PSS J1208+6350 | 12 08 00.95 | +63 50 10.32 | 4.01 | Abazajian et al. (2004) |
| SDSS J120816.46+460440.1 | 12 08 16.46 | +46 04 40.10 | 4.06 | Pâris et al. (2017) |
| SDSS J12083+0010 | 12 08 23.80 | +00 10 28.00 | 5.27 | Zheng et al. (2000) |
| SDSS J120827.94+614325.7 | 12 08 27.94 | +61 43 25.79 | 4.09 | Pâris et al. (2017) |
| J120829.27+394339.72 | 12 08 29.27 | +39 43 39.72 | 4.94 | Wang et al. (2016) |
| SDSS J120831.12+095741.7 | 12 08 31.13 | +09 57 41.78 | 4.06 | Pâris et al. (2014) |
| SDSS J120831.51+640140.8 | 12 08 31.52 | +64 01 40.89 | 4.08 | Pâris et al. (2017) |
| SDSS J120842.23+262305.7 | 12 08 42.24 | +26 23 05.72 | 4.13 | Pâris et al. (2017) |
| SDSS J120852.66+211033.9 | 12 08 52.67 | +21 10 33.97 | 5.06 | Schneider et al. (2010) |
| J1208−0200 | 12 08 59.23 | −02 00 34.80 | 6.20 | Matsuoka et al. (2018b) |
| J1209−0006 | 12 09 23.99 | −00 06 46.50 | 5.86 | Chehade et al. (2018) |
| SDSS J120952.73+183147.2 | 12 09 52.73 | +18 31 47.21 | 5.15 | Pâris et al. (2017) |
| SDSS J121056.59+445336.7 | 12 10 56.59 | +44 53 36.73 | 4.01 | Pâris et al. (2017) |
| SDSS J121114.42+472710.5 | 12 11 14.42 | +47 27 10.55 | 4.08 | Pâris et al. (2017) |
| SDSS J121122.06+375402.9 | 12 11 22.06 | +37 54 03.00 | 4.75 | Schneider et al. (2007) |
| SDSS J121123.96+292044.1 | 12 11 23.96 | +29 20 44.15 | 4.06 | Pâris et al. (2017) |
| SDSS J121130.40+241708.9 | 12 11 30.40 | +24 17 08.96 | 4.23 | Schneider et al. (2010) |
| SDSS J121134.03+484235.9 | 12 11 34.03 | +48 42 35.91 | 4.54 | Pâris et al. (2017) |
| SDSS J121209.54+034749.9 | 12 12 09.54 | +03 47 49.93 | 4.04 | Schneider et al. (2005) |
| SDSS J121212.54+411837.5 | 12 12 12.54 | +41 18 37.54 | 4.10 | Pâris et al. (2017) |
| PSO J183.1124+05.0926 | 12 12 26.98 | +05 05 33.49 | 6.60 | Bañados et al. (2016) |
| SDSS J121329.57+400500.9 | 12 13 29.58 | +40 05 00.97 | 4.15 | Pâris et al. (2012) |
| SDSS J121409.83+035438.8 | 12 14 09.83 | +03 54 38.82 | 4.58 | Pâris et al. (2017) |
| SDSS J121410.58+010014.3 | 12 14 10.58 | +01 00 14.37 | 4.36 | Pâris et al. (2012) |
| SDSS J121447.82+273843.9 | 12 14 47.83 | +27 38 43.95 | 4.91 | Schneider et al. (2010) |
| SDSS J121451.11+375420.1 | 12 14 51.11 | +37 54 20.18 | 4.25 | Pâris et al. (2012) |
| SDSS J121510.36+375811.2 | 12 15 10.36 | +37 58 11.22 | 4.28 | Schneider et al. (2007) |

| | | | | |
|---|---|---|---|---|
| VIK J1215+0023 | 12 15 16.87 | +00 23 24.66 | 5.93 | Venemans et al. (2015b) |
| QPQ6 J121533.54−030925.1 | 12 15 33.54 | −03 09 25.10 | 4.00 | Prochaska et al. (2013) |
| SDSS J121535.33+191320.4 | 12 15 35.33 | +19 13 20.41 | 4.11 | Schneider et al. (2010) |
| SDSS J121537.77+545937.0 | 12 15 37.78 | +54 59 37.08 | 4.11 | Pâris et al. (2017) |
| SDSS J121542.52+253454.0 | 12 15 42.52 | +25 34 54.04 | 4.11 | Pâris et al. (2017) |
| SDSS J121607.57+415653.9 | 12 16 07.58 | +41 56 53.97 | 4.55 | Pâris et al. (2017) |
| SDSS J121609.28+532452.1 | 12 16 09.28 | +53 24 52.14 | 4.12 | Pâris et al. (2017) |
| SDSS J121613.65+435024.3 | 12 16 13.66 | +43 50 24.35 | 4.12 | Schneider et al. (2007) |
| SDSS J121627.57+053508.7 | 12 16 27.57 | +05 35 08.75 | 4.06 | Pâris et al. (2012) |
| DELS J121627.58+451910.7 | 12 16 27.58 | +45 19 10.70 | 6.65 | Wang et al. (2018) |
| SDSS J121636.75+134545.8 | 12 16 36.76 | +13 45 45.83 | 4.62 | Schneider et al. (2007) |
| SDSS J121643.74+624051.6 | 12 16 43.74 | +62 40 51.69 | 4.00 | Pâris et al. (2017) |
| PSO J184.3389+01.5284 | 12 17 21.34 | +01 31 42.47 | 6.20 | Bañados et al. (2016) |
| SDSS J121812.38+444544.5 | 12 18 12.39 | +44 45 44.56 | 4.48 | Pâris et al. (2017) |
| SDSS J121814.54+362709.8 | 12 18 14.55 | +36 27 09.89 | 4.21 | Pâris et al. (2012) |
| J1219+0050 | 12 19 05.34 | +00 50 37.50 | 6.01 | Chehade et al. (2018) |
| SDSS J121919.35−024323.1 | 12 19 19.35 | −02 43 23.17 | 4.03 | Pâris et al. (2012) |
| SDSS J121930.22+324318.0 | 12 19 30.22 | +32 43 18.09 | 4.04 | Schneider et al. (2010) |
| SDSS J121939.66+170500.4 | 12 19 39.67 | +17 05 00.46 | 4.08 | Pâris et al. (2014) |
| SDSS J122000.83+254230.7 | 12 20 00.83 | +25 42 30.74 | 4.03 | Schneider et al. (2010) |
| SDSS J122008.93+343642.3 | 12 20 08.93 | +34 36 42.40 | 4.35 | Schneider et al. (2007) |
| SDSS J122010.53+144625.1 | 12 20 10.53 | +14 46 25.15 | 4.27 | Schneider et al. (2007) |
| SDSS J122014.73+322538.3 | 12 20 14.73 | +32 25 38.37 | 4.51 | Pâris et al. (2017) |
| SDSS J122015.17+295101.0 | 12 20 15.17 | +29 51 01.10 | 4.00 | Pâris et al. (2017) |
| SDSS J122016.05+315253.0 | 12 20 16.06 | +31 52 53.09 | 4.90 | Schneider et al. (2010) |
| SDSS J122021.39+092135.8 | 12 20 21.39 | +09 21 35.87 | 4.13 | Schneider et al. (2005) |
| SDSS J122028.52+295124.1 | 12 20 28.52 | +29 51 24.13 | 4.09 | Schneider et al. (2010) |
| SDSS J122041.99+444218.2 | 12 20 42.00 | +44 42 18.29 | 4.58 | Pâris et al. (2017) |
| SDSS J122044.54+293329.1 | 12 20 44.55 | +29 33 29.11 | 4.07 | Pâris et al. (2017) |
| SDSS J122101.44+483613.4 | 12 21 01.45 | +48 36 13.43 | 4.42 | Schneider et al. (2007) |
| SDSS J122106.40+015957.7 | 12 21 06.41 | +01 59 57.73 | 4.06 | Pâris et al. (2012) |
| SDSS J122131.33+110526.0 | 12 21 31.33 | +11 05 26.05 | 4.12 | Schneider et al. (2005) |
| SDSS J122146.42+444528.0 | 12 21 46.42 | +44 45 28.05 | 5.19 | Schneider et al. (2005) |
| SDSS J122205.67+201412.1 | 12 22 05.67 | +20 14 12.13 | 4.03 | Pâris et al. (2014) |
| SDSS J122207.78+064736.3 | 12 22 07.78 | +06 47 36.32 | 4.11 | Schneider et al. (2007) |
| SDSS J122214.06+283704.6 | 12 22 14.06 | +28 37 04.66 | 4.22 | Schneider et al. (2010) |
| SDSS J122214.16+102609.1 | 12 22 14.17 | +10 26 09.16 | 4.13 | Schneider et al. (2005) |
| SDSS J122237.96+195842.9 | 12 22 37.96 | +19 58 42.93 | 5.13 | Schneider et al. (2010) |
| SDSS J122323.71+204818.3 | 12 23 23.71 | +20 48 18.39 | 4.68 | Pâris et al. (2017) |
| J122342.16+183955.39 | 12 23 42.16 | +18 39 55.39 | 4.55 | Wang et al. (2016) |
| SDSS J122349.16+351208.7 | 12 23 49.16 | +35 12 08.80 | 4.01 | Pâris et al. (2017) |
| SDSS J122359.34+112800.0 | 12 23 59.35 | +11 28 00.03 | 4.12 | Schneider et al. (2007) |
| SDSS J122445.26+375921.3 | 12 24 45.27 | +37 59 21.31 | 4.30 | Schneider et al. (2007) |
| SDSS J122448.77+103453.4 | 12 24 48.77 | +10 34 53.45 | 4.20 | Schneider et al. (2005) |
| SDSS J122546.49+303345.6 | 12 25 46.49 | +30 33 45.62 | 4.87 | Schneider et al. (2010) |
| SDSS J122546.79+231203.6 | 12 25 46.80 | +23 12 03.66 | 4.12 | Schneider et al. (2010) |
| SDSS J122600.68+005923.6 | 12 26 00.68 | +00 59 23.65 | 4.27 | Schneider et al. (2005) |
| PSS J1226+0950 | 12 26 23.80 | +09 50 04.00 | 4.34 | Djorgovski et al. (2001) |
| SDSS J122657.97+000938.4 | 12 26 57.97 | +00 09 38.42 | 4.18 | Schneider et al. (2005) |
| SDSS J122738.30+572749.0 | 12 27 38.30 | +57 27 49.00 | 4.00 | Pâris et al. (2017) |
| SDSS J122805.98+285202.8 | 12 28 05.98 | +28 52 02.87 | 4.56 | Schneider et al. (2010) |
| PSO J187.1047−02.5609 | 12 28 25.15 | −02 33 39.25 | 5.77 | Bañados et al. (2016) |
| PSO J187.3050+04.3243 | 12 29 13.21 | +04 19 27.70 | 5.89 | Bañados et al. (2014) |
| SDSS J123038.45+284437.2 | 12 30 38.46 | +28 44 37.27 | 4.51 | Schneider et al. (2010) |
| SDSS J123109.18+343037.1 | 12 31 09.19 | +34 30 37.19 | 4.22 | Schneider et al. (2010) |
| SDSS J123115.91−020506.1 | 12 31 15.91 | −02 05 06.18 | 4.14 | Schneider et al. (2005) |
| SDSS J123130.07+061824.7 | 12 31 30.08 | +06 18 24.74 | 4.34 | Schneider et al. (2007) |

| | | | | |
|---|---|---|---|---|
| SDSS J123145.74+355812.7 | 12 31 45.74 | +35 58 12.79 | 4.06 | Pâris et al. (2012) |
| SDSS J123153.22+371849.3 | 12 31 53.23 | +37 18 49.33 | 4.11 | Pâris et al. (2012) |
| SDSS J123239.29+525250.9 | 12 32 39.30 | +52 52 50.99 | 4.34 | Schneider et al. (2005) |
| SDSS J123333.47+062234.1 | 12 33 33.47 | +06 22 34.19 | 5.30 | Schneider et al. (2007) |
| SDSS J123347.21−014853.8 | 12 33 47.22 | −01 48 53.83 | 4.26 | Schneider et al. (2005) |
| SDSS J123356.29+522820.9 | 12 33 56.30 | +52 28 21.00 | 4.05 | Pâris et al. (2017) |
| SDSS J123427.43+292657.9 | 12 34 27.43 | +29 26 57.96 | 4.51 | Schneider et al. (2010) |
| SDSS J123452.55+361146.6 | 12 34 52.55 | +36 11 46.63 | 4.83 | Schneider et al. (2007) |
| SDSS J123455.97+453007.3 | 12 34 55.98 | +45 30 07.32 | 4.06 | Pâris et al. (2017) |
| SDSS J123511.60+153836.0 | 12 35 11.61 | +15 38 36.02 | 4.23 | Pâris et al. (2017) |
| SDSS J123525.82+014945.6 | 12 35 25.83 | +01 49 45.70 | 4.04 | Schneider et al. (2005) |
| SDSS J123526.40+181918.9 | 12 35 26.41 | +18 19 19.00 | 4.04 | Schneider et al. (2010) |
| PC 1233+4752 | 12 35 31.00 | +47 36 05.00 | 4.45 | Schneider, Schmidt, & Gunn (1994b) |
| SDSS J123555.21+335954.6 | 12 35 55.21 | +33 59 54.70 | 4.08 | Schneider et al. (2007) |
| SDSS J123607.27+012018.9 | 12 36 07.28 | +01 20 18.93 | 4.05 | Pâris et al. (2012) |
| SDSS J123623.03+182435.8 | 12 36 23.04 | +18 24 35.81 | 4.85 | Schneider et al. (2010) |
| SDSS J123628.26+342003.8 | 12 36 28.27 | +34 20 03.82 | 4.08 | Pâris et al. (2012) |
| SDSS J123643.29+172754.8 | 12 36 43.29 | +17 27 54.84 | 4.07 | Schneider et al. (2010) |
| B01.174 | 12 36 48.00 | +62 09 40.00 | 5.19 | Barger et al. (2002) |
| SDSS J123649.90+372854.4 | 12 36 49.90 | +37 28 54.43 | 4.22 | Pâris et al. (2012) |
| SDSS J123700.61+381244.0 | 12 37 00.61 | +38 12 44.08 | 4.09 | Pâris et al. (2017) |
| SDSS J123706.52+361516.8 | 12 37 06.53 | +36 15 16.89 | 4.13 | Pâris et al. (2017) |
| SDSS J123718.03+555741.3 | 12 37 18.04 | +55 57 41.36 | 4.05 | Pâris et al. (2017) |
| SDSS J123739.80+543425.4 | 12 37 39.81 | +54 34 25.45 | 4.00 | Pâris et al. (2017) |
| SDSS J123746.76+533342.8 | 12 37 46.76 | +53 33 42.82 | 4.10 | Schneider et al. (2005) |
| SDSS J123750.07+343047.7 | 12 37 50.08 | +34 30 47.73 | 4.36 | Schneider et al. (2007) |
| SDSS J123849.65+151147.0 | 12 38 49.65 | +15 11 47.07 | 4.25 | Schneider et al. (2007) |
| SDSS J123922.21+350407.2 | 12 39 22.22 | +35 04 07.26 | 4.49 | Schneider et al. (2007) |
| SDSS J123949.06+381509.3 | 12 39 49.07 | +38 15 09.32 | 4.12 | Pâris et al. (2012) |
| SDSS J123958.88+383804.2 | 12 39 58.88 | +38 38 04.22 | 4.10 | Pâris et al. (2012) |
| SDSS J124022.62+025915.1 | 12 40 22.63 | +02 59 15.11 | 4.05 | Schneider et al. (2005) |
| SDSS J124029.57+281742.4 | 12 40 29.58 | +28 17 42.45 | 4.21 | Pâris et al. (2017) |
| SDSS J124144.14+034809.2 | 12 41 44.14 | +03 48 09.27 | 4.60 | Pâris et al. (2017) |
| SDSS J124244.17+321741.5 | 12 42 44.17 | +32 17 41.58 | 4.39 | Schneider et al. (2010) |
| SDSS J124247.91+521306.7 | 12 42 47.92 | +52 13 06.72 | 5.04 | Pâris et al. (2017) |
| SDSS J124250.47−013338.5 | 12 42 50.47 | −01 33 38.53 | 4.29 | Schneider et al. (2005) |
| SDSS J124300.94+631855.7 | 12 43 00.94 | +63 18 55.79 | 4.28 | Pâris et al. (2017) |
| SDSS J124310.35+070118.4 | 12 43 10.36 | +07 01 18.47 | 4.16 | Schneider et al. (2010) |
| SDSS J124311.99+485602.8 | 12 43 11.99 | +48 56 02.88 | 4.04 | Schneider et al. (2005) |
| SDSS J124316.59+072139.8 | 12 43 16.60 | +07 21 39.81 | 4.15 | Pâris et al. (2014) |
| ULAS J1243+2529 | 12 43 40.82 | +25 29 23.80 | 5.83 | Bañados et al. (2014) |
| SDSS J124400.04+553406.8 | 12 44 00.04 | +55 34 06.85 | 4.62 | Schneider et al. (2005) |
| SDSS J124421.98+063152.5 | 12 44 21.99 | +06 31 52.59 | 4.04 | Pâris et al. (2012) |
| SDSS J124509.79+142543.7 | 12 45 09.80 | +14 25 43.78 | 4.11 | Schneider et al. (2007) |
| SDSS J124510.13+434837.9 | 12 45 10.13 | +43 48 37.92 | 4.82 | Schneider et al. (2007) |
| SDSS J124515.46+382247.5 | 12 45 15.47 | +38 22 47.54 | 4.94 | Schneider et al. (2010) |
| SDSS J124523.28+415433.2 | 12 45 23.28 | +41 54 33.20 | 4.19 | Pâris et al. (2012) |
| SDSS J124735.78+063842.6 | 12 47 35.79 | +06 38 42.66 | 4.74 | Pâris et al. (2012) |
| SDSS J124750.28+280128.7 | 12 47 50.28 | +28 01 28.73 | 4.10 | Schneider et al. (2010) |
| SDSS J124757.43−011925.7 | 12 47 57.43 | −01 19 25.79 | 4.17 | Pâris et al. (2017) |
| PSS J1248+3110 | 12 48 20.21 | +31 10 43.19 | 4.34 | Djorgovski et al. (2001) |
| SDSS J124825.34+194334.6 | 12 48 25.34 | +19 43 34.67 | 4.32 | Pâris et al. (2017) |
| SDSS J124839.16+213106.7 | 12 48 39.17 | +21 31 06.73 | 4.24 | Schneider et al. (2010) |
| SDSS J124902.62+043337.6 | 12 49 02.62 | +04 33 37.67 | 4.38 | Pâris et al. (2017) |
| SDSS J124922.70−014337.1 | 12 49 22.70 | −01 43 37.17 | 4.04 | Pâris et al. (2012) |
| SDSS J124939.10+303136.1 | 12 49 39.10 | +30 31 36.12 | 4.18 | Schneider et al. (2010) |
| PC 1247+3406 | 12 49 42.07 | +33 49 52.00 | 4.90 | Schneider, Schmidt, & Gunn (1991) |

| | | | | |
|---|---|---|---|---|
| SDSS J124948.79+554753.5 | 12 49 48.80 | +55 47 53.52 | 4.17 | Schneider et al. (2005) |
| SDSS J125025.40+183458.1 | 12 50 25.41 | +18 34 58.16 | 4.56 | Schneider et al. (2010) |
| PS1 J125049.27−065758.59 | 12 50 49.27 | −06 57 58.59 | 4.72 | Yang et al. (2018) |
| SDSS J125050.39+144805.0 | 12 50 50.40 | +14 48 05.09 | 4.08 | Schneider et al. (2007) |
| SDSS J12508+3130 | 12 50 51.93 | +31 30 22.00 | 6.13 | Fan et al. (2006) |
| SDSS J125147.91+041831.1 | 12 51 47.91 | +04 18 31.12 | 4.51 | Pâris et al. (2012) |
| SDSS J125156.64+332056.1 | 12 51 56.65 | +33 20 56.19 | 4.41 | Schneider et al. (2010) |
| SDSS J125200.83+234033.2 | 12 52 00.84 | +23 40 33.25 | 4.40 | Schneider et al. (2010) |
| SDSS J125205.88+214042.2 | 12 52 05.88 | +21 40 42.28 | 4.34 | Pâris et al. (2017) |
| SDSS J125223.89+431518.3 | 12 52 23.90 | +43 15 18.39 | 4.31 | Pâris et al. (2017) |
| XMM J125329.4+305539 | 12 53 29.41 | +30 55 39.43 | 5.08 | Khorunzhev et al. (2017) |
| PSS J1253−0228 | 12 53 36.36 | −02 28 07.81 | 4.03 | Péroux et al. (2001) |
| SDSS J125353.35+104603.1 | 12 53 53.35 | +10 46 03.19 | 4.91 | Schneider et al. (2010) |
| SDSS J125433.57−003922.6 | 12 54 33.57 | −00 39 22.67 | 4.28 | Schneider et al. (2005) |
| SDSS J125508.68−013200.7 | 12 55 08.69 | −01 32 00.74 | 4.13 | Pâris et al. (2012) |
| SDSS J125609.96+101950.1 | 12 56 09.97 | +10 19 50.13 | 4.08 | Schneider et al. (2010) |
| SDSS J125610.14+171353.9 | 12 56 10.14 | +17 13 53.92 | 4.34 | Schneider et al. (2010) |
| PSO J194.1290+25.5476 | 12 56 30.97 | +25 32 51.45 | 5.91 | Bañados et al. (2016) |
| SDSS J125655.36+362715.1 | 12 56 55.37 | +36 27 15.12 | 4.66 | Pâris et al. (2012) |
| SDSS J125716.01+481948.5 | 12 57 16.02 | +48 19 48.53 | 4.60 | Pâris et al. (2017) |
| SDSS J125718.02+374729.9 | 12 57 18.03 | +37 47 29.91 | 4.73 | Schneider et al. (2010) |
| SDSS J125757.17+254820.8 | 12 57 57.17 | +25 48 20.87 | 4.16 | Pâris et al. (2017) |
| SDSS J1257+6349 | 12 57 57.48 | +63 49 37.16 | 6.02 | Jiang et al. (2015) |
| SDSS J125759.21−011130.3 | 12 57 59.22 | −01 11 30.35 | 4.14 | Schneider et al. (2005) |
| SDSS J125802.62+022721.2 | 12 58 02.62 | +02 27 21.25 | 4.27 | Schneider et al. (2005) |
| SDSS J125832.51+141009.1 | 12 58 32.52 | +14 10 09.13 | 4.69 | Pâris et al. (2017) |
| SDSS J125850.93+615738.7 | 12 58 50.93 | +61 57 38.73 | 4.50 | Pâris et al. (2017) |
| SDSS J125911.73+160305.7 | 12 59 11.73 | +16 03 05.74 | 4.30 | Schneider et al. (2010) |
| SDSS J125955.72+471659.4 | 12 59 55.72 | +47 16 59.42 | 4.72 | Pâris et al. (2017) |
| SDSS J130010.93+381350.0 | 13 00 10.94 | +38 13 50.04 | 4.05 | Pâris et al. (2012) |
| SDSS J130018.44+181657.6 | 13 00 18.44 | +18 16 57.68 | 4.06 | Pâris et al. (2014) |
| SDSS J130039.12+032203.7 | 13 00 39.13 | +03 22 03.74 | 4.11 | Schneider et al. (2005) |
| SDSS J130055.01+454535.9 | 13 00 55.01 | +45 45 35.95 | 4.04 | Schneider et al. (2007) |
| SDSS J130109.13+360020.4 | 13 01 09.13 | +36 00 20.43 | 4.13 | Pâris et al. (2012) |
| SDSS J130110.95+252738.2 | 13 01 10.95 | +25 27 38.30 | 4.66 | Pâris et al. (2017) |
| SDSS J130128.48+101939.4 | 13 01 28.49 | +10 19 39.46 | 4.05 | Schneider et al. (2010) |
| SDSS J130129.22+385709.3 | 13 01 29.23 | +38 57 09.37 | 4.11 | Schneider et al. (2010) |
| SDSS J130137.24+124605.0 | 13 01 37.25 | +12 46 05.07 | 4.12 | Schneider et al. (2007) |
| SDSS J130149.48+044023.4 | 13 01 49.48 | +04 40 23.42 | 4.07 | Schneider et al. (2005) |
| SDSS J130152.55+221012.2 | 13 01 52.56 | +22 10 12.21 | 4.80 | Schneider et al. (2010) |
| SDSS J130204.98−011459.3 | 13 02 04.99 | −01 14 59.31 | 4.11 | Pâris et al. (2012) |
| SDSS J130206.68+281118.9 | 13 02 06.68 | +28 11 18.92 | 4.87 | Pâris et al. (2017) |
| SDSS J130212.04+053703.0 | 13 02 12.04 | +05 37 03.01 | 4.06 | Schneider et al. (2005) |
| SDSS J130215.72+550553.5 | 13 02 15.72 | +55 05 53.52 | 4.46 | Pâris et al. (2017) |
| SDSS J130216.13+003032.1 | 13 02 16.13 | +00 30 32.14 | 4.51 | Schneider et al. (2005) |
| SDSS J130221.73+241714.1 | 13 02 21.73 | +24 17 14.20 | 4.00 | Pâris et al. (2017) |
| SDSS J130240.37+231854.6 | 13 02 40.37 | +23 18 54.65 | 4.27 | Schneider et al. (2010) |
| SDSS J130328.28+214421.3 | 13 03 28.28 | +21 44 21.31 | 4.77 | Schneider et al. (2010) |
| SDSS J130332.40+621900.6 | 13 03 32.40 | +62 19 00.61 | 4.64 | Pâris et al. (2017) |
| SDSS J130332.75+053714.4 | 13 03 32.75 | +05 37 14.44 | 4.09 | Pâris et al. (2017) |
| SDSS J130355.12+445925.1 | 13 03 55.13 | +44 59 25.16 | 4.02 | Schneider et al. (2007) |
| SDSS J130502.28+052151.1 | 13 05 02.28 | +05 21 51.13 | 4.08 | Schneider et al. (2005) |
| SDSS J130553.29+064347.3 | 13 05 53.30 | +06 43 47.36 | 4.05 | Pâris et al. (2017) |
| SDSS J130600.05+293335.8 | 13 06 00.05 | +29 33 35.90 | 4.08 | Schneider et al. (2007) |
| SDSS J130607.68+063408.5 | 13 06 07.68 | +06 34 08.57 | 4.06 | Pâris et al. (2017) |
| SDSSp J130608.26+035626.3 | 13 06 08.26 | +03 56 26.30 | 5.99 | Fan et al. (2001a) |
| SDSS J130619.39+023658.9 | 13 06 19.39 | +02 36 58.94 | 4.80 | Pâris et al. (2017) |

| | | | | |
|---|---|---|---|---|
| SDSS J130625.16+352318.1 | 13 06 25.17 | +35 23 18.16 | 4.44 | Pâris et al. (2012) |
| SDSS J130707.14+150155.8 | 13 07 07.14 | +15 01 55.87 | 4.11 | Schneider et al. (2007) |
| SDSS J130722.44+460525.5 | 13 07 22.44 | +46 05 25.56 | 4.41 | Pâris et al. (2017) |
| SDSS J130806.17+625152.7 | 13 08 06.18 | +62 51 52.76 | 4.18 | Pâris et al. (2017) |
| SDSS J130810.74+565647.1 | 13 08 10.75 | +56 56 47.14 | 4.04 | Pâris et al. (2017) |
| SDSS J130906.75+144511.8 | 13 09 06.75 | +14 45 11.87 | 4.12 | Pâris et al. (2014) |
| SDSS J130917.13+165758.4 | 13 09 17.13 | +16 57 58.49 | 4.71 | Pâris et al. (2017) |
| SDSS J130951.81+551032.0 | 13 09 51.82 | +55 10 32.03 | 4.59 | Pâris et al. (2017) |
| PS1 J131013.11−063951.56 | 13 10 13.11 | −06 39 51.56 | 5.06 | Yang et al. (2018) |
| SDSS J131016.42+053042.0 | 13 10 16.42 | +05 30 42.04 | 4.51 | Pâris et al. (2012) |
| SDSS J131018.11+060153.0 | 13 10 18.11 | +06 01 53.03 | 4.24 | Schneider et al. (2005) |
| SDSS J131052.51−005533.2 | 13 10 52.51 | −00 55 33.23 | 4.16 | Schneider et al. (2005) |
| PSO J197.7198+25.5351 | 13 10 52.75 | +25 32 06.68 | 5.84 | Bañados et al. (2016) |
| SDSS J131056.86+105530.1 | 13 10 56.86 | +10 55 30.16 | 4.48 | Schneider et al. (2010) |
| MMK J131103.78−012403.9 | 13 11 03.78 | −01 24 03.90 | 4.39 | Martini, Mulchaey, & Kelson (2007) |
| SDSS J131106.20+560953.9 | 13 11 06.21 | +56 09 53.97 | 4.21 | Schneider et al. (2005) |
| SDSS J131111.56+280017.0 | 13 11 11.57 | +28 00 17.01 | 4.19 | Schneider et al. (2010) |
| SDSS J131137.38+381411.9 | 13 11 37.39 | +38 14 12.00 | 4.05 | Pâris et al. (2017) |
| SDSS J131221.37+580101.5 | 13 12 21.38 | +58 01 01.54 | 4.28 | Schneider et al. (2005) |
| SDSS J131234.08+230716.3 | 13 12 34.08 | +23 07 16.36 | 4.89 | Schneider et al. (2010) |
| SDSS J131303.38+523846.7 | 13 13 03.38 | +52 38 46.78 | 4.31 | Pâris et al. (2017) |
| SDSS J131313.09+103437.4 | 13 13 13.09 | +10 34 37.48 | 4.35 | Schneider et al. (2010) |
| SDSS J131318.32+162447.3 | 13 13 18.32 | +16 24 47.34 | 4.25 | Schneider et al. (2010) |
| SDSS J131428.97+281840.2 | 13 14 28.97 | +28 18 40.29 | 4.82 | Schneider et al. (2010) |
| QPQ6 J131433.79+281702.6 | 13 14 33.79 | +28 17 02.60 | 4.43 | Prochaska et al. (2013) |
| PSS J1315+2924B | 13 15 39.12 | +29 24 38.96 | 4.18 | Hennawi et al. (2010) |
| PSS J1315+2924 | 13 15 39.60 | +29 24 41.00 | 4.18 | Djorgovski et al. (2001) |
| SDSS J131600.91+211201.9 | 13 16 00.92 | +21 12 01.98 | 4.04 | Pâris et al. (2014) |
| DELS J131608.14+102832.8 | 13 16 08.14 | +10 28 32.80 | 6.35 | Wang et al. (2018) |
| SDSS J131620.93+011146.5 | 13 16 20.94 | +01 11 46.55 | 4.06 | Pâris et al. (2012) |
| SDSS J131649.66+565746.8 | 13 16 49.66 | +56 57 46.82 | 4.59 | Schneider et al. (2005) |
| SDSS J131712.17+272819.8 | 13 17 12.18 | +27 28 19.85 | 4.63 | Schneider et al. (2010) |
| J131720.78−023913.0 | 13 17 20.78 | −02 39 13.00 | 5.25 | Yang et al. (2017) |
| SDSS J131737.27+110533.1 | 13 17 37.28 | +11 05 33.10 | 4.76 | Pâris et al. (2017) |
| PSS J1317+3531 | 13 17 43.13 | +35 31 31.86 | 4.38 | Kennefick, Djorgovski, & de Carvalho (1995b) |
| SDSS J131808.44+215437.0 | 13 18 08.45 | +21 54 37.08 | 4.23 | Pâris et al. (2017) |
| ULAS J1319+0950 | 13 19 11.33 | +09 50 51.00 | 6.13 | Mortlock et al. (2009) |
| SDSS J131912.15+290501.3 | 13 19 12.15 | +29 05 01.33 | 4.05 | Schneider et al. (2007) |
| SDSS J131923.42+234517.4 | 13 19 23.43 | +23 45 17.46 | 4.09 | Schneider et al. (2010) |
| J131929.23+151305.0 | 13 19 29.23 | +15 13 05.00 | 4.50 | Yang et al. (2017) |
| SDSS J131939.25+245322.5 | 13 19 39.26 | +24 53 22.58 | 4.30 | Pâris et al. (2014) |
| SDSS J131959.76+545017.8 | 13 19 59.76 | +54 50 17.89 | 4.32 | Schneider et al. (2005) |
| SDSS J132000.74+431553.7 | 13 20 00.75 | +43 15 53.78 | 4.26 | Pâris et al. (2017) |
| SDSS J132014.08+112428.9 | 13 20 14.09 | +11 24 28.96 | 4.06 | Schneider et al. (2007) |
| SDSS J132028.44+103035.3 | 13 20 28.45 | +10 30 35.33 | 4.23 | Pâris et al. (2014) |
| SDSS J132106.07+623629.6 | 13 21 06.07 | +62 36 29.70 | 4.26 | Schneider et al. (2005) |
| SDSS J132110.81+003821.6 | 13 21 10.82 | +00 38 21.69 | 4.73 | Schneider et al. (2005) |
| SDSS J132122.97+163015.0 | 13 21 22.97 | +16 30 15.08 | 4.37 | Schneider et al. (2010) |
| SDSS J132124.54+294446.9 | 13 21 24.55 | +29 44 46.96 | 4.75 | Pâris et al. (2017) |
| SDSS J132134.37+143037.1 | 13 21 34.37 | +14 30 37.20 | 4.13 | Pâris et al. (2014) |
| SDSS J132136.47+303435.1 | 13 21 36.48 | +30 34 35.20 | 4.47 | Schneider et al. (2010) |
| SDSS J132228.96+273508.1 | 13 22 28.96 | +27 35 08.19 | 4.14 | Schneider et al. (2010) |
| SDSS J132304.92+135418.2 | 13 23 04.92 | +13 54 18.24 | 4.56 | Schneider et al. (2010) |
| J132319.69+291755.75 | 13 23 19.69 | +29 17 55.75 | 4.92 | Wang et al. (2016) |
| SDSS J132346.05+140517.5 | 13 23 46.05 | +14 05 17.59 | 4.07 | Schneider et al. (2010) |
| SDSS J132358.71+271221.1 | 13 23 58.72 | +27 12 21.19 | 4.03 | Schneider et al. (2010) |
| SDSS J132420.83+422554.6 | 13 24 20.84 | +42 25 54.61 | 4.04 | Pâris et al. (2017) |

| | | | | |
|---|---|---|---|---|
| SDSS J132447.26−031358.1 | 13 24 47.26 | −03 13 58.20 | 4.05 | Schneider et al. (2005) |
| SDSS J132521.65+033335.7 | 13 25 21.65 | +03 33 35.73 | 4.03 | Pâris et al. (2017) |
| SDSS J132536.24+232823.8 | 13 25 36.25 | +23 28 23.82 | 4.79 | Schneider et al. (2010) |
| SDSS J132554.11+125546.5 | 13 25 54.12 | +12 55 46.54 | 4.16 | Schneider et al. (2007) |
| SDSS J132603.95+060353.6 | 13 26 03.95 | +06 03 53.65 | 4.08 | Schneider et al. (2010) |
| PSS J1326+0743 | 13 26 11.85 | +07 43 58.39 | 4.12 | Djorgovski et al. (2001) |
| SDSS J132612.43+074041.7 | 13 26 12.44 | +07 40 41.75 | 4.12 | Pâris et al. (2017) |
| SDSS J132644.89+395953.8 | 13 26 44.89 | +39 59 53.82 | 4.02 | Pâris et al. (2012) |
| PSO J201.9222+57.5440 | 13 27 41.32 | +57 32 38.37 | 5.74 | Bañados et al. (2016) |
| SDSS J132749.05+451529.0 | 13 27 49.05 | +45 15 29.00 | 4.12 | Pâris et al. (2017) |
| SDSS J132757.81+240421.7 | 13 27 57.82 | +24 04 21.76 | 4.45 | Schneider et al. (2010) |
| SDSS J132808.53+202654.0 | 13 28 08.54 | +20 26 54.09 | 4.62 | Schneider et al. (2010) |
| SDSS J132825.16+444500.2 | 13 28 25.17 | +44 45 00.24 | 4.81 | Schneider et al. (2007) |
| SDSS J132825.28+382638.1 | 13 28 25.28 | +38 26 38.10 | 4.10 | Pâris et al. (2012) |
| SDSS J132853.66−022441.6 | 13 28 53.66 | −02 24 41.67 | 4.69 | Schneider et al. (2005) |
| SDSS J132856.67+085713.9 | 13 28 56.68 | +08 57 13.90 | 4.16 | Pâris et al. (2017) |
| SDSS J132859.73+325714.8 | 13 28 59.73 | +32 57 14.85 | 4.12 | Schneider et al. (2007) |
| SDSS J132923.41+234418.7 | 13 29 23.41 | +23 44 18.73 | 4.39 | Schneider et al. (2010) |
| SDSS J133043.47+180401.1 | 13 30 43.48 | +18 04 01.16 | 4.89 | Pâris et al. (2014) |
| SDSS J133125.56+025535.5 | 13 31 25.57 | +02 55 35.55 | 4.73 | Schneider et al. (2005) |
| 2SLAQ J133127.82+000421.1 | 13 31 27.82 | +00 04 21.12 | 4.19 | Croom et al. (2009) |
| SDSS J133128.64+432458.3 | 13 31 28.64 | +43 24 58.32 | 4.03 | Schneider et al. (2005) |
| BRI 1328−0433 | 13 31 30.87 | −04 48 51.00 | 4.22 | Kennefick, Djorgovski, & Meylan (1996) |
| SDSS J133145.22+484057.9 | 13 31 45.23 | +48 40 57.96 | 4.16 | Pâris et al. (2017) |
| SDSS J133156.30+073240.8 | 13 31 56.31 | +07 32 40.83 | 4.58 | Schneider et al. (2010) |
| SDSS J133203.86+553105.0 | 13 32 03.87 | +55 31 05.02 | 4.74 | Schneider et al. (2005) |
| SDSS J133211.90+031556.3 | 13 32 11.90 | +03 15 56.31 | 4.67 | Pâris et al. (2017) |
| SDSS J133230.66+370057.3 | 13 32 30.67 | +37 00 57.36 | 4.33 | Schneider et al. (2010) |
| SDSS J133250.08+465108.6 | 13 32 50.09 | +46 51 08.67 | 4.85 | Schneider et al. (2007) |
| J133257.45+220835.91 | 13 32 57.45 | +22 08 35.91 | 5.11 | Wang et al. (2016) |
| SDSS J133259.10+532028.1 | 13 32 59.10 | +53 20 28.15 | 4.52 | Pâris et al. (2017) |
| SDSS J133304.50+604736.0 | 13 33 04.51 | +60 47 36.09 | 4.43 | Pâris et al. (2017) |
| SDSS J133305.56+381552.1 | 13 33 05.57 | +38 15 52.15 | 4.14 | Schneider et al. (2007) |
| SDSS J133329.64+193814.4 | 13 33 29.65 | +19 38 14.42 | 4.31 | Schneider et al. (2010) |
| SDSS J133352.65−010135.0 | 13 33 52.65 | −01 01 35.01 | 4.03 | Pâris et al. (2017) |
| SDSS J133357.40+495327.6 | 13 33 57.41 | +49 53 27.62 | 4.18 | Schneider et al. (2007) |
| SDSS J133412.56+122020.7 | 13 34 12.56 | +12 20 20.71 | 5.12 | Schneider et al. (2007) |
| SDSS J133422.64+475033.6 | 13 34 22.64 | +47 50 33.60 | 4.96 | Pâris et al. (2017) |
| SDSS J133523.44+214020.7 | 13 35 23.45 | +21 40 20.75 | 4.06 | Schneider et al. (2010) |
| SDSS J133525.02+124411.1 | 13 35 25.03 | +12 44 11.18 | 4.14 | Schneider et al. (2007) |
| SDSS J133529.45+410125.9 | 13 35 29.45 | +41 01 25.95 | 4.27 | Pâris et al. (2017) |
| SDSS J133540.64+210807.3 | 13 35 40.65 | +21 08 07.33 | 4.15 | Schneider et al. (2010) |
| SDSS J13358+3533 | 13 35 50.80 | +35 33 16.00 | 5.93 | Fan et al. (2006) |
| 133556.24−032838.2 | 13 35 56.24 | −03 28 38.20 | 5.67 | Yang et al. (2017) |
| SDSS J133603.28+325226.2 | 13 36 03.29 | +32 52 26.27 | 4.02 | Schneider et al. (2007) |
| SDSS J133720.91+563329.0 | 13 37 20.92 | +56 33 29.02 | 4.46 | Schneider et al. (2005) |
| SDSS J133728.81+415539.8 | 13 37 28.81 | +41 55 39.85 | 5.03 | Schneider et al. (2007) |
| SDSS J133753.22+360223.0 | 13 37 53.22 | +36 02 23.05 | 4.07 | Pâris et al. (2012) |
| SDSS J133754.79+333721.8 | 13 37 54.80 | +33 37 21.82 | 4.03 | Schneider et al. (2007) |
| BRI 1335−0417 | 13 38 03.40 | −04 32 35.00 | 4.40 | Dietrich et al. (2003) |
| SDSS J133843.66+203242.8 | 13 38 43.66 | +20 32 42.80 | 4.93 | Pâris et al. (2017) |
| SDSS J133854.53+034620.5 | 13 38 54.53 | +03 46 20.56 | 4.37 | Pâris et al. (2012) |
| PSS J1339+5154 | 13 39 12.95 | +51 54 03.77 | 4.06 | Djorgovski et al. (2001) |
| SDSS J133952.62+360750.9 | 13 39 52.63 | +36 07 50.93 | 4.21 | Schneider et al. (2010) |
| SDSS J134009.78+365813.2 | 13 40 09.78 | +36 58 13.26 | 4.21 | Schneider et al. (2010) |
| SDSS J134012.12+201219.5 | 13 40 12.13 | +20 12 19.55 | 4.51 | Schneider et al. (2010) |
| SDSS J134015.03+392630.6 | 13 40 15.03 | +39 26 30.69 | 5.03 | Pâris et al. (2017) |

| | | | | |
|---|---|---|---|---|
| SDSS J134040.24+281328.1 | 13 40 40.24 | +28 13 28.16 | 5.34 | Schneider et al. (2007) |
| SDSS J134056.53+111044.9 | 13 40 56.54 | +11 10 44.97 | 4.58 | Schneider et al. (2007) |
| SDSS J134101.96+551624.4 | 13 41 01.96 | +55 16 24.44 | 4.25 | Schneider et al. (2005) |
| SDSS J134105.41+233254.6 | 13 41 05.41 | +23 32 54.67 | 4.48 | Schneider et al. (2010) |
| SDSS J134117.59+513855.8 | 13 41 17.59 | +51 38 55.89 | 4.40 | Schneider et al. (2007) |
| SDSS J134134.20+014157.6 | 13 41 34.20 | +01 41 57.68 | 4.65 | Pâris et al. (2017) |
| SDSS J134141.45+461110.3 | 13 41 41.46 | +46 11 10.30 | 5.02 | Schneider et al. (2007) |
| SDSS J134143.21+365405.4 | 13 41 43.22 | +36 54 05.45 | 4.13 | Pâris et al. (2012) |
| SDSS J134154.01+351005.7 | 13 41 54.02 | +35 10 05.71 | 5.23 | Pâris et al. (2017) |
| ULAS J134208.10+092838.61 | 13 42 08.10 | +09 28 38.61 | 7.54 | Bañados et al. (2018) |
| SDSS J134216.47+623837.7 | 13 42 16.47 | +62 38 37.76 | 4.02 | Schneider et al. (2005) |
| SDSS J134225.36+363815.1 | 13 42 25.37 | +36 38 15.12 | 4.08 | Schneider et al. (2010) |
| SDSS J134243.46+583850.0 | 13 42 43.47 | +58 38 50.07 | 4.86 | Pâris et al. (2017) |
| SDSS J134258.23+064745.6 | 13 42 58.23 | +06 47 45.63 | 4.23 | Schneider et al. (2010) |
| SDSS J134311.43+172212.1 | 13 43 11.44 | +17 22 12.16 | 4.19 | Schneider et al. (2010) |
| SDSS J134408.61+152125.0 | 13 44 08.62 | +15 21 25.05 | 4.87 | Schneider et al. (2010) |
| SDSS J134444.91+134422.9 | 13 44 44.92 | +13 44 22.99 | 4.23 | Schneider et al. (2010) |
| SDSS J134453.51+294519.6 | 13 44 53.51 | +29 45 19.64 | 4.66 | Schneider et al. (2007) |
| SDSS J134521.39+281822.2 | 13 45 21.39 | +28 18 22.24 | 4.08 | Schneider et al. (2007) |
| SDSS J134526.62+232949.3 | 13 45 26.62 | +23 29 49.37 | 5.06 | Schneider et al. (2010) |
| SDSS J134546.96−015940.3 | 13 45 46.97 | −01 59 40.38 | 4.70 | Schneider et al. (2005) |
| SDSS J134552.37+304201.6 | 13 45 52.37 | +30 42 01.65 | 4.02 | Pâris et al. (2017) |
| SDSS J134559.72+375858.3 | 13 45 59.72 | +37 58 58.32 | 4.20 | Pâris et al. (2012) |
| SDSS J134604.33+263332.3 | 13 46 04.33 | +26 33 32.39 | 4.16 | Schneider et al. (2007) |
| SDSS J134605.17+102337.1 | 13 46 05.17 | +10 23 37.10 | 4.37 | Schneider et al. (2010) |
| SDSS J134633.50+582509.1 | 13 46 33.51 | +58 25 09.19 | 4.02 | Pâris et al. (2017) |
| SDSS J134651.22+275317.9 | 13 46 51.23 | +27 53 17.98 | 4.03 | Pâris et al. (2014) |
| SDSS J134702.28−004207.0 | 13 47 02.28 | −00 42 07.01 | 4.52 | Pâris et al. (2012) |
| SDSS J134723.09+002158.7 | 13 47 23.09 | +00 21 58.79 | 4.30 | Schneider et al. (2005) |
| PSS J1347+4956 | 13 47 43.29 | +49 56 21.30 | 4.56 | Djorgovski et al. (2001) |
| SDSS J134750.98+633331.3 | 13 47 50.98 | +63 33 31.37 | 4.49 | Schneider et al. (2005) |
| SDSS J134817.51+465308.0 | 13 48 17.52 | +46 53 08.05 | 4.02 | Schneider et al. (2005) |
| SDSS J134819.87+181925.8 | 13 48 19.88 | +18 19 25.82 | 4.94 | Schneider et al. (2010) |
| SDSS J134821.50+243408.7 | 13 48 21.50 | +24 34 08.77 | 4.00 | Pâris et al. (2014) |
| SDSS J134831.67+172138.9 | 13 48 31.67 | +17 21 38.94 | 4.71 | Schneider et al. (2010) |
| SDSS J134838.48+510511.0 | 13 48 38.49 | +51 05 11.01 | 4.22 | Pâris et al. (2017) |
| SDSS J134910.08+212208.6 | 13 49 10.09 | +21 22 08.69 | 4.56 | Schneider et al. (2010) |
| SDSS J134939.77+124230.7 | 13 49 39.78 | +12 42 30.72 | 4.21 | Pâris et al. (2017) |
| SDSS J134946.13+350751.5 | 13 49 46.14 | +35 07 51.57 | 4.20 | Pâris et al. (2012) |
| SDSS J135025.69+450734.6 | 13 50 25.69 | +45 07 34.64 | 4.12 | Pâris et al. (2017) |
| SDSS J135029.64−000623.8 | 13 50 29.65 | −00 06 23.84 | 4.06 | Pâris et al. (2012) |
| SDSS J135033.39+321517.6 | 13 50 33.40 | +32 15 17.60 | 4.13 | Pâris et al. (2012) |
| SDSS J135057.86−004355.3 | 13 50 57.86 | −00 43 55.30 | 4.44 | Schneider et al. (2005) |
| SDSS J135112.33+265453.5 | 13 51 12.33 | +26 54 53.53 | 4.07 | Pâris et al. (2017) |
| SDSS J135113.75+224533.9 | 13 51 13.76 | +22 45 33.96 | 4.36 | Schneider et al. (2010) |
| SDSS J135127.30+075321.4 | 13 51 27.30 | +07 53 21.44 | 4.05 | Schneider et al. (2010) |
| SDSS J135127.53+472345.5 | 13 51 27.53 | +47 23 45.54 | 4.40 | Schneider et al. (2005) |
| SDSS J135134.47−003652.3 | 13 51 34.47 | −00 36 52.37 | 4.01 | Schneider et al. (2005) |
| SDSS J135219.88+014559.1 | 13 52 19.88 | +01 45 59.19 | 4.07 | Pâris et al. (2012) |
| SDSS J135229.60+455446.2 | 13 52 29.61 | +45 54 46.23 | 4.29 | Pâris et al. (2017) |
| SDSS J135230.49+531108.6 | 13 52 30.50 | +53 11 08.63 | 4.22 | Schneider et al. (2005) |
| SDSS J135242.74+493045.7 | 13 52 42.74 | +49 30 45.76 | 4.68 | Schneider et al. (2007) |
| SDSS J135249.38+431747.2 | 13 52 49.39 | +43 17 47.29 | 4.20 | Schneider et al. (2005) |
| SDSS J135249.82−031354.2 | 13 52 49.82 | −03 13 54.26 | 4.72 | Schneider et al. (2005) |
| SDSS J135252.20+164838.0 | 13 52 52.21 | +16 48 38.08 | 4.13 | Schneider et al. (2010) |
| SDSS J135402.19+401419.9 | 13 54 02.20 | +40 14 19.99 | 4.76 | Pâris et al. (2012) |
| SDSS J135422.99−003906.0 | 13 54 23.00 | −00 39 06.08 | 4.42 | Pâris et al. (2017) |

| | | | | |
|---|---|---|---|---|
| SDSS J135433.77+275144.3 | 13 54 33.78 | +27 51 44.31 | 4.24 | Schneider et al. (2010) |
| SDSS J135533.89+235156.0 | 13 55 33.89 | +23 51 56.05 | 4.11 | Pâris et al. (2014) |
| SDSS J135547.72+181957.7 | 13 55 47.73 | +18 19 57.77 | 4.56 | Schneider et al. (2010) |
| SDSS J135611.08+321322.7 | 13 56 11.09 | +32 13 22.79 | 4.23 | Pâris et al. (2017) |
| SDSS J135623.64+565539.8 | 13 56 23.64 | +56 55 39.88 | 4.16 | Pâris et al. (2017) |
| SDSS J135625.75+283009.9 | 13 56 25.75 | +28 30 10.00 | 4.21 | Pâris et al. (2017) |
| IMS J135747+530543 | 13 57 47.34 | +53 05 42.60 | 5.32 | Kim et al. (2019) |
| IMS J135856+514317 | 13 58 55.96 | +51 43 17.00 | 4.97 | Kim et al. (2019) |
| SDSS J135917.56+581250.8 | 13 59 17.56 | +58 12 50.88 | 4.03 | Pâris et al. (2017) |
| SDSS J135946.43+350438.3 | 13 59 46.43 | +35 04 38.31 | 4.23 | Schneider et al. (2007) |
| J1400−0011 | 14 00 28.79 | −00 11 51.50 | 6.04 | Chehade et al. (2018) |
| J1400−0125 | 14 00 29.99 | −01 25 21.00 | 6.04 | Chehade et al. (2018) |
| SDSS J140033.16+155415.5 | 14 00 33.16 | +15 54 15.52 | 4.26 | Schneider et al. (2010) |
| SDSS J140053.75+543012.1 | 14 00 53.75 | +54 30 12.20 | 4.17 | Schneider et al. (2007) |
| PSS J1401+4111 | 14 01 32.77 | +41 11 50.51 | 4.01 | Djorgovski et al. (2001) |
| SDSS J140135.98+515711.7 | 14 01 35.99 | +51 57 11.76 | 4.15 | Pâris et al. (2017) |
| SDSS J140145.26+031812.9 | 14 01 45.26 | +03 18 12.95 | 4.09 | Pâris et al. (2012) |
| SDSS J140146.53+024434.7 | 14 01 46.53 | +02 44 34.73 | 4.42 | Schneider et al. (2005) |
| IMS J140147+564145 | 14 01 46.97 | +56 41 44.80 | 4.98 | Kim et al. (2019) |
| PSO J210.4472+27.8263 | 14 01 47.34 | +27 49 35.03 | 6.14 | Bañados et al. (2016) |
| IMS J140150+514310 | 14 01 49.96 | +51 43 10.40 | 5.17 | Kim et al. (2019) |
| SDSS J140213.04+383532.3 | 14 02 13.05 | +38 35 32.32 | 4.15 | Schneider et al. (2007) |
| SDSS J140243.97+590959.0 | 14 02 43.97 | +59 09 59.02 | 4.14 | Schneider et al. (2005) |
| SDSS J140245.17+620220.5 | 14 02 45.18 | +62 02 20.56 | 4.07 | Schneider et al. (2005) |
| SDSS J140246.25+445013.1 | 14 02 46.25 | +44 50 13.19 | 4.05 | Pâris et al. (2017) |
| SDSS J140248.08+014634.0 | 14 02 48.08 | +01 46 34.09 | 4.16 | Schneider et al. (2005) |
| PSO J210.7277+40.4008 | 14 02 54.67 | +40 24 03.19 | 6.04 | Bañados et al. (2016) |
| SDSS J140300.23+432805.4 | 14 03 00.23 | +43 28 05.44 | 4.67 | Schneider et al. (2005) |
| SDSS J140303.14+070454.9 | 14 03 03.15 | +07 04 54.93 | 4.23 | Schneider et al. (2010) |
| PSO J210.8297+09.0474 | 14 03 19.13 | +09 02 50.99 | 5.88 | Jiang et al. (2015) |
| SDSS J140331.95+310745.1 | 14 03 31.95 | +31 07 45.13 | 4.12 | Pâris et al. (2012) |
| SDSS J140337.05+403205.9 | 14 03 37.06 | +40 32 05.95 | 4.08 | Schneider et al. (2007) |
| SDSS J140342.07+125252.5 | 14 03 42.07 | +12 52 52.58 | 4.91 | Schneider et al. (2007) |
| SDSS J140404.65+031403.8 | 14 04 04.65 | +03 14 03.86 | 4.90 | Schneider et al. (2005) |
| SDSS J140433.54+424512.6 | 14 04 33.54 | +42 45 12.61 | 4.22 | Schneider et al. (2005) |
| IMS J140440+565651 | 14 04 40.29 | +56 56 50.70 | 4.74 | Kim et al. (2019) |
| SDSS J140503.29+334149.7 | 14 05 03.30 | +33 41 49.80 | 4.42 | Schneider et al. (2007) |
| SDSS J140546.80+242126.0 | 14 05 46.81 | +24 21 26.04 | 4.05 | Schneider et al. (2010) |
| J1406−0116 | 14 06 29.12 | −01 16 11.20 | 6.33 | Chehade et al. (2018) |
| J1406−0144 | 14 06 46.88 | −01 44 02.60 | 6.10 | Chehade et al. (2018) |
| SDSS J140720.62+213645.0 | 14 07 20.62 | +21 36 45.08 | 4.08 | Schneider et al. (2010) |
| SDSS J140739.38+603036.1 | 14 07 39.38 | +60 30 36.11 | 4.77 | Schneider et al. (2005) |
| SDSS J140802.97+535154.4 | 14 08 02.98 | +53 51 54.43 | 4.06 | Pâris et al. (2017) |
| SDSS J140803.04+364753.4 | 14 08 03.04 | +36 47 53.43 | 4.73 | Pâris et al. (2017) |
| SDSS J140837.24+164503.0 | 14 08 37.25 | +16 45 03.01 | 4.06 | Schneider et al. (2010) |
| SDSS J140935.00+122657.3 | 14 09 35.00 | +12 26 57.33 | 4.55 | Schneider et al. (2007) |
| SDSS J141005.14+304628.8 | 14 10 05.14 | +30 46 28.88 | 4.26 | Schneider et al. (2010) |
| SDSS J141018.17+214223.4 | 14 10 18.18 | +21 42 23.44 | 4.29 | Schneider et al. (2010) |
| SDSS J14104+3856 | 14 10 26.20 | +38 56 53.00 | 4.75 | Chiu et al. (2005) |
| SDSS J141108.02+260404.9 | 14 11 08.03 | +26 04 04.97 | 4.03 | Schneider et al. (2010) |
| SDSS J14111+1217 | 14 11 11.33 | +12 17 37.00 | 5.93 | Fan et al. (2004) |
| SDSS J141154.39+422717.6 | 14 11 54.40 | +42 27 17.62 | 4.05 | Pâris et al. (2014) |
| SDSS J141254.36+541411.0 | 14 12 54.36 | +54 14 11.06 | 4.33 | Pâris et al. (2017) |
| SDSS J141258.83+163405.6 | 14 12 58.84 | +16 34 05.65 | 4.45 | Pâris et al. (2014) |
| SDSS J141315.36+000032.3 | 14 13 15.37 | +00 00 32.39 | 4.08 | Schneider et al. (2005) |
| SDSS J141332.35−004909.5 | 14 13 32.36 | −00 49 09.55 | 4.14 | Schneider et al. (2005) |
| SDSS J141359.69+095934.2 | 14 13 59.69 | +09 59 34.22 | 4.49 | Pâris et al. (2014) |

| | | | | |
|---|---|---|---|---|
| SDSS J141400.15+074125.4 | 14 14 00.16 | +07 41 25.42 | 4.00 | Pâris et al. (2012) |
| IMS J141432+573234 | 14 14 31.56 | +57 32 34.40 | 5.16 | Kim et al. (2019) |
| SDSS J141434.09+360840.9 | 14 14 34.09 | +36 08 40.98 | 4.02 | Pâris et al. (2012) |
| J1414+0130 | 14 14 39.54 | +01 30 36.50 | 5.94 | Matsuoka et al. (2018b) |
| SDSS J141440.51+331946.6 | 14 14 40.52 | +33 19 46.63 | 4.81 | Schneider et al. (2007) |
| SDSS J141517.15+322737.4 | 14 15 17.16 | +32 27 37.40 | 4.24 | Pâris et al. (2017) |
| SDSS J141534.91+033132.2 | 14 15 34.91 | +03 31 32.21 | 4.47 | Schneider et al. (2005) |
| SDSS J141551.58+120445.0 | 14 15 51.58 | +12 04 45.01 | 4.83 | Pâris et al. (2017) |
| SDSS J141600.05+133601.1 | 14 16 00.06 | +13 36 01.18 | 4.04 | Schneider et al. (2007) |
| J1416+0015 | 14 16 12.71 | +00 15 46.20 | 6.03 | Matsuoka et al. (2018b) |
| J1416+0147 | 14 16 53.01 | +01 47 02.20 | 6.07 | Chehade et al. (2018) |
| J1417+0117 | 14 17 28.67 | +01 17 12.40 | 6.02 | Matsuoka et al. (2018b) |
| SDSS J141741.56+253702.0 | 14 17 41.56 | +25 37 02.02 | 4.79 | Pâris et al. (2017) |
| PC 1415+3408 | 14 17 55.20 | +33 54 42.00 | 4.59 | Schneider, Schmidt, & Gunn (1997) |
| PSS J1418+4449 | 14 18 31.70 | +44 49 37.58 | 4.34 | Djorgovski et al. (2001) |
| SDSS J141839.99+314244.0 | 14 18 39.99 | +31 42 44.07 | 4.85 | Schneider et al. (2010) |
| SDSS J141847.87+062731.8 | 14 18 47.87 | +06 27 31.83 | 4.17 | Schneider et al. (2007) |
| SDSS J141912.03+534039.2 | 14 19 12.03 | +53 40 39.23 | 5.38 | Pâris et al. (2017) |
| SDSS J141914.19−015012.6 | 14 19 14.19 | −01 50 12.63 | 4.56 | Pâris et al. (2017) |
| SDSS J141924.18+193615.5 | 14 19 24.18 | +19 36 15.58 | 4.17 | Schneider et al. (2010) |
| SDSS J141954.10+163009.3 | 14 19 54.11 | +16 30 09.37 | 4.40 | Pâris et al. (2014) |
| SDSS J142004.11+022708.7 | 14 20 04.12 | +02 27 08.77 | 4.19 | Schneider et al. (2005) |
| SDSS J142013.67+300950.5 | 14 20 13.68 | +30 09 50.60 | 4.20 | Schneider et al. (2010) |
| SDSS J142019.98+321859.5 | 14 20 19.98 | +32 18 59.53 | 4.30 | Pâris et al. (2012) |
| SDSS J142023.77+283106.5 | 14 20 23.77 | +28 31 06.59 | 4.31 | Schneider et al. (2010) |
| SDSS J1420+2830B | 14 20 23.80 | +28 30 55.73 | 4.28 | Hennawi et al. (2010) |
| SDSS J142025.76+615510.1 | 14 20 25.76 | +61 55 10.18 | 4.45 | Pâris et al. (2017) |
| SDSS J142029.02−014050.1 | 14 20 29.03 | −01 40 50.10 | 4.13 | Pâris et al. (2012) |
| SDSS J142036.68+322456.5 | 14 20 36.69 | +32 24 56.51 | 4.22 | Pâris et al. (2012) |
| SDSS J142046.88+100206.3 | 14 20 46.89 | +10 02 06.38 | 4.56 | Schneider et al. (2010) |
| SDSS J142103.83+343332.0 | 14 21 03.83 | +34 33 32.02 | 4.96 | Schneider et al. (2007) |
| SDSS J142111.10+095337.5 | 14 21 11.10 | +09 53 37.59 | 4.08 | Schneider et al. (2010) |
| SDSS J142117.36+163127.8 | 14 21 17.37 | +16 31 27.87 | 4.00 | Schneider et al. (2010) |
| SDSS J142122.53+362832.8 | 14 21 22.54 | +36 28 32.86 | 4.09 | Pâris et al. (2012) |
| SDSS J142136.28+530113.8 | 14 21 36.28 | +53 01 13.89 | 4.29 | Pâris et al. (2017) |
| SDSS J142144.98+351315.4 | 14 21 44.99 | +35 13 15.48 | 4.56 | Schneider et al. (2007) |
| SDSS J142155.02+161620.5 | 14 21 55.03 | +16 16 20.58 | 4.05 | Pâris et al. (2014) |
| J1422+0011 | 14 22 00.23 | +00 11 03.00 | 5.89 | Chehade et al. (2018) |
| SDSS J142305.03+240507.9 | 14 23 05.04 | +24 05 07.90 | 4.12 | Pâris et al. (2017) |
| SDSS J142325.92+130300.7 | 14 23 25.92 | +13 03 00.70 | 5.02 | Schneider et al. (2007) |
| J1423−0018 | 14 23 31.71 | −00 18 09.10 | 6.13 | Matsuoka et al. (2018b) |
| SDSS J142408.35+024219.8 | 14 24 08.35 | +02 42 19.89 | 4.26 | Schneider et al. (2005) |
| SDSS J142444.16+200822.2 | 14 24 44.17 | +20 08 22.28 | 4.22 | Schneider et al. (2010) |
| SDSS J142454.47+401320.3 | 14 24 54.47 | +40 13 20.39 | 4.14 | Schneider et al. (2007) |
| AGES J142512.60+332051.0 | 14 25 12.60 | +33 20 51.02 | 4.03 | Kochanek et al. (2012) |
| NDWFS J14252+3254 | 14 25 16.33 | +32 54 09.00 | 5.85 | Cool et al. (2006) |
| J1425−0015 | 14 25 17.72 | −00 15 40.90 | 6.18 | Matsuoka et al. (2018b) |
| SDSS J142526.09+082718.4 | 14 25 26.10 | +08 27 18.46 | 4.94 | Schneider et al. (2007) |
| SDSS J142535.97−023934.4 | 14 25 35.98 | −02 39 34.42 | 4.75 | Schneider et al. (2005) |
| SDSS J142539.09+453504.0 | 14 25 39.10 | +45 35 04.06 | 4.03 | Schneider et al. (2005) |
| SDSS J142545.42+491654.0 | 14 25 45.43 | +49 16 54.05 | 4.21 | Schneider et al. (2007) |
| SDSS J142608.00+512103.2 | 14 26 08.00 | +51 21 03.30 | 4.24 | Schneider et al. (2005) |
| SDSS J142613.15+074351.3 | 14 26 13.15 | +07 43 51.30 | 4.03 | Pâris et al. (2017) |
| SDSS J142621.29+614732.9 | 14 26 21.29 | +61 47 32.99 | 4.34 | Pâris et al. (2017) |
| AGES J142628.52+335927.1 | 14 26 28.53 | +33 59 27.14 | 4.00 | Kochanek et al. (2012) |
| SDSS J142634.33+204336.3 | 14 26 34.33 | +20 43 36.38 | 4.82 | Schneider et al. (2010) |
| SDSS J142705.86+330817.8 | 14 27 05.87 | +33 08 17.90 | 4.68 | Pâris et al. (2017) |

| | | | | |
|---|---|---|---|---|
| SDSS J142709.04+220916.3 | 14 27 09.05 | +22 09 16.37 | 4.04 | Schneider et al. (2010) |
| SDSS J142711.24+220039.1 | 14 27 11.25 | +22 00 39.11 | 4.13 | Schneider et al. (2010) |
| PS1 J142721.56−050353.04 | 14 27 21.56 | −05 03 53.04 | 5.08 | Yang et al. (2018) |
| NDWFS J14275+3522 | 14 27 29.73 | +35 22 09.00 | 5.53 | Cool et al. (2006) |
| SDSS J142758.93+233608.9 | 14 27 58.94 | +23 36 08.91 | 4.08 | Pâris et al. (2014) |
| SDSS J142817.80+182107.7 | 14 28 17.80 | +18 21 07.76 | 4.02 | Pâris et al. (2014) |
| SDSS J142845.25+190330.2 | 14 28 45.25 | +19 03 30.22 | 4.30 | Schneider et al. (2010) |
| IMS J142854+564602 | 14 28 53.85 | +56 46 02.00 | 4.73 | Kim et al. (2019) |
| J1429−0104 | 14 29 03.08 | −01 04 43.40 | 6.80 | Matsuoka et al. (2018b) |
| SDSS J142911.84+632345.0 | 14 29 11.84 | +63 23 45.03 | 4.34 | Pâris et al. (2017) |
| AGES J142918.37+331922.9 | 14 29 18.38 | +33 19 22.97 | 4.99 | Kochanek et al. (2012) |
| J1429−0002 | 14 29 20.22 | −00 02 07.40 | 6.04 | Matsuoka et al. (2018b) |
| BTC40 J1429+011 | 14 29 26.40 | +01 19 54.00 | 4.84 | Monier et al. (2002) |
| SDSS J142935.54+435629.0 | 14 29 35.55 | +43 56 29.06 | 4.64 | Schneider et al. (2005) |
| NDWFS J14296+3304 | 14 29 37.93 | +33 04 16.00 | 5.39 | Cool et al. (2006) |
| SDSS J143003.95+144354.8 | 14 30 03.96 | +14 43 54.84 | 4.70 | Schneider et al. (2010) |
| SDSS J143007.34+483052.9 | 14 30 07.34 | +48 30 52.96 | 4.01 | Pâris et al. (2017) |
| NDWFS J143017.78+322003.4 | 14 30 17.78 | +32 20 03.40 | 4.75 | Glikman et al. (2010) |
| SDSS J143022.34+565712.5 | 14 30 22.34 | +56 57 12.50 | 4.56 | Schneider et al. (2005) |
| PSS J1430+2828 | 14 30 31.62 | +28 28 31.53 | 4.31 | Kennefick et al. (1995a) |
| SDSS J143047.08+060201.0 | 14 30 47.09 | +06 02 01.05 | 4.11 | Schneider et al. (2007) |
| AGES J143105.50+342717.8 | 14 31 05.51 | +34 27 17.87 | 4.58 | Kochanek et al. (2012) |
| SDSS J143107.51+342730.9 | 14 31 07.52 | +34 27 30.93 | 4.28 | Schneider et al. (2007) |
| SDSS J143111.58+053721.9 | 14 31 11.59 | +05 37 21.94 | 4.15 | Schneider et al. (2007) |
| PSO J217.9185−07.4120 | 14 31 40.45 | −07 24 43.47 | 6.14 | Bañados et al. (2016) |
| IMS J143156+560201 | 14 31 56.36 | +56 02 00.90 | 4.75 | Kim et al. (2019) |
| SDSS J143219.51+125619.2 | 14 32 19.51 | +12 56 19.25 | 4.18 | Schneider et al. (2007) |
| PSS J1432+3940 | 14 32 24.77 | +39 40 24.50 | 4.30 | Djorgovski et al. (2001) |
| SDSS J143239.00+375713.3 | 14 32 39.00 | +37 57 13.36 | 4.13 | Pâris et al. (2014) |
| 2SLAQ J143250.16+001756.3 | 14 32 50.16 | +00 17 56.37 | 4.84 | Croom et al. (2009) |
| SDSS J143253.52+024308.9 | 14 32 53.52 | +02 43 08.98 | 4.93 | Pâris et al. (2014) |
| SDSS J143300.89+103027.6 | 14 33 00.90 | +10 30 27.69 | 4.15 | Schneider et al. (2007) |
| AGES J143312.13+340206.2 | 14 33 12.13 | +34 02 06.22 | 4.23 | Kochanek et al. (2012) |
| NDWFS J143331.15+343248.3 | 14 33 31.15 | +34 32 48.30 | 4.15 | Glikman et al. (2010) |
| SDSS J143352.21+022713.9 | 14 33 52.21 | +02 27 13.97 | 4.62 | Schneider et al. (2005) |
| SDSS J143356.25+232222.8 | 14 33 56.26 | +23 22 22.82 | 4.14 | Schneider et al. (2007) |
| SDSS J143408.31+232229.9 | 14 34 08.31 | +23 22 29.97 | 4.00 | Schneider et al. (2007) |
| SDSS J143426.68+354930.9 | 14 34 26.68 | +35 49 30.93 | 4.16 | Pâris et al. (2014) |
| SDSS J143450.08+621159.0 | 14 34 50.08 | +62 11 59.02 | 4.01 | Pâris et al. (2017) |
| SDSS J143505.33+135144.2 | 14 35 05.33 | +13 51 44.21 | 4.02 | Pâris et al. (2014) |
| SDSS J143508.80+485521.1 | 14 35 08.81 | +48 55 21.10 | 4.78 | Pâris et al. (2017) |
| PSS J1435+3057 | 14 35 23.43 | +30 57 22.05 | 4.31 | Kennefick et al. (1995a) |
| AGES J143540.96+350325.6 | 14 35 40.96 | +35 03 25.60 | 4.80 | Kochanek et al. (2012) |
| SDSS J143551.00+200326.6 | 14 35 51.00 | +20 03 26.66 | 4.16 | Pâris et al. (2014) |
| SDSS J143556.32+435204.4 | 14 35 56.32 | +43 52 04.49 | 4.29 | Schneider et al. (2005) |
| SDSS J143558.77+214652.5 | 14 35 58.78 | +21 46 52.59 | 4.67 | Schneider et al. (2010) |
| SDSS J143605.00+213239.2 | 14 36 05.00 | +21 32 39.25 | 5.22 | Schneider et al. (2010) |
| SDSS J14361+5007 | 14 36 11.80 | +50 07 07.00 | 5.83 | Fan et al. (2006) |
| SDSS J143619.27−004855.4 | 14 36 19.27 | −00 48 55.43 | 4.00 | Pâris et al. (2012) |
| SDSS J143629.94+063507.9 | 14 36 29.94 | +06 35 07.93 | 4.78 | Schneider et al. (2007) |
| SDSS J143638.02+505107.8 | 14 36 38.02 | +50 51 07.82 | 4.00 | Schneider et al. (2005) |
| NDWFS J143658.34+333632.0 | 14 36 58.34 | +33 36 32.00 | 4.02 | Glikman et al. (2010) |
| SDSS J143658.89+223737.2 | 14 36 58.89 | +22 37 37.29 | 4.63 | Pâris et al. (2014) |
| J143704.81+070807.71 | 14 37 04.81 | +07 08 07.71 | 4.93 | Wang et al. (2016) |
| IMS J143705+522801 | 14 37 05.17 | +52 28 00.80 | 4.78 | Kim et al. (2019) |
| SDSS J143706.20+343659.2 | 14 37 06.20 | +34 36 59.21 | 4.37 | Schneider et al. (2007) |
| NDWFS J143732.67+335522.0 | 14 37 32.67 | +33 55 22.00 | 4.22 | Glikman et al. (2010) |

| | | | | |
|---|---|---|---|---|
| SDSS J143751.82+232313.3 | 14 37 51.83 | +23 23 13.35 | 5.31 | Schneider et al. (2010) |
| IMS J143757+515115 | 14 37 56.54 | +51 51 15.10 | 5.17 | Kim et al. (2019) |
| IMS J143804+573646 | 14 38 04.05 | +57 36 46.40 | 4.84 | Kim et al. (2019) |
| NDWFS J143813.85+350236.4 | 14 38 13.85 | +35 02 36.40 | 4.25 | Glikman et al. (2010) |
| SDSS J143814.57+441631.2 | 14 38 14.58 | +44 16 31.21 | 4.24 | Schneider et al. (2005) |
| SDSS J143824.76+362739.0 | 14 38 24.76 | +36 27 39.10 | 4.22 | Schneider et al. (2007) |
| IMS J143831+563946 | 14 38 30.83 | +56 39 46.40 | 4.82 | Kim et al. (2019) |
| PSS J1438+2538 | 14 38 35.51 | +25 38 30.71 | 4.24 | Kennefick, Djorgovski, & de Carvalho (1995b) |
| SDSS J143835.95+431459.2 | 14 38 35.95 | +43 14 59.24 | 4.68 | Schneider et al. (2005) |
| NDWFS J143839.68+351245.9 | 14 38 39.68 | +35 12 45.90 | 4.63 | Glikman et al. (2010) |
| SDSS J143843.19+460406.2 | 14 38 43.20 | +46 04 06.27 | 4.10 | Pâris et al. (2017) |
| SDSS J143850.48+055622.6 | 14 38 50.49 | +05 56 22.67 | 4.45 | Schneider et al. (2007) |
| SDSS J143906.17+552842.3 | 14 39 06.17 | +55 28 42.35 | 4.23 | Pâris et al. (2017) |
| SDSS J143932.14+252211.1 | 14 39 32.14 | +25 22 11.12 | 4.31 | Schneider et al. (2010) |
| IMS J143945+562627 | 14 39 44.88 | +56 26 26.60 | 4.70 | Kim et al. (2019) |
| SDSS J14398−0034 | 14 39 51.60 | −00 34 29.00 | 4.24 | Schneider et al. (2000) |
| SDSS J143952.15+133332.1 | 14 39 52.16 | +13 33 32.17 | 4.26 | Schneider et al. (2010) |
| SDSS J14398−0033 | 14 39 52.58 | −00 33 59.08 | 4.23 | Schneider et al. (2000) |
| J1440−0107 | 14 40 01.30 | −01 07 02.20 | 6.13 | Matsuoka et al. (2018b) |
| SDSS J144029.45+190800.6 | 14 40 29.45 | +19 08 00.66 | 4.77 | Schneider et al. (2010) |
| SDSS J144031.80+455243.9 | 14 40 31.80 | +45 52 43.90 | 4.15 | Pâris et al. (2017) |
| SDSS J144042.48+082201.9 | 14 40 42.48 | +08 22 01.97 | 4.63 | Schneider et al. (2010) |
| SDSS J144042.56+272922.7 | 14 40 42.57 | +27 29 22.72 | 4.00 | Schneider et al. (2010) |
| SDSS J144117.46+035910.5 | 14 41 17.46 | +03 59 10.56 | 4.29 | Schneider et al. (2005) |
| SDSS J144237.42+304921.4 | 14 42 37.43 | +30 49 21.46 | 4.75 | Schneider et al. (2007) |
| SDSS J144255.56+590949.9 | 14 42 55.56 | +59 09 49.96 | 4.34 | Schneider et al. (2005) |
| SDSS J144258.78+173214.4 | 14 42 58.78 | +17 32 14.46 | 4.11 | Pâris et al. (2014) |
| SDSS J144317.80+452846.9 | 14 43 17.80 | +45 28 46.96 | 4.01 | Pâris et al. (2017) |
| PSS J1443+2724 | 14 43 31.17 | +27 24 36.78 | 4.43 | Kennefick et al. (1995a) |
| PSS J1443+5856 | 14 43 40.70 | +58 56 53.24 | 4.31 | Djorgovski et al. (2001) |
| SDSS J144350.66+362315.1 | 14 43 50.67 | +36 23 15.14 | 5.12 | Schneider et al. (2007) |
| SDSS J144352.94+060533.1 | 14 43 52.95 | +06 05 33.16 | 4.89 | Schneider et al. (2007) |
| SDSS J144407.63−010152.7 | 14 44 07.63 | −01 01 52.78 | 4.54 | Schneider et al. (2005) |
| SDSS J144413.26+004836.7 | 14 44 13.26 | +00 48 36.70 | 4.78 | Richards et al. (2006) |
| SDSS J144419.21+463336.9 | 14 44 19.22 | +46 33 36.98 | 4.34 | Schneider et al. (2007) |
| SDSS J144420.79+380000.5 | 14 44 20.80 | +38 00 00.57 | 4.31 | Schneider et al. (2005) |
| SDSS J144428.63−012343.9 | 14 44 28.63 | −01 23 44.00 | 4.20 | Pâris et al. (2017) |
| SDSS J144526.31+263626.5 | 14 45 26.31 | +26 36 26.53 | 4.11 | Schneider et al. (2010) |
| SDSS J144617.35−010131.1 | 14 46 17.36 | −01 01 31.16 | 4.17 | Schneider et al. (2005) |
| SDSS J144638.48+285715.5 | 14 46 38.49 | +28 57 15.59 | 4.01 | Schneider et al. (2010) |
| SDSS J144649.47+213920.8 | 14 46 49.47 | +21 39 20.87 | 4.35 | Pâris et al. (2014) |
| SDSS J144656.04+395219.8 | 14 46 56.05 | +39 52 19.82 | 4.84 | Pâris et al. (2014) |
| SDSS J144713.04−012158.5 | 14 47 13.04 | −01 21 58.58 | 4.03 | Schneider et al. (2005) |
| SDSS J144717.97+040112.4 | 14 47 17.98 | +04 01 12.48 | 4.52 | Schneider et al. (2005) |
| SDSS J144734.00+391639.5 | 14 47 34.00 | +39 16 39.52 | 4.02 | Pâris et al. (2014) |
| SDSS J144734.09+102513.2 | 14 47 34.10 | +10 25 13.20 | 4.69 | Schneider et al. (2010) |
| SDSS J144827.81+281059.5 | 14 48 27.82 | +28 10 59.54 | 4.66 | Schneider et al. (2010) |
| SDSS J144853.29+190205.7 | 14 48 53.29 | +19 02 05.78 | 4.87 | Schneider et al. (2010) |
| SDSS J144905.90+431039.0 | 14 49 05.91 | +43 10 39.03 | 4.25 | Schneider et al. (2005) |
| SDSS J145004.78+240658.7 | 14 50 04.79 | +24 06 58.77 | 4.05 | Schneider et al. (2010) |
| SDSS J145005.79+334142.6 | 14 50 05.80 | +33 41 42.67 | 4.06 | Pâris et al. (2012) |
| SDSS J145020.11+553716.4 | 14 50 20.11 | +55 37 16.40 | 4.23 | Pâris et al. (2017) |
| SDSS J145050.18+340637.6 | 14 50 50.18 | +34 06 37.68 | 4.29 | Schneider et al. (2007) |
| SDSS J145103.72+403700.0 | 14 51 03.73 | +40 37 00.06 | 4.21 | Pâris et al. (2014) |
| SDSS J145107.93+025615.6 | 14 51 07.94 | +02 56 15.64 | 4.48 | Schneider et al. (2005) |
| SDSS J14513−0104 | 14 51 18.73 | −01 04 46.00 | 4.67 | Zheng et al. (2000) |
| SDSS J145130.32+170929.5 | 14 51 30.33 | +17 09 29.51 | 4.08 | Pâris et al. (2017) |

| | | | | |
|---|---|---|---|---|
| SDSS J145201.55+410443.9 | 14 52 01.56 | +41 04 43.98 | 4.14 | Pâris et al. (2017) |
| SDSS J145211.50+422429.6 | 14 52 11.50 | +42 24 29.63 | 4.81 | Pâris et al. (2014) |
| SDSS J145212.86+023526.3 | 14 52 12.86 | +02 35 26.35 | 4.90 | Schneider et al. (2005) |
| SDSS J145223.60+331207.7 | 14 52 23.60 | +33 12 07.76 | 4.20 | Pâris et al. (2012) |
| SDSS J145229.37+595156.2 | 14 52 29.37 | +59 51 56.29 | 4.02 | Pâris et al. (2017) |
| SDSS J145247.72+115620.1 | 14 52 47.72 | +11 56 20.12 | 4.03 | Schneider et al. (2007) |
| PC 1450+3404 | 14 53 00.60 | +33 52 08.00 | 4.19 | Schneider, Schmidt, & Gunn (1997) |
| SDSS J145342.10+165558.2 | 14 53 42.10 | +16 55 58.29 | 4.19 | Pâris et al. (2014) |
| SDSS J145347.17+055732.3 | 14 53 47.17 | +05 57 32.33 | 4.04 | Schneider et al. (2010) |
| SDSS J145350.37+610109.2 | 14 53 50.38 | +61 01 09.29 | 4.13 | Pâris et al. (2017) |
| SDSS J145408.44+342029.2 | 14 54 08.44 | +34 20 29.29 | 4.20 | Schneider et al. (2007) |
| SDSS J145448.07+220924.6 | 14 54 48.08 | +22 09 24.61 | 4.57 | Pâris et al. (2017) |
| SDSS J145510.73+593715.4 | 14 55 10.73 | +59 37 15.49 | 4.59 | Pâris et al. (2017) |
| SDSS J145512.99+453338.5 | 14 55 12.99 | +45 33 38.52 | 4.27 | Schneider et al. (2007) |
| SDSS J145527.92+552647.2 | 14 55 27.93 | +55 26 47.24 | 4.29 | Pâris et al. (2017) |
| SDSS J145545.32+004447.2 | 14 55 45.32 | +00 44 47.22 | 4.27 | Pâris et al. (2017) |
| PSS J1456+2007 | 14 56 28.97 | +20 07 27.09 | 4.26 | Péroux et al. (2001) |
| SDSS J145716.14+235055.3 | 14 57 16.14 | +23 50 55.31 | 4.19 | Schneider et al. (2010) |
| SDSS J145747.66+575332.1 | 14 57 47.67 | +57 53 32.19 | 4.35 | Schneider et al. (2005) |
| SDSS J145805.99+332723.0 | 14 58 06.00 | +33 27 23.07 | 4.83 | Schneider et al. (2007) |
| SDSS J145824.21+485119.4 | 14 58 24.21 | +48 51 19.47 | 4.14 | Pâris et al. (2017) |
| SDSS J145834.53+290653.1 | 14 58 34.54 | +29 06 53.13 | 4.01 | Pâris et al. (2012) |
| SDSS J145835.16+023820.7 | 14 58 35.17 | +02 38 20.73 | 4.10 | Pâris et al. (2012) |
| SDSS J145837.49+083131.1 | 14 58 37.50 | +08 31 31.10 | 4.08 | Pâris et al. (2017) |
| SDSS J145916.97+013405.9 | 14 59 16.97 | +01 34 05.98 | 4.11 | Pâris et al. (2012) |
| PSS J1500+5829 | 15 00 07.67 | +58 29 38.00 | 4.22 | Djorgovski et al. (2001) |
| SDSS J150027.89+434200.9 | 15 00 27.90 | +43 42 00.90 | 4.63 | Schneider et al. (2007) |
| SDSS J150052.61+231837.4 | 15 00 52.62 | +23 18 37.49 | 4.01 | Schneider et al. (2010) |
| SDSS J150128.23+193411.3 | 15 01 28.24 | +19 34 11.40 | 4.28 | Schneider et al. (2010) |
| SDSS J150155.35+262017.5 | 15 01 55.35 | +26 20 17.57 | 4.23 | Schneider et al. (2010) |
| SDSS J150216.63+323203.3 | 15 02 16.63 | +32 32 03.31 | 4.15 | Schneider et al. (2007) |
| SDSS J150220.46+465233.5 | 15 02 20.46 | +46 52 33.60 | 4.20 | Pâris et al. (2017) |
| SDSS J150302.42+160807.9 | 15 03 02.43 | +16 08 07.98 | 4.29 | Schneider et al. (2010) |
| SDSS J150358.25+425642.3 | 15 03 58.26 | +42 56 42.32 | 4.02 | Pâris et al. (2017) |
| SDSS J150524.42+121126.5 | 15 05 24.42 | +12 11 26.57 | 4.37 | Schneider et al. (2010) |
| SDSS J150527.34+573632.1 | 15 05 27.35 | +57 36 32.16 | 4.38 | Pâris et al. (2017) |
| SDSS J150609.86+101222.1 | 15 06 09.87 | +10 12 22.16 | 4.70 | Pâris et al. (2014) |
| SDSS J150619.21+045553.9 | 15 06 19.21 | +04 55 53.91 | 4.64 | Pâris et al. (2017) |
| SDSS J150631.75+113149.7 | 15 06 31.75 | +11 31 49.71 | 4.53 | Schneider et al. (2010) |
| SDSS J150636.19+053532.8 | 15 06 36.19 | +05 35 32.84 | 4.32 | Schneider et al. (2010) |
| PSS J1506+5220 | 15 06 54.55 | +52 20 04.74 | 4.15 | Trump et al. (2006) |
| SDSS J150655.23+023732.0 | 15 06 55.24 | +02 37 32.01 | 4.96 | Pâris et al. (2012) |
| SDSS J150655.73+534709.6 | 15 06 55.74 | +53 47 09.63 | 4.14 | Pâris et al. (2017) |
| SDSS J150711.72+143434.0 | 15 07 11.73 | +14 34 34.10 | 4.30 | Schneider et al. (2010) |
| SDSS J150730.62+553710.9 | 15 07 30.62 | +55 37 10.93 | 4.50 | Pâris et al. (2017) |
| SDSS J150731.89+435429.6 | 15 07 31.89 | +43 54 29.69 | 4.13 | Pâris et al. (2017) |
| SDSS J150802.29+430645.4 | 15 08 02.29 | +43 06 45.45 | 4.68 | Schneider et al. (2007) |
| SDSS J150803.09+370722.8 | 15 08 03.10 | +37 07 22.81 | 4.02 | Pâris et al. (2014) |
| SDSS J150817.57+432635.7 | 15 08 17.57 | +43 26 35.76 | 4.04 | Schneider et al. (2007) |
| SDSS J150831.26−020925.1 | 15 08 31.27 | −02 09 25.17 | 4.00 | Schneider et al. (2005) |
| SDSS J150834.34+505246.8 | 15 08 34.34 | +50 52 46.86 | 4.42 | Schneider et al. (2005) |
| SDSS J150847.59+571501.1 | 15 08 47.59 | +57 15 01.14 | 4.88 | Pâris et al. (2017) |
| SDSS J150851.23+042140.5 | 15 08 51.24 | +04 21 40.54 | 4.01 | Schneider et al. (2005) |
| SDSS J150903.53+274309.1 | 15 09 03.54 | +27 43 09.19 | 4.06 | Schneider et al. (2010) |
| SDSS J150916.99+042530.0 | 15 09 17.00 | +04 25 30.02 | 4.15 | Pâris et al. (2017) |
| SDSS J150935.63+105128.7 | 15 09 35.63 | +10 51 28.71 | 4.01 | Pâris et al. (2017) |
| SDSS J150949.82+504917.4 | 15 09 49.82 | +50 49 17.41 | 4.03 | Schneider et al. (2005) |

| | | | | |
|---|---|---|---|---|
| SDSS J151035.29+514841.0 | 15 10 35.29 | +51 48 41.10 | 5.06 | Pâris et al. (2017) |
| SDSS J151041.79+031810.6 | 15 10 41.79 | +03 18 10.61 | 4.27 | Schneider et al. (2005) |
| SDSS J151145.15+421326.0 | 15 11 45.16 | +42 13 26.10 | 4.12 | Pâris et al. (2017) |
| SDSS J151155.35+495723.8 | 15 11 55.35 | +49 57 23.84 | 4.46 | Pâris et al. (2017) |
| SDSS J151155.98+040802.9 | 15 11 55.98 | +04 08 03.00 | 4.65 | Schneider et al. (2005) |
| SDSS J151254.37−005636.5 | 15 12 54.37 | −00 56 36.60 | 4.47 | Pâris et al. (2017) |
| SDSS J151314.62+291906.3 | 15 13 14.62 | +29 19 06.36 | 4.23 | Pâris et al. (2012) |
| SDSS J151317.55+424557.2 | 15 13 17.55 | +42 45 57.25 | 4.09 | Schneider et al. (2007) |
| SDSS J151317.89+154141.8 | 15 13 17.90 | +15 41 41.81 | 4.27 | Pâris et al. (2014) |
| SDSS J151320.89+105807.3 | 15 13 20.90 | +10 58 07.34 | 4.62 | Schneider et al. (2010) |
| SDSS J151325.37+282430.6 | 15 13 25.37 | +28 24 30.63 | 4.00 | Pâris et al. (2012) |
| J151339.64+085406.5 | 15 13 39.64 | +08 54 06.50 | 5.47 | Yang et al. (2017) |
| SDSS J151404.78+473815.8 | 15 14 04.78 | +47 38 15.82 | 4.66 | Schneider et al. (2005) |
| PSO J228.6871+21.2388 | 15 14 44.91 | +21 14 19.78 | 5.92 | Bañados et al. (2016) |
| SDSS J151540.89+115534.4 | 15 15 40.90 | +11 55 34.47 | 4.03 | Schneider et al. (2010) |
| SDSS J151542.68+404311.1 | 15 15 42.68 | +40 43 11.17 | 4.53 | Schneider et al. (2005) |
| SDSS J151601.00+134545.0 | 15 16 01.01 | +13 45 45.08 | 4.62 | Schneider et al. (2010) |
| SDSS J151602.33+443233.5 | 15 16 02.33 | +44 32 33.52 | 4.10 | Schneider et al. (2005) |
| SDSS J151700.56+243814.0 | 15 17 00.57 | +24 38 14.01 | 4.40 | Schneider et al. (2010) |
| SDSS J151701.92+155224.6 | 15 17 01.92 | +15 52 24.65 | 4.03 | Pâris et al. (2014) |
| SDSS J151719.08+490003.3 | 15 17 19.09 | +49 00 03.32 | 4.67 | Pâris et al. (2017) |
| SDSS J151848.25+253930.2 | 15 18 48.26 | +25 39 30.22 | 4.23 | Schneider et al. (2010) |
| SDSS J151848.99+385922.9 | 15 18 49.00 | +38 59 22.99 | 4.23 | Pâris et al. (2014) |
| J151901.27+042348.60 | 15 19 01.27 | +04 23 48.60 | 4.94 | Wang et al. (2016) |
| SDSS J151909.09+030633.8 | 15 19 09.09 | +03 06 33.82 | 4.41 | Schneider et al. (2005) |
| PS1 J151911.32−065042.97 | 15 19 11.32 | −06 50 42.97 | 4.95 | Yang et al. (2018) |
| SDSS J151929.10+022812.1 | 15 19 29.11 | +02 28 12.11 | 4.48 | Pâris et al. (2017) |
| SDSS J152005.92+233952.9 | 15 20 05.93 | +23 39 52.96 | 4.49 | Schneider et al. (2010) |
| SDSS J152030.16+224641.1 | 15 20 30.17 | +22 46 41.15 | 4.08 | Pâris et al. (2012) |
| SDSS J152037.56+381247.3 | 15 20 37.57 | +38 12 47.38 | 4.02 | Pâris et al. (2017) |
| SDSS J152120.48+135348.1 | 15 21 20.48 | +13 53 48.11 | 4.07 | Pâris et al. (2014) |
| SDSS J152132.89+003252.2 | 15 21 32.89 | +00 32 52.26 | 4.55 | Pâris et al. (2012) |
| SDSS J152140.36+593738.5 | 15 21 40.37 | +59 37 38.59 | 4.14 | Pâris et al. (2017) |
| SDSS J152209.65+454625.7 | 15 22 09.66 | +45 46 25.71 | 4.33 | Schneider et al. (2005) |
| SDSS J152238.94+464306.8 | 15 22 38.94 | +46 43 06.86 | 4.42 | Pâris et al. (2017) |
| SDSS J152241.26+410740.4 | 15 22 41.26 | +41 07 40.41 | 4.07 | Pâris et al. (2017) |
| SDSS J152244.34−003412.9 | 15 22 44.35 | −00 34 12.95 | 4.75 | Pâris et al. (2017) |
| SDSS J152245.19+024543.8 | 15 22 45.19 | +02 45 43.85 | 4.09 | Schneider et al. (2005) |
| SDSS J152254.35+023035.9 | 15 22 54.36 | +02 30 35.95 | 4.13 | Pâris et al. (2017) |
| J152302.90+591633.04 | 15 23 02.90 | +59 16 33.04 | 5.11 | Wang et al. (2016) |
| SDSS J152345.70+334759.8 | 15 23 45.70 | +33 47 59.84 | 5.33 | Pâris et al. (2012) |
| SDSS J152347.89+315527.2 | 15 23 47.89 | +31 55 27.25 | 4.54 | Schneider et al. (2007) |
| SDSS J152400.30+015237.0 | 15 24 00.31 | +01 52 37.01 | 4.02 | Pâris et al. (2017) |
| SDSS J15240+0816 | 15 24 04.13 | +08 16 39.00 | 5.08 | Chiu et al. (2005) |
| SDSS J152404.23+134417.5 | 15 24 04.23 | +13 44 17.54 | 4.79 | Schneider et al. (2010) |
| SDSS J152443.18+011358.8 | 15 24 43.18 | +01 13 58.88 | 4.12 | Schneider et al. (2005) |
| SDSS J152446.76+162208.7 | 15 24 46.76 | +16 22 08.74 | 4.46 | Pâris et al. (2017) |
| SDSS J152509.79−001418.3 | 15 25 09.79 | −00 14 18.32 | 4.33 | Pâris et al. (2012) |
| SDSS J152512.45+432847.8 | 15 25 12.46 | +43 28 47.89 | 4.14 | Pâris et al. (2017) |
| SDSS J152542.62+211810.6 | 15 25 42.63 | +21 18 10.69 | 4.17 | Pâris et al. (2012) |
| SDSS J152544.87+592526.4 | 15 25 44.87 | +59 25 26.40 | 4.06 | Pâris et al. (2017) |
| SDSS J152617.91+053554.1 | 15 26 17.91 | +05 35 54.11 | 4.24 | Schneider et al. (2010) |
| SDSS J152623.22−005725.0 | 15 26 23.23 | −00 57 25.05 | 4.29 | Pâris et al. (2012) |
| SDSS J152638.12+061402.5 | 15 26 38.12 | +06 14 02.52 | 4.65 | Schneider et al. (2010) |
| SDSS J152642.67+245047.4 | 15 26 42.68 | +24 50 47.48 | 4.23 | Pâris et al. (2012) |
| SDSS J152649.81+585811.2 | 15 26 49.81 | +58 58 11.29 | 4.37 | Pâris et al. (2017) |
| SDSS J152656.82+251011.1 | 15 26 56.82 | +25 10 11.14 | 4.10 | Pâris et al. (2012) |

| | | | | |
|---|---|---|---|---|
| SDSS J152707.77+415405.3 | 15 27 07.78 | +41 54 05.40 | 4.58 | Pâris et al. (2017) |
| J152712.86+064121.9 | 15 27 12.86 | +06 41 21.90 | 5.57 | Yang et al. (2017) |
| SDSS J152740.52−010602.7 | 15 27 40.52 | −01 06 02.75 | 4.43 | Schneider et al. (2005) |
| SDSS J152743.86+035301.4 | 15 27 43.86 | +03 53 01.41 | 4.23 | Pâris et al. (2017) |
| SDSS J152812.08+224753.9 | 15 28 12.08 | +22 47 53.93 | 4.20 | Pâris et al. (2017) |
| SDSS J152821.38+591047.2 | 15 28 21.39 | +59 10 47.21 | 4.34 | Pâris et al. (2017) |
| SDSS J152831.26+285052.1 | 15 28 31.27 | +28 50 52.16 | 4.21 | Pâris et al. (2012) |
| SDSS J152838.81+381855.5 | 15 28 38.82 | +38 18 55.54 | 4.06 | Schneider et al. (2005) |
| SDSS J152854.65+024840.6 | 15 28 54.65 | +02 48 40.64 | 4.15 | Pâris et al. (2012) |
| SDSS J152908.59+023013.6 | 15 29 08.59 | +02 30 13.65 | 4.42 | Schneider et al. (2010) |
| SDSS J152918.29+154552.7 | 15 29 18.29 | +15 45 52.72 | 4.03 | Pâris et al. (2012) |
| SDSS J153010.81+202027.4 | 15 30 10.82 | +20 20 27.44 | 4.59 | Pâris et al. (2012) |
| SDSS J153024.82+241913.0 | 15 30 24.82 | +24 19 13.02 | 4.71 | Schneider et al. (2010) |
| SDSS J153112.85+561004.8 | 15 31 12.85 | +56 10 04.85 | 4.01 | Schneider et al. (2010) |
| PSS J1531+4517 | 15 31 29.92 | +45 17 07.75 | 4.19 | Djorgovski et al. (2001) |
| SDSS J153224.27+291215.1 | 15 32 24.27 | +29 12 15.17 | 4.20 | Schneider et al. (2010) |
| SDSS J153229.11+160949.7 | 15 32 29.11 | +16 09 49.77 | 4.80 | Pâris et al. (2012) |
| SDSS J153236.78+275154.8 | 15 32 36.78 | +27 51 54.82 | 4.17 | Pâris et al. (2012) |
| SDSS J153247.42+223704.1 | 15 32 47.42 | +22 37 04.18 | 4.44 | Pâris et al. (2017) |
| SDSS J153259.73+001440.2 | 15 32 59.74 | +00 14 40.30 | 4.14 | Pâris et al. (2017) |
| SDSSp J153259.96−003944.1 | 15 32 59.96 | −00 39 44.10 | 4.62 | Fan et al. (2000a) |
| SDSS J153308.65+301820.7 | 15 33 08.66 | +30 18 20.76 | 4.44 | Schneider et al. (2007) |
| SDSS J153321.12+082448.3 | 15 33 21.12 | +08 24 48.37 | 4.03 | Schneider et al. (2010) |
| SDSS J153422.74+571140.5 | 15 34 22.75 | +57 11 40.50 | 4.82 | Schneider et al. (2005) |
| SDSS J153424.03+165423.2 | 15 34 24.04 | +16 54 23.26 | 4.12 | Schneider et al. (2010) |
| SDSS J153459.75+132701.4 | 15 34 59.76 | +13 27 01.42 | 5.04 | Pâris et al. (2017) |
| SDSS J153505.37+163514.5 | 15 35 05.38 | +16 35 14.59 | 4.23 | Pâris et al. (2017) |
| DELS J153532.87+194320.1 | 15 35 32.87 | +19 43 20.10 | 6.40 | Wang et al. (2018) |
| SDSS J153539.16+335830.8 | 15 35 39.16 | +33 58 30.82 | 4.21 | Pâris et al. (2017) |
| SDSS J153607.23+344434.2 | 15 36 07.23 | +34 44 34.25 | 4.14 | Pâris et al. (2014) |
| SDSS J153627.09+143717.1 | 15 36 27.09 | +14 37 17.15 | 4.88 | Schneider et al. (2010) |
| SDSS J153650.25+500810.3 | 15 36 50.26 | +50 08 10.33 | 4.93 | Schneider et al. (2005) |
| SDSS J153711.60+230727.1 | 15 37 11.61 | +23 07 27.18 | 4.33 | Pâris et al. (2012) |
| SDSS J153715.42+072128.7 | 15 37 15.43 | +07 21 28.71 | 4.71 | Pâris et al. (2017) |
| SDSS J153743.81+161714.8 | 15 37 43.82 | +16 17 14.83 | 4.43 | Pâris et al. (2017) |
| SDSS J153801.08+122128.1 | 15 38 01.08 | +12 21 28.17 | 4.02 | Pâris et al. (2012) |
| SDSS J153812.30+361818.6 | 15 38 12.31 | +36 18 18.64 | 4.27 | Pâris et al. (2014) |
| SDSS J153820.84+143646.5 | 15 38 20.85 | +14 36 46.53 | 4.43 | Schneider et al. (2010) |
| J1538+5032 | 15 39 34.52 | +50 32 08.90 | 4.96 | Polsterer, Zinn, & Gieseke (2013) |
| SDSS J153941.58+095807.1 | 15 39 41.58 | +09 58 07.14 | 4.13 | Schneider et al. (2010) |
| SDSS J153957.62+182032.2 | 15 39 57.63 | +18 20 32.27 | 4.02 | Pâris et al. (2012) |
| SDSS J154055.70+153700.5 | 15 40 55.70 | +15 37 00.55 | 4.46 | Pâris et al. (2012) |
| SDSS J154104.66+360252.9 | 15 41 04.67 | +36 02 52.93 | 4.30 | Bovy et al. (2011) |
| SDSS J154135.77+121923.3 | 15 41 35.78 | +12 19 23.32 | 4.29 | Pâris et al. (2012) |
| SDSS J154215.20+012849.2 | 15 42 15.20 | +01 28 49.27 | 4.06 | Pâris et al. (2012) |
| SDSS J154254.06+072641.1 | 15 42 54.06 | +07 26 41.18 | 4.17 | Pâris et al. (2012) |
| SDSS J154254.66+052559.6 | 15 42 54.66 | +05 25 59.61 | 4.32 | Pâris et al. (2017) |
| SDSS J154324.58+490254.9 | 15 43 24.58 | +49 02 54.95 | 4.09 | Pâris et al. (2017) |
| SDSS J154328.13+192934.4 | 15 43 28.13 | +19 29 34.43 | 4.26 | Pâris et al. (2012) |
| SDSS J154331.51+491128.8 | 15 43 31.52 | +49 11 28.85 | 4.47 | Pâris et al. (2017) |
| SDSS J154339.63+233758.1 | 15 43 39.63 | +23 37 58.12 | 4.07 | Pâris et al. (2012) |
| PSS J1543+3417 | 15 43 40.38 | +34 17 44.46 | 4.42 | Djorgovski et al. (2001) |
| PSO J235.9450+17.0079 | 15 43 46.82 | +17 00 28.46 | 5.82 | Bañados et al. (2016) |
| SDSS J154352.92+333759.5 | 15 43 52.93 | +33 37 59.56 | 4.58 | Schneider et al. (2007) |
| SDSS J154424.26+140922.5 | 15 44 24.26 | +14 09 22.53 | 4.75 | Pâris et al. (2012) |
| J1545+4232 | 15 45 05.62 | +42 32 11.60 | 6.50 | Chehade et al. (2018) |
| SDSS J154508.25+242846.1 | 15 45 08.26 | +24 28 46.15 | 4.53 | Pâris et al. (2012) |

| | | | | |
|---|---|---|---|---|
| PSO J236.2912+16.6088 | 15 45 09.90 | +16 36 31.91 | 5.82 | Bañados et al. (2016) |
| SDSS J1545+6028 | 15 45 52.09 | +60 28 23.95 | 5.78 | Wang et al. (2016) |
| SDSS J154559.64+401506.7 | 15 45 59.64 | +40 15 06.74 | 4.10 | Pâris et al. (2017) |
| SDSS J154606.79+465614.5 | 15 46 06.79 | +46 56 14.57 | 4.17 | Pâris et al. (2017) |
| SDSS J154612.86+082109.2 | 15 46 12.86 | +08 21 09.26 | 4.23 | Pâris et al. (2017) |
| SDSS J154629.70+191435.7 | 15 46 29.71 | +19 14 35.74 | 4.02 | Pâris et al. (2012) |
| SDSS J154633.95+360343.7 | 15 46 33.95 | +36 03 43.75 | 4.11 | Schneider et al. (2007) |
| SDSS J154633.96+315358.4 | 15 46 33.96 | +31 53 58.43 | 4.07 | Pâris et al. (2012) |
| SDSS J154650.26+374331.4 | 15 46 50.27 | +37 43 31.40 | 4.09 | Pâris et al. (2014) |
| SDSS J154729.78+035416.4 | 15 47 29.79 | +03 54 16.48 | 4.04 | Schneider et al. (2010) |
| SDSS J154730.09+064709.7 | 15 47 30.09 | +06 47 09.79 | 4.34 | Pâris et al. (2012) |
| SDSS J154734.94+444652.4 | 15 47 34.95 | +44 46 52.46 | 4.57 | Pâris et al. (2017) |
| SDSS J154739.64+483319.5 | 15 47 39.65 | +48 33 19.60 | 4.31 | Pâris et al. (2017) |
| SDSS J154814.20+202908.6 | 15 48 14.21 | +20 29 08.60 | 4.72 | Pâris et al. (2017) |
| SDSS J154837.08+323151.1 | 15 48 37.09 | +32 31 51.13 | 4.25 | Pâris et al. (2012) |
| SDSS J154841.76+352142.0 | 15 48 41.76 | +35 21 42.01 | 4.94 | Schneider et al. (2007) |
| SDSS J154900.17+263233.4 | 15 49 00.17 | +26 32 33.46 | 4.09 | Pâris et al. (2012) |
| SDSS J154912.59+282002.1 | 15 49 12.60 | +28 20 02.17 | 4.38 | Pâris et al. (2012) |
| J1550+4318 | 15 50 00.93 | +43 18 02.80 | 5.84 | Chehade et al. (2018) |
| SDSS J155017.30+111213.7 | 15 50 17.31 | +11 12 13.74 | 4.20 | Pâris et al. (2014) |
| SDSS J155022.18+391839.2 | 15 50 22.19 | +39 18 39.23 | 4.38 | Pâris et al. (2014) |
| SDSS J155051.20+110418.9 | 15 50 51.20 | +11 04 18.94 | 4.55 | Schneider et al. (2010) |
| SDSS J155103.40+165324.5 | 15 51 03.41 | +16 53 24.56 | 4.68 | Pâris et al. (2012) |
| SDSS J155119.50+513358.5 | 15 51 19.50 | +51 33 58.57 | 4.07 | Pâris et al. (2017) |
| SDSS J155144.28+111614.3 | 15 51 44.28 | +11 16 14.38 | 4.31 | Pâris et al. (2014) |
| SDSS J155201.68+043933.0 | 15 52 01.68 | +04 39 33.00 | 4.09 | Schneider et al. (2010) |
| SDSS J155243.04+255229.2 | 15 52 43.04 | +25 52 29.23 | 4.67 | Schneider et al. (2007) |
| SDSS J155247.93+210054.8 | 15 52 47.93 | +21 00 54.89 | 4.26 | Pâris et al. (2017) |
| SDSS J155255.38+145432.9 | 15 52 55.39 | +14 54 32.95 | 4.10 | Schneider et al. (2010) |
| SDSS J155319.11+325957.4 | 15 53 19.11 | +32 59 57.43 | 4.79 | Schneider et al. (2005) |
| SDSS J155338.07+392218.0 | 15 53 38.08 | +39 22 18.05 | 4.65 | Schneider et al. (2005) |
| SDSS J155343.11+500257.4 | 15 53 43.11 | +50 02 57.48 | 4.28 | Pâris et al. (2017) |
| SDSS J155405.25+204049.5 | 15 54 05.26 | +20 40 49.52 | 4.14 | Schneider et al. (2010) |
| SDSS J15543+3032 | 15 54 23.00 | +30 32 14.00 | 4.84 | Chiu et al. (2005) |
| SDSS J155426.15+193703.0 | 15 54 26.16 | +19 37 03.04 | 4.61 | Schneider et al. (2010) |
| SDSS J155437.34+210057.0 | 15 54 37.34 | +21 00 57.09 | 4.10 | Pâris et al. (2012) |
| SDSS J155442.53+045520.6 | 15 54 42.53 | +04 55 20.61 | 4.03 | Pâris et al. (2017) |
| SDSS J155452.51+185920.0 | 15 54 52.51 | +18 59 20.09 | 4.07 | Schneider et al. (2010) |
| PSS J1555+2003 | 15 55 02.55 | +20 03 25.11 | 4.21 | Djorgovski et al. (2001) |
| SDSS J155617.67+071044.1 | 15 56 17.67 | +07 10 44.11 | 4.07 | Pâris et al. (2012) |
| SDSS J155631.73+205701.9 | 15 56 31.74 | +20 57 01.91 | 4.46 | Pâris et al. (2017) |
| SDSS J155639.52+312739.9 | 15 56 39.53 | +31 27 39.94 | 4.00 | Schneider et al. (2005) |
| SDSS J155653.70+613249.3 | 15 56 53.70 | +61 32 49.32 | 4.18 | Pâris et al. (2017) |
| SDSS J155700.16+101841.7 | 15 57 00.17 | +10 18 41.77 | 4.83 | Schneider et al. (2010) |
| SDSS J155726.74+242116.1 | 15 57 26.75 | +24 21 16.16 | 4.69 | Pâris et al. (2017) |
| SDSS J155735.42+273004.6 | 15 57 35.43 | +27 30 04.62 | 4.04 | Pâris et al. (2017) |
| SDSS J155738.40+232057.4 | 15 57 38.40 | +23 20 57.43 | 4.12 | Pâris et al. (2017) |
| SDSS J155759.32+220823.1 | 15 57 59.33 | +22 08 23.17 | 4.01 | Pâris et al. (2017) |
| SDSS J155813.84+313101.4 | 15 58 13.84 | +31 31 01.40 | 4.17 | Pâris et al. (2017) |
| DELS J155909.09+221214.4 | 15 59 09.09 | +22 12 14.40 | 6.07 | Wang et al. (2017) |
| SDSS J155909.32+561840.8 | 15 59 09.32 | +56 18 40.90 | 4.09 | Pâris et al. (2017) |
| SDSS J160023.14+182706.8 | 16 00 23.14 | +18 27 06.83 | 4.10 | Pâris et al. (2012) |
| SDSS J160031.73+210251.1 | 16 00 31.73 | +21 02 51.19 | 4.40 | Pâris et al. (2017) |
| SDSS J160120.10+374948.8 | 16 01 20.11 | +37 49 48.85 | 4.40 | Schneider et al. (2005) |
| SDSS J160205.30+374605.5 | 16 02 05.31 | +37 46 05.59 | 4.42 | Schneider et al. (2005) |
| SDSS J160207.96+523717.9 | 16 02 07.96 | +52 37 17.91 | 4.91 | Schneider et al. (2005) |
| SDSS J1602+4228 | 16 02 53.98 | +42 28 24.94 | 6.09 | Fan et al. (2004) |

| | | | | |
|---|---|---|---|---|
| BR J1603+0721 | 16 03 20.89 | +07 21 04.51 | 4.42 | Storrie-Lombardi et al. (2001) |
| SDSS J160326.03+121726.5 | 16 03 26.03 | +12 17 26.53 | 4.07 | Schneider et al. (2010) |
| SDSS J160329.14+090218.3 | 16 03 29.14 | +09 02 18.31 | 4.73 | Schneider et al. (2007) |
| SDSS J160336.65+350824.3 | 16 03 36.65 | +35 08 24.31 | 4.46 | Schneider et al. (2007) |
| ELAIS1091000446 | 16 03 49.07 | +55 10 32.30 | 6.04 | Kashikawa et al. (2015) |
| SDSS J160351.84+345517.4 | 16 03 51.84 | +34 55 17.46 | 4.61 | Schneider et al. (2007) |
| SDSS J160354.70+155317.1 | 16 03 54.70 | +15 53 17.18 | 4.06 | Pâris et al. (2012) |
| SDSS J160420.32+504737.0 | 16 04 20.33 | +50 47 37.02 | 4.66 | Schneider et al. (2005) |
| SDSS J160447.18+241431.4 | 16 04 47.18 | +24 14 31.43 | 4.02 | Pâris et al. (2012) |
| SDSS J160501.20−011220.6 | 16 05 01.21 | −01 12 20.69 | 4.92 | Schneider et al. (2005) |
| SDSS J160516.16+210638.5 | 16 05 16.16 | +21 06 38.55 | 4.49 | Schneider et al. (2010) |
| SDSS J160523.49+080849.8 | 16 05 23.49 | +08 08 49.84 | 4.25 | Pâris et al. (2012) |
| SDSS J160641.00+291919.2 | 16 06 41.00 | +29 19 19.29 | 4.15 | Schneider et al. (2007) |
| SDSS J160651.01+085037.5 | 16 06 51.01 | +08 50 37.52 | 4.54 | Pâris et al. (2017) |
| SDSS J160730.00+281336.9 | 16 07 30.01 | +28 13 36.93 | 4.01 | Pâris et al. (2012) |
| SDSS J160734.22+160417.4 | 16 07 34.23 | +16 04 17.44 | 4.76 | Schneider et al. (2010) |
| SDSS J160759.73+315537.6 | 16 07 59.74 | +31 55 37.65 | 4.20 | Schneider et al. (2007) |
| SDSS J160828.42+104228.2 | 16 08 28.43 | +10 42 28.22 | 4.06 | Schneider et al. (2010) |
| SDSS J160829.81+212321.6 | 16 08 29.82 | +21 23 21.61 | 4.16 | Pâris et al. (2012) |
| SDSS J160906.58+364717.1 | 16 09 06.59 | +36 47 17.14 | 4.23 | Pâris et al. (2012) |
| SDSS J160911.30+320555.2 | 16 09 11.30 | +32 05 55.22 | 4.03 | Pâris et al. (2017) |
| ULAS J1609+3041 | 16 09 37.27 | +30 41 47.78 | 6.16 | Jiang et al. (2016) |
| SDSS J160941.79+425157.9 | 16 09 41.79 | +42 51 57.93 | 4.11 | Pâris et al. (2017) |
| SDSS J160953.77+474544.2 | 16 09 53.77 | +47 45 44.25 | 4.26 | Pâris et al. (2017) |
| SDSS J161001.03+305402.7 | 16 10 01.04 | +30 54 02.70 | 4.06 | Schneider et al. (2005) |
| SDSS J161016.71+411753.7 | 16 10 16.72 | +41 17 53.78 | 5.01 | Pâris et al. (2014) |
| SDSS J161119.57+441144.0 | 16 11 19.57 | +44 11 44.03 | 4.01 | Schneider et al. (2005) |
| SDSS J161121.27+190522.0 | 16 11 21.27 | +19 05 22.03 | 4.03 | Schneider et al. (2010) |
| SDSS J161151.60+404740.8 | 16 11 51.60 | +40 47 40.82 | 4.87 | Pâris et al. (2014) |
| Q J1612+5255 | 16 12 53.07 | +52 55 44.00 | 4.95 | Sharp et al. (2001) |
| SDSS J161317.33+185340.3 | 16 13 17.34 | +18 53 40.39 | 4.39 | Pâris et al. (2017) |
| SDSS J161333.49+195333.8 | 16 13 33.50 | +19 53 33.83 | 4.26 | Pâris et al. (2012) |
| SDSS J161335.16+114212.0 | 16 13 35.16 | +11 42 12.05 | 4.02 | Pâris et al. (2014) |
| SDSS J161447.03+205902.9 | 16 14 47.04 | +20 59 02.97 | 5.09 | Schneider et al. (2010) |
| SDSS J161451.02+233929.9 | 16 14 51.03 | +23 39 29.95 | 4.39 | Pâris et al. (2012) |
| PSS J1615+1803 | 16 15 22.86 | +18 03 56.32 | 4.01 | Djorgovski et al. (2001) |
| SDSS J161538.11+430301.2 | 16 15 38.12 | +43 03 01.21 | 4.10 | Schneider et al. (2005) |
| SDSSp J161544.14+010401.9 | 16 15 44.14 | +01 04 01.90 | 4.01 | Schneider et al. (2001) |
| SDSS J161559.52+233203.9 | 16 15 59.53 | +23 32 03.98 | 4.12 | Schneider et al. (2007) |
| SDSS J161616.26+513336.9 | 16 16 16.27 | +51 33 36.95 | 4.53 | Schneider et al. (2005) |
| SDSS J161618.08+122351.5 | 16 16 18.08 | +12 23 51.52 | 4.29 | Schneider et al. (2010) |
| SDSS J161622.10+050127.7 | 16 16 22.11 | +05 01 27.75 | 4.87 | Schneider et al. (2010) |
| SDSS J161626.65+122625.6 | 16 16 26.65 | +12 26 25.62 | 4.30 | Schneider et al. (2010) |
| SDSS J161629.55+254511.6 | 16 16 29.56 | +25 45 11.63 | 4.03 | Pâris et al. (2017) |
| SDSS J161701.17+163615.7 | 16 17 01.17 | +16 36 15.70 | 4.47 | Schneider et al. (2010) |
| SDSS J161723.33+160905.4 | 16 17 23.33 | +16 09 05.46 | 4.05 | Pâris et al. (2012) |
| SDSS J161822.66+333748.3 | 16 18 22.67 | +33 37 48.32 | 4.44 | Schneider et al. (2007) |
| PSS J1618+4125 | 16 18 22.76 | +41 25 58.31 | 4.22 | Constantin et al. (2002) |
| SDSS J161845.26+455257.5 | 16 18 45.26 | +45 52 57.53 | 4.70 | Schneider et al. (2005) |
| SDSS J161859.06+263000.3 | 16 18 59.06 | +26 30 00.34 | 4.55 | Schneider et al. (2007) |
| SDSS J161916.80+204101.7 | 16 19 16.81 | +20 41 01.78 | 4.03 | Pâris et al. (2012) |
| SDSS J161931.58+123844.4 | 16 19 31.59 | +12 38 44.50 | 4.77 | Schneider et al. (2010) |
| SDSS J161936.67+164804.6 | 16 19 36.67 | +16 48 04.63 | 4.33 | Schneider et al. (2010) |
| SDSS J162007.15+374721.7 | 16 20 07.16 | +37 47 21.77 | 4.44 | Pâris et al. (2014) |
| SDSS J162027.87+300003.5 | 16 20 27.88 | +30 00 03.52 | 4.15 | Pâris et al. (2012) |
| J162045.64+520246.65 | 16 20 45.64 | +52 02 46.65 | 4.79 | Wang et al. (2016) |
| SDSS J162049.07+512527.3 | 16 20 49.08 | +51 25 27.31 | 4.03 | Pâris et al. (2017) |

| | | | | |
|---|---|---|---|---|
| SDSS J162052.58+260136.7 | 16 20 52.58 | +26 01 36.76 | 4.02 | Pâris et al. (2012) |
| SDSS J162100.70+515544.8 | 16 21 00.70 | +51 55 44.80 | 5.71 | Wang et al. (2008) |
| SDSS J162159.10+311005.7 | 16 21 59.10 | +31 10 05.75 | 4.61 | Schneider et al. (2007) |
| SDSS J162246.91+390220.8 | 16 22 46.91 | +39 02 20.84 | 4.03 | Pâris et al. (2014) |
| SDSS J162257.91+220524.9 | 16 22 57.92 | +22 05 24.93 | 4.04 | Pâris et al. (2012) |
| J162315.28+470559.90 | 16 23 15.28 | +47 05 59.90 | 5.13 | Wang et al. (2016) |
| SDSS J162321.15+282814.2 | 16 23 21.16 | +28 28 14.26 | 4.22 | Schneider et al. (2007) |
| SDSS J162331.80+311200.5 | 16 23 31.93 | +31 12 01.00 | 6.22 | Fan et al. (2004) |
| SDSS J162445.03+271418.7 | 16 24 45.04 | +27 14 18.79 | 4.50 | Schneider et al. (2005) |
| SDSS J162502.77+305210.0 | 16 25 02.78 | +30 52 10.07 | 4.33 | Pâris et al. (2012) |
| SDSS J162509.67+312714.2 | 16 25 09.68 | +31 27 14.24 | 4.10 | Pâris et al. (2012) |
| SDSS J162522.37+123320.0 | 16 25 22.37 | +12 33 20.02 | 4.42 | Schneider et al. (2010) |
| SDSS J162539.84+251558.8 | 16 25 39.85 | +25 15 58.82 | 4.15 | Schneider et al. (2007) |
| SDSS J162542.13+310459.2 | 16 25 42.14 | +31 04 59.28 | 4.08 | Schneider et al. (2007) |
| SDSS J162623.38+484136.4 | 16 26 23.38 | +48 41 36.47 | 4.84 | Schneider et al. (2005) |
| SDSS J162626.50+275132.4 | 16 26 26.50 | +27 51 32.50 | 5.16 | Pâris et al. (2017) |
| SDSS J162629.19+285857.5 | 16 26 29.20 | +28 58 57.58 | 5.00 | Pâris et al. (2017) |
| SDSS J162704.10+374509.0 | 16 27 04.10 | +37 45 09.06 | 4.27 | Pâris et al. (2014) |
| SDSS J162716.69+555337.0 | 16 27 16.69 | +55 53 37.05 | 4.07 | Pâris et al. (2017) |
| QPQ6 J162737.24+460609.3 | 16 27 37.24 | +46 06 09.30 | 4.11 | Prochaska et al. (2013) |
| SDSS J162754.76+211631.9 | 16 27 54.76 | +21 16 31.95 | 4.10 | Schneider et al. (2007) |
| SDSS J162825.26+461631.1 | 16 28 25.27 | +46 16 31.16 | 4.00 | Pâris et al. (2017) |
| J162838.83+063859.14 | 16 28 38.83 | +06 38 59.14 | 4.85 | Wang et al. (2016) |
| SDSS J162840.62+204546.1 | 16 28 40.63 | +20 45 46.11 | 4.47 | Schneider et al. (2007) |
| SDSS J162844.07+200039.7 | 16 28 44.07 | +20 00 39.72 | 4.25 | Schneider et al. (2010) |
| SDSS J162852.19+174013.4 | 16 28 52.19 | +17 40 13.41 | 4.00 | Pâris et al. (2012) |
| PSO J247.2970+24.1277 | 16 29 11.29 | +24 07 39.60 | 6.48 | Mazzucchelli et al. (2017) |
| SDSS J162916.16+333714.5 | 16 29 16.17 | +33 37 14.58 | 4.41 | Schneider et al. (2005) |
| SDSS J163009.32+280421.5 | 16 30 09.33 | +28 04 21.53 | 4.06 | Schneider et al. (2007) |
| SDSS J163016.99+193954.3 | 16 30 16.99 | +19 39 54.39 | 4.15 | Schneider et al. (2010) |
| SDSS J16305+4012 | 16 30 33.93 | +40 12 10.00 | 6.05 | Fan et al. (2003) |
| SDSS J163059.03+450717.3 | 16 30 59.03 | +45 07 17.39 | 4.14 | Pâris et al. (2014) |
| SDSS J163112.11+351845.4 | 16 31 12.11 | +35 18 45.42 | 4.12 | Schneider et al. (2005) |
| SDSS J163114.44+315513.2 | 16 31 14.45 | +31 55 13.27 | 4.05 | Pâris et al. (2017) |
| SDSS J163213.31+333733.1 | 16 32 13.32 | +33 37 33.14 | 4.16 | Pâris et al. (2014) |
| SDSS J163257.06+441110.2 | 16 32 57.07 | +44 11 10.26 | 4.10 | Schneider et al. (2005) |
| PSS J1633+1411 | 16 33 19.63 | +14 11 42.07 | 4.38 | Péroux et al. (2001) |
| SDSS J163332.87+314649.4 | 16 33 32.87 | +31 46 49.41 | 4.01 | Pâris et al. (2014) |
| SDSS J163411.81+215325.0 | 16 34 11.82 | +21 53 25.09 | 4.56 | Schneider et al. (2007) |
| SDSS J163423.72+282031.9 | 16 34 23.73 | +28 20 31.93 | 4.08 | Schneider et al. (2010) |
| SDSS J163506.33+181715.8 | 16 35 06.33 | +18 17 15.86 | 4.01 | Pâris et al. (2012) |
| SDSS J163628.67+480320.8 | 16 36 28.68 | +48 03 20.88 | 4.61 | Pâris et al. (2017) |
| SDSS J163636.92+315717.1 | 16 36 36.93 | +31 57 17.13 | 4.55 | Pâris et al. (2017) |
| SDSS J163647.19+382031.3 | 16 36 47.19 | +38 20 31.37 | 4.20 | Pâris et al. (2017) |
| SDSS J163655.17+322828.7 | 16 36 55.18 | +32 28 28.71 | 4.10 | Schneider et al. (2005) |
| SDSS J163701.76+132949.2 | 16 37 01.76 | +13 29 49.29 | 4.24 | Pâris et al. (2017) |
| SDSS J163710.74+443659.5 | 16 37 10.75 | +44 36 59.56 | 4.19 | Schneider et al. (2005) |
| SDSS J163804.10+365612.8 | 16 38 04.10 | +36 56 12.86 | 4.03 | Schneider et al. (2005) |
| J163810.39+150058.26 | 16 38 10.39 | +15 00 58.26 | 4.76 | Wang et al. (2016) |
| SDSS J164037.86+471917.0 | 16 40 37.87 | +47 19 17.05 | 4.71 | Pâris et al. (2017) |
| SDSS J164113.75+134158.8 | 16 41 13.76 | +13 41 58.90 | 4.11 | Pâris et al. (2017) |
| CFHQS J16413+3755 | 16 41 21.73 | +37 55 20.00 | 6.04 | Willott et al. (2007) |
| SDSS J164146.27+290148.6 | 16 41 46.27 | +29 01 48.60 | 4.15 | Schneider et al. (2007) |
| SDSS J164336.63+225207.4 | 16 43 36.63 | +22 52 07.48 | 4.09 | Pâris et al. (2017) |
| SDSS J164409.46+495856.3 | 16 44 09.46 | +49 58 56.33 | 4.33 | Pâris et al. (2017) |
| SDSS J164428.81+424201.6 | 16 44 28.81 | +42 42 01.62 | 4.06 | Schneider et al. (2005) |
| SDSS J164430.21+173545.3 | 16 44 30.21 | +17 35 45.32 | 4.24 | Pâris et al. (2012) |

| | | | | |
|---|---|---|---|---|
| SDSS J164640.07+241319.7 | 16 46 40.08 | +24 13 19.77 | 4.07 | Schneider et al. (2007) |
| SDSS J164655.38+311630.5 | 16 46 55.38 | +31 16 30.56 | 4.61 | Schneider et al. (2005) |
| PSS J1646+5514 | 16 46 56.40 | +55 14 46.00 | 4.04 | Péroux et al. (2001) |
| SDSS J164739.64+343608.6 | 16 47 39.65 | +34 36 08.64 | 4.02 | Schneider et al. (2005) |
| SDSS J164829.70+350158.9 | 16 48 29.71 | +35 01 58.88 | 4.08 | Newman et al. (2013) |
| SDSS J164934.13+334214.9 | 16 49 34.13 | +33 42 14.90 | 4.20 | Schneider et al. (2005) |
| SDSS J165051.24+311851.9 | 16 50 51.24 | +31 18 51.92 | 4.16 | Schneider et al. (2005) |
| SDSS J165202.23+383435.7 | 16 52 02.23 | +38 34 35.78 | 4.13 | Schneider et al. (2005) |
| SDSS J165248.64+174345.7 | 16 52 48.64 | +17 43 45.73 | 4.57 | Pâris et al. (2012) |
| SDSS J165354.61+405402.2 | 16 53 54.62 | +40 54 02.21 | 4.96 | Schneider et al. (2005) |
| SDSS J165412.23+254227.8 | 16 54 12.23 | +25 42 27.84 | 4.11 | Pâris et al. (2012) |
| SDSS J165436.85+222733.8 | 16 54 36.85 | +22 27 33.80 | 4.70 | Schneider et al. (2007) |
| J165635.46+454113.55 | 16 56 35.46 | +45 41 13.55 | 5.34 | Wang et al. (2016) |
| SDSS J165902.12+270935.1 | 16 59 02.12 | +27 09 35.19 | 5.31 | Schneider et al. (2007) |
| J165951.03+323928.63 | 16 59 51.03 | +32 39 28.63 | 5.17 | Wang et al. (2016) |
| SDSS J170033.94+190309.3 | 17 00 33.94 | +19 03 09.35 | 4.02 | Schneider et al. (2007) |
| SDSS J170248.55+314047.9 | 17 02 48.56 | +31 40 47.99 | 4.36 | Pâris et al. (2017) |
| SDSS J170254.22+243341.6 | 17 02 54.23 | +24 33 41.66 | 4.90 | Schneider et al. (2007) |
| CXO J17040+5147 | 17 04 03.40 | +51 47 58.00 | 4.27 | Eckart et al. (2006) |
| SDSS J170424.77+252236.6 | 17 04 24.78 | +25 22 36.65 | 4.69 | Schneider et al. (2007) |
| SDSS J170804.91+602201.9 | 17 08 04.91 | +60 22 02.00 | 4.40 | Schneider et al. (2005) |
| SDSS J170952.20+332905.9 | 17 09 52.21 | +33 29 05.96 | 4.24 | Schneider et al. (2005) |
| SDSS J171014.51+592326.4 | 17 10 14.52 | +59 23 26.46 | 4.49 | Schneider et al. (2005) |
| SDSS J171216.50+440742.7 | 17 12 16.51 | +44 07 42.76 | 4.07 | Pâris et al. (2017) |
| SDSS J171224.91+560624.9 | 17 12 24.91 | +56 06 24.92 | 4.22 | Schneider et al. (2005) |
| J171337.2+585306 | 17 13 37.20 | +58 53 06.00 | 4.37 | Khorunzhev et al. (2016) |
| SDSS J171437.67+272223.8 | 17 14 37.67 | +27 22 23.81 | 4.50 | Schneider et al. (2005) |
| SPIT J17149+5937 | 17 14 56.26 | +59 37 00.89 | 4.03 | Papovich et al. (2006) |
| SDSS J171509.96+294555.0 | 17 15 09.97 | +29 45 55.04 | 4.54 | Schneider et al. (2005) |
| PSS J1715+3809 | 17 15 39.47 | +38 09 10.00 | 4.52 | Prochaska, Castro, & Djorgovski (2003) |
| SDSS J171652.78+272005.4 | 17 16 52.79 | +27 20 05.47 | 4.13 | Pâris et al. (2017) |
| XFLS J17179+6009 | 17 17 54.60 | +60 09 14.00 | 4.27 | Lacy et al. (2007) |
| SDSS J171808.65+551511.1 | 17 18 08.66 | +55 15 11.15 | 4.62 | Schneider et al. (2005) |
| SDSS J171941.01+304918.7 | 17 19 41.02 | +30 49 18.76 | 4.19 | Schneider et al. (2010) |
| AMS16 | 17 19 42.13 | +58 47 09.00 | 4.17 | Martínez-Sansigre et al. (2006) |
| PSS J1721+3256 | 17 21 06.64 | +32 56 36.28 | 4.05 | Péroux et al. (2001) |
| SDSS J173744.87+582829.6 | 17 37 44.87 | +58 28 29.67 | 4.92 | Schneider et al. (2005) |
| HRQC J203957.78+004519.4 | 20 39 57.78 | +00 45 19.40 | 4.97 | McGreer et al. (2013) |
| J203958.0−004337 | 20 39 58.00 | −00 43 37.00 | 4.63 | Khorunzhev et al. (2016) |
| SDSS J204421.51−052521.8 | 20 44 21.51 | −05 25 21.84 | 4.33 | Schneider et al. (2005) |
| HRQC J204723.18−005021.9 | 20 47 23.18 | −00 50 21.90 | 4.89 | McGreer et al. (2013) |
| SDSS J204941.58−004051.3 | 20 49 41.59 | −00 40 51.32 | 4.19 | Schneider et al. (2005) |
| SDSS J205316.76+005920.9 | 20 53 16.77 | +00 59 20.97 | 4.30 | Schneider et al. (2005) |
| SDSS J20533+0047 | 20 53 21.80 | +00 47 07.00 | 5.92 | Jiang et al. (2009) |
| SDSS J20541−0005 | 20 54 06.40 | −00 05 14.00 | 6.06 | Jiang et al. (2008) |
| HRQC J205413.18+003503.0 | 20 54 13.18 | +00 35 03.00 | 4.86 | McGreer et al. (2013) |
| J205442.21+022952.02 | 20 54 42.21 | +02 29 52.02 | 4.56 | Wang et al. (2016) |
| SDSS J205509.48−071748.6 | 20 55 09.49 | −07 17 48.62 | 4.01 | Schneider et al. (2005) |
| SDSS J205724.14−003018.7 | 20 57 24.15 | −00 30 18.75 | 4.66 | Schneider et al. (2005) |
| SDSS J210155.44−062711.7 | 21 01 55.45 | −06 27 11.80 | 4.34 | Schneider et al. (2005) |
| SDSS J210216.52+104906.6 | 21 02 16.52 | +10 49 06.66 | 4.18 | Schneider et al. (2005) |
| PS1 J210759.13−032300.53 | 21 07 59.13 | −03 23 00.53 | 4.64 | Yang et al. (2018) |
| HRQC J211018.94+002208.8 | 21 10 18.94 | +00 22 08.80 | 4.66 | McGreer et al. (2013) |
| J211105.62−015604.14 | 21 11 05.62 | −01 56 04.14 | 4.85 | Wang et al. (2016) |
| HRQC J211158.01+005302.6 | 21 11 58.01 | +00 53 02.60 | 4.98 | McGreer et al. (2013) |
| HRQC J211225.39−000141.3 | 21 12 25.39 | −00 01 41.30 | 4.67 | McGreer et al. (2013) |
| HRQC J211435.27+001733.4 | 21 14 35.27 | +00 17 33.40 | 4.75 | McGreer et al. (2013) |

| | | | | |
|---|---|---|---|---|
| SDSS J211450.33−063257.0 | 21 14 50.34 | −06 32 57.09 | 4.24 | Schneider et al. (2005) |
| HRQC J211547.22+003123.8 | 21 15 47.22 | +00 31 23.80 | 4.84 | McGreer et al. (2013) |
| SDSS J211637.30+085302.3 | 21 16 37.30 | +08 53 02.38 | 4.03 | Pâris et al. (2012) |
| SDSS J211729.28−004810.8 | 21 17 29.28 | −00 48 10.90 | 4.04 | Pâris et al. (2012) |
| SDSS J21194+1029 | 21 19 28.33 | +10 29 07.00 | 5.18 | Chiu et al. (2005) |
| SDSS J211951.89−004020.1 | 21 19 51.89 | −00 40 20.14 | 5.87 | Jiang et al. (2016) |
| PSS J2122−0014 | 21 22 07.36 | −00 14 45.64 | 4.13 | Péroux et al. (2001) |
| SDSS J212336.02+005616.3 | 21 23 36.03 | +00 56 16.31 | 4.32 | Schneider et al. (2005) |
| SDSS J212426.45+063555.4 | 21 24 26.46 | +06 35 55.49 | 4.01 | Pâris et al. (2012) |
| SDSS J212744.12+005720.3 | 21 27 44.13 | +00 57 20.30 | 4.35 | Schneider et al. (2005) |
| SDSS J213008.94+002610.0 | 21 30 08.95 | +00 26 10.01 | 4.95 | Schneider et al. (2007) |
| SDSS J213112.19+043412.4 | 21 31 12.20 | +04 34 12.48 | 4.37 | Pâris et al. (2012) |
| SDSS J21324−0009 | 21 32 26.60 | −00 09 09.00 | 4.30 | Jiang et al. (2006) |
| PSS J2132+0106 | 21 32 43.26 | +01 06 33.86 | 4.03 | Abazajian et al. (2004) |
| SDSS J213429.47+003118.3 | 21 34 29.48 | +00 31 18.38 | 4.17 | Pâris et al. (2017) |
| PSS J2134+0817 | 21 34 43.20 | +08 17 29.00 | 4.00 | Djorgovski et al. (2001) |
| SDSS J213704.98+081729.1 | 21 37 04.98 | +08 17 29.19 | 4.03 | Pâris et al. (2012) |
| J021401.9−003941 | 21 40 01.90 | −00 39 41.00 | 4.17 | Khorunzhev et al. (2016) |
| SDSS J214045.65+091859.6 | 21 40 45.66 | +09 18 59.63 | 4.05 | Pâris et al. (2012) |
| SDSS J214217.26+000819.8 | 21 42 17.27 | +00 08 19.81 | 4.07 | Pâris et al. (2012) |
| J214239.27−012000.3 | 21 42 39.27 | −01 20 00.30 | 5.61 | Yang et al. (2017) |
| HRQC J214300.53−002024.6 | 21 43 00.53 | −00 20 24.60 | 4.84 | McGreer et al. (2013) |
| SDSS J214453.09+043410.0 | 21 44 53.10 | +04 34 10.06 | 4.11 | Pâris et al. (2012) |
| SDSS J214725.71−083834.6 | 21 47 25.71 | −08 38 34.70 | 4.59 | Schneider et al. (2005) |
| SDSS J21479+0107 | 21 47 55.40 | +01 07 55.00 | 5.81 | Jiang et al. (2009) |
| SDSS J214755.49+045716.6 | 21 47 55.50 | +04 57 16.65 | 4.08 | Pâris et al. (2012) |
| HRQC J215055.14−010439.8 | 21 50 55.14 | −01 04 39.80 | 4.73 | McGreer et al. (2013) |
| HRQC J215151.83−001711.1 | 21 51 51.83 | −00 17 11.10 | 4.66 | McGreer et al. (2013) |
| J215216.10+104052.44 | 21 52 16.10 | +10 40 52.44 | 4.79 | Wang et al. (2016) |
| PSS J2154+0335 | 21 54 06.73 | +03 35 40.00 | 4.36 | Péroux et al. (2001) |
| HRQC J215445.28+000421.7 | 21 54 45.28 | +00 04 21.70 | 4.74 | McGreer et al. (2013) |
| SDSS J215536.17+090309.3 | 21 55 36.17 | +09 03 09.34 | 4.03 | Pâris et al. (2017) |
| SDSS J215601.99−010258.5 | 21 56 01.99 | −01 02 58.56 | 4.14 | Pâris et al. (2012) |
| SDSS J215746.24+001701.0 | 21 57 46.25 | +00 17 01.01 | 4.16 | Pâris et al. (2012) |
| SDSS J215817.61−010555.0 | 21 58 17.62 | −01 05 55.00 | 4.13 | Pâris et al. (2017) |
| J215904.97+050745.76 | 21 59 04.97 | +05 07 45.76 | 4.71 | Wang et al. (2016) |
| SDSS J220008.66+001744.9 | 22 00 08.67 | +00 17 44.93 | 4.77 | Schneider et al. (2005) |
| J220106.63+030207.71 | 22 01 06.63 | +03 02 07.71 | 5.06 | Wang et al. (2016) |
| J2201+0155 | 22 01 32.07 | +01 55 29.00 | 6.16 | Matsuoka et al. (2018b) |
| IMS J220233+013120 | 22 02 33.20 | +01 31 20.30 | 5.21 | Kim et al. (2019) |
| SDSS J220237.95−010217.9 | 22 02 37.95 | −01 02 17.94 | 4.10 | Pâris et al. (2012) |
| SDSS J220307.39−004612.1 | 22 03 07.39 | −00 46 12.10 | 4.15 | Schneider et al. (2005) |
| SDSS J220402.13−084943.5 | 22 04 02.14 | −08 49 43.52 | 4.45 | Schneider et al. (2005) |
| SDSS J220407.49+054018.5 | 22 04 07.49 | +05 40 18.56 | 4.17 | Pâris et al. (2012) |
| IMS J2204+0012 | 22 04 17.92 | +01 11 44.80 | 5.94 | Kim et al. (2015) |
| IMS J220522+025730 | 22 05 22.15 | +02 57 30.00 | 4.74 | Kim et al. (2019) |
| IMS J220635+020136 | 22 06 34.81 | +02 01 36.30 | 5.10 | Kim et al. (2019) |
| J220710.12−041656.28 | 22 07 10.12 | −04 16 56.28 | 5.53 | Wang et al. (2016) |
| SDSS J220905.87+044647.6 | 22 09 05.87 | +04 46 47.65 | 4.92 | Pâris et al. (2014) |
| IMS J221004+025424 | 22 10 03.90 | +02 54 24.40 | 4.64 | Kim et al. (2019) |
| J2210+0304 | 22 10 27.24 | +03 04 28.50 | 6.90 | Chehade et al. (2018) |
| IMS J221037+024314 | 22 10 36.99 | +02 43 13.70 | 5.20 | Kim et al. (2019) |
| IMS J221118+031207 | 22 11 18.37 | +03 12 07.40 | 4.82 | Kim et al. (2019) |
| HRQC J221141.01+001118.9 | 22 11 41.01 | +00 11 18.90 | 5.23 | McGreer et al. (2013) |
| J221232.06+021200.09 | 22 12 32.06 | +02 12 00.09 | 4.61 | Wang et al. (2016) |
| SDSS J221251.49−004230.6 | 22 12 51.50 | −00 42 30.69 | 4.95 | Schneider et al. (2007) |
| IMS J221310−002428 | 22 13 09.67 | −00 24 28.10 | 4.80 | Kim et al. (2019) |

| | | | | |
|---|---|---|---|---|
| SDSS J221342.19+010913.3 | 22 13 42.20 | +01 09 13.40 | 4.06 | Pâris et al. (2017) |
| J221520.22−000908.39 | 22 15 20.22 | −00 09 08.39 | 5.28 | Ikeda et al. (2017) |
| IMS J221622+013815 | 22 16 21.85 | +01 38 14.70 | 4.93 | Kim et al. (2019) |
| SDSS J221644.01+001348.1 | 22 16 44.02 | +00 13 48.12 | 5.01 | Pâris et al. (2012) |
| HSC J2216−0016 | 22 16 44.47 | −00 16 50.10 | 6.10 | Matsuoka et al. (2016) |
| SDSS J221705.71−001307.6 | 22 17 05.71 | −00 13 07.64 | 4.67 | Schneider et al. (2007) |
| SDSS J221733.39−004225.8 | 22 17 33.40 | −00 42 25.80 | 4.12 | Pâris et al. (2017) |
| SDSS J221851.72−010259.1 | 22 18 51.73 | −01 02 59.14 | 4.71 | Pâris et al. (2012) |
| VIMOS2911001793 | 22 19 17.22 | +01 02 48.90 | 6.16 | Kashikawa et al. (2015) |
| J221921.74+144126.31 | 22 19 21.74 | +14 41 26.31 | 4.59 | Wang et al. (2016) |
| SDSS J222018.50−010147.0 | 22 20 18.50 | −01 01 47.09 | 5.61 | Pâris et al. (2017) |
| SDSS J222050.80+001959.1 | 22 20 50.81 | +00 19 59.16 | 4.68 | Pâris et al. (2017) |
| HRQC J222216.02−000405.6 | 22 22 16.02 | −00 04 05.60 | 4.95 | McGreer et al. (2013) |
| SDSS J222249.11+000504.5 | 22 22 49.11 | +00 05 04.56 | 4.26 | Pâris et al. (2012) |
| J2223+0326 | 22 23 09.51 | +03 26 20.30 | 6.05 | Chehade et al. (2018) |
| SDSS J222509.19−001406.8 | 22 25 09.19 | −00 14 06.82 | 4.85 | Schneider et al. (2005) |
| J222514.38+033012.50 | 22 25 14.38 | +03 30 12.50 | 5.24 | Wang et al. (2016) |
| J222612.41−061807.29 | 22 26 12.41 | −06 18 07.29 | 5.08 | Wang et al. (2016) |
| SDSS J222612.99−003058.8 | 22 26 12.99 | −00 30 58.83 | 4.01 | Pâris et al. (2012) |
| HRQC J222629.28−010956.5 | 22 26 29.28 | −01 09 56.50 | 4.99 | McGreer et al. (2013) |
| SDSS J222807.57+003526.3 | 22 28 07.58 | +00 35 26.31 | 4.55 | Schneider et al. (2007) |
| HSC J2228+0128 | 22 28 27.83 | +01 28 09.50 | 6.01 | Matsuoka et al. (2016) |
| SDSS J222843.54+011032.2 | 22 28 43.54 | +01 10 32.20 | 5.95 | Zeimann et al. (2011) |
| SDSS J222845.14−075755.3 | 22 28 45.15 | −07 57 55.38 | 5.14 | Schneider et al. (2005) |
| J2228+0152 | 22 28 47.71 | +01 52 40.50 | 6.08 | Matsuoka et al. (2018b) |
| J2231−0035 | 22 31 48.89 | −00 35 47.50 | 5.87 | Chehade et al. (2018) |
| HSC J2232+0012 | 22 32 12.03 | +00 12 38.40 | 6.18 | Matsuoka et al. (2016) |
| HRQC J223327.64−010704.4 | 22 33 27.64 | −01 07 04.40 | 5.11 | McGreer et al. (2013) |
| SDSS J223338.57−011137.5 | 22 33 38.58 | −01 11 37.54 | 4.53 | Pâris et al. (2012) |
| SDSS J223414.83+074733.0 | 22 34 14.84 | +07 47 33.09 | 4.04 | Pâris et al. (2017) |
| SDSS J223521.22−082127.2 | 22 35 21.23 | −08 21 27.24 | 4.43 | Schneider et al. (2005) |
| SDSS J223546.47+062325.0 | 22 35 46.48 | +06 23 25.09 | 4.05 | Pâris et al. (2017) |
| HSC J2236+0032 | 22 36 44.58 | +00 32 56.90 | 6.40 | Matsuoka et al. (2016) |
| HRQC J223653.26+002603.0 | 22 36 53.26 | +00 26 03.00 | 4.70 | McGreer et al. (2013) |
| BRI 2235−0301 | 22 38 22.53 | −02 45 53.00 | 4.25 | Smith et al. (1994b) |
| SDSS J223828.65+084242.0 | 22 38 28.65 | +08 42 42.05 | 4.07 | Pâris et al. (2017) |
| HRQC J223850.20−002701.8 | 22 38 50.20 | −00 27 01.80 | 5.17 | McGreer et al. (2013) |
| SDSS J223853.54−010313.5 | 22 38 53.54 | −01 03 13.50 | 4.22 | Pâris et al. (2012) |
| SDSS J223859.79+005623.6 | 22 38 59.79 | +00 56 23.68 | 4.88 | Pâris et al. (2012) |
| HRQC J223925.51+004337.7 | 22 39 25.51 | +00 43 37.70 | 4.53 | McGreer et al. (2013) |
| J2239+0207 | 22 39 47.47 | +02 07 47.50 | 6.26 | Matsuoka et al. (2018b) |
| BR 2237−0607 | 22 39 53.67 | −05 52 20.00 | 4.55 | Constantin et al. (2002) |
| HRQC J224206.52+002523.9 | 22 42 06.52 | +00 25 23.90 | 4.78 | McGreer et al. (2013) |
| SDSS J224206.89−005151.8 | 22 42 06.89 | −00 51 51.85 | 4.01 | Schneider et al. (2007) |
| CFHQS J2242+0334 | 22 42 37.53 | +03 34 22.00 | 5.88 | Willott et al. (2010a) |
| SDSS J224243.03−091543.9 | 22 42 43.03 | −09 15 43.92 | 4.21 | Schneider et al. (2005) |
| SDSS J224255.53+124225.7 | 22 42 55.53 | +12 42 25.77 | 4.44 | Pâris et al. (2017) |
| SDSS J224343.17+093735.0 | 22 43 43.18 | +09 37 35.03 | 4.06 | Pâris et al. (2017) |
| Q J2245+0033 | 22 45 31.00 | +00 33 58.00 | 4.45 | Sharp et al. (2001) |
| SDSS J224605.45+072356.8 | 22 46 05.46 | +07 23 56.84 | 4.23 | Pâris et al. (2017) |
| SDSS J224721.05−091548.6 | 22 47 21.06 | −09 15 48.65 | 4.13 | Schneider et al. (2005) |
| SDSS J224737.98−084225.7 | 22 47 37.99 | −08 42 25.76 | 4.08 | Schneider et al. (2005) |
| SDSS J224740.17−091511.7 | 22 47 40.17 | −09 15 11.71 | 4.17 | Schneider et al. (2005) |
| SDSS J224748.91+100536.0 | 22 47 48.91 | +10 05 36.10 | 4.07 | Pâris et al. (2014) |
| SDSS J224937.79+113608.7 | 22 49 37.80 | +11 36 08.79 | 4.04 | Pâris et al. (2017) |
| SDSS J224941.35+001556.6 | 22 49 41.36 | +00 15 56.62 | 4.13 | Pâris et al. (2012) |
| DMS 2247−0209 | 22 49 52.13 | −01 53 32.00 | 4.34 | Hall et al. (1996) |

| | | | | |
|---|---|---|---|---|
| SDSS J225153.72+050028.0 | 22 51 53.73 | +05 00 28.05 | 4.32 | Pâris et al. (2014) |
| J2252+0225 | 22 52 05.44 | +02 25 31.90 | 6.12 | Chehade et al. (2018) |
| SDSS J225246.02−005644.4 | 22 52 46.02 | −00 56 44.49 | 4.09 | Pâris et al. (2017) |
| SDSS J225426.66+000750.4 | 22 54 26.66 | +00 07 50.45 | 4.44 | Pâris et al. (2017) |
| SDSS J225448.40−005309.9 | 22 54 48.40 | −00 53 09.96 | 4.08 | Pâris et al. (2012) |
| J2255+0251 | 22 55 38.04 | +02 51 26.60 | 6.34 | Chehade et al. (2018) |
| SDSS J225624.34+004720.2 | 22 56 24.34 | +00 47 20.22 | 4.10 | Schneider et al. (2007) |
| SDSS J225812.62+001950.7 | 22 58 12.63 | +00 19 50.72 | 4.15 | Pâris et al. (2012) |
| SDSS J225843.27−092710.5 | 22 58 43.28 | −09 27 10.59 | 4.07 | Schneider et al. (2005) |
| SDSS J225910.27+005103.6 | 22 59 10.27 | +00 51 03.62 | 4.10 | Pâris et al. (2012) |
| PS1 J225944.26+093624.42 | 22 59 44.26 | +09 36 24.42 | 4.87 | Yang et al. (2018) |
| SDSS J230320.38−085433.1 | 23 03 20.39 | −08 54 33.14 | 4.31 | Schneider et al. (2005) |
| SDSS J230333.41+010405.0 | 23 03 33.41 | +01 04 05.04 | 4.12 | Pâris et al. (2012) |
| HRQC J230413.47−011149.2 | 23 04 13.47 | −01 11 49.20 | 4.75 | McGreer et al. (2013) |
| J2304+0045 | 23 04 22.97 | +00 45 05.40 | 6.36 | Chehade et al. (2018) |
| SDSS J230451.68+005135.1 | 23 04 51.68 | +00 51 35.15 | 4.17 | Pâris et al. (2012) |
| SDSS J23075+0031 | 23 07 35.40 | +00 31 49.00 | 5.87 | Jiang et al. (2009) |
| SDSS J230916.77+001002.5 | 23 09 16.77 | +00 10 02.58 | 4.73 | Pâris et al. (2012) |
| HRQC J231000.37−004327.0 | 23 10 00.37 | −00 43 27.00 | 4.83 | McGreer et al. (2013) |
| SDSS J231010.59−100653.9 | 23 10 10.59 | −10 06 53.98 | 4.53 | Schneider et al. (2005) |
| SDSS J231216.43+010051.6 | 23 12 16.44 | +01 00 51.63 | 5.07 | Pâris et al. (2012) |
| SDSS J231452.34+004237.1 | 23 14 52.34 | +00 42 37.14 | 4.47 | Pâris et al. (2012) |
| SDSS J23157−0023 | 23 15 46.60 | −00 23 58.00 | 6.12 | Jiang et al. (2008) |
| PSS J2315+0921 | 23 15 59.13 | +09 21 43.00 | 4.41 | Péroux et al. (2001) |
| SDSS J231701.01+003205.6 | 23 17 01.01 | +00 32 05.66 | 4.68 | Pâris et al. (2012) |
| CFHSQ J23180−0246 | 23 18 02.80 | −02 46 34.00 | 6.05 | Willott et al. (2009) |
| HRQC J232006.60−001822.3 | 23 20 06.60 | −00 18 22.30 | 4.80 | McGreer et al. (2013) |
| SDSS J232112.40+143312.0 | 23 21 12.41 | +14 33 12.01 | 4.05 | Schneider et al. (2005) |
| SDSS J232513.15−094049.2 | 23 25 13.15 | −09 40 49.30 | 4.01 | Schneider et al. (2005) |
| SDSS J232531.83+061459.2 | 23 25 31.84 | +06 14 59.24 | 4.07 | Pâris et al. (2014) |
| J232536.64−055328.3 | 23 25 36.64 | −05 53 28.30 | 5.22 | Yang et al. (2017) |
| SDSS J232808.99−002757.4 | 23 28 08.99 | −00 27 57.49 | 4.13 | Pâris et al. (2012) |
| CFHQS J23291−0301 | 23 29 08.33 | −03 01 59.00 | 6.43 | Willott et al. (2007) |
| CFHQS J23292−0403 | 23 29 14.53 | −04 03 24.00 | 5.90 | Willott et al. (2009) |
| J233008.71+095743.7 | 23 30 08.71 | +09 57 43.70 | 5.30 | Yang et al. (2017) |
| SDSS J233104.34+123442.7 | 23 31 04.34 | +12 34 42.74 | 4.10 | Pâris et al. (2017) |
| SDSS J233106.06+061812.6 | 23 31 06.07 | +06 18 12.69 | 4.59 | Ahn et al. (2014) |
| SDSS J233223.57+010253.6 | 23 32 23.58 | +01 02 53.62 | 4.81 | Pâris et al. (2012) |
| SDSS J233250.46+062449.2 | 23 32 50.46 | +06 24 49.23 | 4.06 | Pâris et al. (2014) |
| SDSS J233255.72+141916.4 | 23 32 55.73 | +14 19 16.42 | 4.72 | Pâris et al. (2017) |
| SDSS J233333.67−091217.3 | 23 33 33.68 | −09 12 17.39 | 4.03 | Schneider et al. (2005) |
| SDSS J233427.52+030528.6 | 23 34 27.53 | +03 05 28.69 | 4.13 | Pâris et al. (2017) |
| HRQC J233428.47−005207.7 | 23 34 28.47 | −00 52 07.70 | 4.77 | McGreer et al. (2013) |
| HRQC J233455.05−001022.1 | 23 34 55.05 | −00 10 22.10 | 5.11 | McGreer et al. (2013) |
| SDSS J233506.17+024632.5 | 23 35 06.17 | +02 46 32.56 | 4.22 | Pâris et al. (2014) |
| SDSS J233509.91+010938.8 | 23 35 09.92 | +01 09 38.84 | 4.04 | Pâris et al. (2012) |
| SDSS J233610.47−005814.8 | 23 36 10.48 | −00 58 14.86 | 4.52 | Schneider et al. (2007) |
| SDSS J233928.27+005906.4 | 23 39 28.27 | +00 59 06.41 | 4.09 | Schneider et al. (2007) |
| SDSS J233938.57+104039.0 | 23 39 38.57 | +10 40 39.03 | 4.17 | Pâris et al. (2017) |
| SDSS J234017.18−002659.3 | 23 40 17.19 | −00 26 59.35 | 4.20 | Pâris et al. (2012) |
| SDSS J234128.92−091610.6 | 23 41 28.92 | −09 16 10.61 | 4.13 | Schneider et al. (2005) |
| HRQC J234206.94+003614.1 | 23 42 06.94 | +00 36 14.10 | 4.74 | McGreer et al. (2013) |
| PSS J2344+0342 | 23 44 03.13 | +03 42 27.00 | 4.24 | Péroux et al. (2001) |
| SDSS J234600.20−000238.8 | 23 46 00.21 | −00 02 38.81 | 4.41 | Pâris et al. (2012) |
| HRQC J234601.55−003855.2 | 23 46 01.55 | −00 38 55.20 | 4.93 | McGreer et al. (2013) |
| SDSS J234620.76+065158.6 | 23 46 20.76 | +06 51 58.64 | 4.25 | Pâris et al. (2017) |
| SDSS J234645.57−005859.0 | 23 46 45.58 | −00 58 59.04 | 4.02 | Schneider et al. (2007) |

| | | | | |
|---|---|---|---|---|
| HRQC J234730.56+002306.3 | 23 47 30.56 | +00 23 06.30 | 4.71 | McGreer et al. (2013) |
| SDSS J234847.71+053043.9 | 23 48 47.72 | +05 30 43.91 | 4.04 | Pâris et al. (2017) |
| PSO J357.8289+06.4019 | 23 51 18.96 | +06 24 06.92 | 5.81 | Bañados et al. (2016) |
| J235124.31−045907.3 | 23 51 24.31 | −04 59 07.30 | 5.25 | Yang et al. (2017) |
| SDSS J235344.26+143525.3 | 23 53 44.26 | +14 35 25.33 | 4.24 | Pâris et al. (2017) |
| SDSS J235457.96+082804.2 | 23 54 57.97 | +08 28 04.20 | 4.18 | Pâris et al. (2017) |
| PSO J359.1352−06.3831 | 23 56 32.45 | −06 22 59.26 | 6.15 | Bañados et al. (2016) |
| SDSS J23568+0023 | 23 56 51.60 | +00 23 33.00 | 6.00 | Jiang et al. (2009) |
| SDSS J235700.23+034511.3 | 23 57 00.24 | +03 45 11.37 | 4.15 | Pâris et al. (2012) |
| SDSS J235718.36+004350.3 | 23 57 18.36 | +00 43 50.35 | 4.37 | Schneider et al. (2005) |
| J235824.04+063437.4 | 23 58 24.04 | +06 34 37.40 | 5.32 | Yang et al. (2017) |

## REFERENCES


Abazajian K., et al., 2004, AJ, 128, 502
Ahn C. P., et al., 2014, ApJS, 211, 17
Anderson S. F., et al., 2001, AJ, 122, 503
Bañados E., et al., 2014, AJ, 148, 14
Bañados E., et al., 2016, ApJS, 227, 11
Bañados E., et al., 2018, Natur, 553, 473
Barger A. J., Cowie L. L., Brandt W. N., Capak P., Garmire G. P., Hornschemeier A. E., Steffen A. T., Wehner E. H., 2002, AJ, 124, 1839
Boutsia K., Grazian A., Giallongo E., Fiore F., Civano F., 2018, ApJ, 869, 20
Bovy J., et al., 2011, ApJ, 729, 141
Chehade B., et al., 2018, MNRAS, 478, 1649
Chiu K., et al., 2005, AJ, 130, 13
Collinge M. J., et al., 2005, AJ, 129, 2542
Constantin A., Shields J. C., Hamann F., Foltz C. B., Chaffee F. H., 2002, ApJ, 565, 50
Cool R. J., et al., 2006, AJ, 132, 823
Croom S. M., et al., 2009, MNRAS, 392, 19
De Rosa G., Decarli R., Walter F., Fan X., Jiang L., Kurk J., Pasquali A., Rix H. W., 2011, ApJ, 739, 56
Dietrich M., Appenzeller I., Hamann F., Heidt J., Jäger K., Vestergaard M., Wagner S. J., 2003, A&A, 398, 891
Djorgovski S. G., Mahabal A. A., Brunner R. J., Gal R. R., Castro S., de Carvalho R. R., Odewahn S. C., 2001, ASPC, 225, 52
Djorgovski S. G., Stern D., Mahabal A. A., Brunner R., 2003, ApJ, 596, 67
Eckart M. E., Stern D., Helfand D. J., Harrison F. A., Mao P. H., Yost S. A., 2006, ApJS, 165, 19
Esquej P., et al., 2013, A&A, 557, A123
Fan X., et al., 2000, AJ, 119, 1
Fan X., et al., 2000, AJ, 120, 1167
Fan X., et al., 2001, AJ, 122, 2833
Fan X., et al., 2001, AJ, 121, 31
Fan X., et al., 2003, AJ, 125, 1649
Fan X., et al., 2004, AJ, 128, 515
Fan X., et al., 2006, AJ, 131, 1203
Glikman E., Djorgovski S. G., Stern D., Bogosavljević M., Mahabal A., 2007, ApJ, 663, L73
Glikman E., Bogosavljević M., Djorgovski S. G., Stern D., Dey A., Jannuzi B. T., Mahabal A., 2010, ApJ, 710, 1498
Goto T., 2006, MNRAS, 371, 769
Hall P. B., Osmer P. S., Green R. F., Porter A. C., Warren S. J., 1996, ApJ, 462, 614
Hall P. B., et al., 2000, AJ, 120, 2220
Hennawi J. F., et al., 2010, ApJ, 719, 1672
Hiroi K., Ueda Y., Akiyama M., Watson M. G., 2012, ApJ, 758, 49
Ikeda H., Nagao T., Matsuoka K., Kawakatu N., KAJ,isawa M., Akiyama M., MiyAJ,i T., Morokuma T., 2017, ApJ, 846, 57
Jiang L., et al., 2006, AJ, 131, 2788
Jiang L., et al., 2008, AJ, 135, 1057
Jiang L., et al., 2009, AJ, 138, 305
Jiang L., McGreer I. D., Fan X., Bian F., Cai Z., Clément B., Wang R., Fan Z., 2015, AJ, 149, 188
Jiang L., et al., 2016, ApJ, 833, 222
Kashikawa N., et al., 2015, ApJ, 798, 28
Kennefick J. D., de Carvalho R. R., Djorgovski S. G., Wilber M. M., Dickson E. S., Weir N., Fayyad U., Roden J., 1995, AJ, 110, 78
Kennefick J. D., Djorgovski S. G., de Carvalho R. R., 1995, AJ, 110, 2553
Kennefick J. D., Djorgovski S. G., Meylan G., 1996, AJ, 111, 1816
Khorunzhev G. A., Burenin R. A., Meshcheryakov A. V., Sazonov S. Y., 2016, AstL, 42, 277
Khorunzhev G. A., Burenin R. A., Sazonov S. Y., Amvrosov A. L., Eselevich M. V., 2017, AstL, 43, 135
Kim Y., et al., 2015, ApJ, 813, L35
Kim Y., et al., 2019, ApJ, 870, 86
Kochanek C. S., et al., 2012, ApJS, 200, 8
Lacy M., Petric A. O., SAJ,ina A., Canalizo G., Storrie-Lombardi L. J., Armus L., Fadda D., Marleau F. R., 2007, AJ, 133, 186
Mahabal A., Stern D., Bogosavljević M., Djorgovski S. G., Thompson D., 2005, ApJ, 634, L9
Martínez-Sansigre A., Rawlings S., Lacy M., Fadda D., Jarvis M. J., Marleau F. R., Simpson C., Willott C. J., 2006, MNRAS, 370, 1479
Martini P., Mulchaey J. S., Kelson D. D., 2007, ApJ, 664, 761
Masters D., et al., 2012, ApJ, 755, 169
Matsuoka Y., et al., 2016, ApJ, 828, 26
Matsuoka Y., et al., 2018, ApJS, 237, 5
Matsuoka Y., et al., 2018, PASJ, 70, S35
Matute I., et al., 2013, A&A, 557, A78
Mazzucchelli C., et al., 2017, ApJ, 849, 91
McGreer I. D., et al., 2013, ApJ, 768, 105
Monier E. M., Kennefick J. D., Hall P. B., Osmer P. S., Smith M. G., Dalton G. B., Green R. F., 2002, AJ, 124, 2971
Mortlock D. J., et al., 2009, A&A, 505, 97
Mortlock D. J., et al., 2011, Natur, 474, 616
Newman J. A., et al., 2013, ApJS, 208, 5
Pâris I., et al., 2012, A&A, 548, A66
Pâris I., et al., 2014, A&A, 563, A54
Pâris I., et al., 2017, A&A, 597, A79
Péroux C., Storrie-Lombardi L. J., McMahon R. G., Irwin M., Hook I. M., 2001, AJ, 121, 1799
Papovich C., et al., 2006, AJ, 132, 231
Polsterer K. L., Zinn P.-C., Gieseke F., 2013, MNRAS, 428, 226
Prochaska J. X., et al., 2013, ApJ, 776, 136
Prochaska J. X., Castro S., Djorgovski S. G., 2003, ApJS, 148, 317
Rabbette M., McBreen B., Smith N., Steel S., 1998, AnAS, 129, 445
Richards G. T., et al., 2006, AJ, 131, 49
Schmidt M., Schneider D. P., Gunn J. E., 1987, ApJ, 321, L7
Schneider D. P., Schmidt M., Hasinger G., Lehmann I., Gunn J. E., Giacconi R., Trümper J., Zamorani G., 1998, AJ, 115, 1230
Schneider D. P., et al., 2000, AJ, 120, 2183
Schneider D. P., et al., 2001, AJ, 121, 1232
Schneider D. P., et al., 2005, AJ, 130, 367
Schneider D. P., et al., 2007, AJ, 134, 102
Schneider D. P., et al., 2010, AJ, 139, 2360
Schneider D. P., Schmidt M., Gunn J. E., 1989, AJ, 98, 1507
Schneider D. P., Schmidt M., Gunn J. E., 1989, AJ, 98, 1951
Schneider D. P., Schmidt M., Gunn J. E., 1991, AJ, 102, 837
Schneider D. P., Schmidt M., Gunn J. E., 1994, AJ, 107, 880
Schneider D. P., Schmidt M., Gunn J. E., 1994, AJ, 107, 1245
Schneider D. P., Schmidt M., Gunn J. E., 1997, AJ, 114, 36
Sharp R. G., McMahon R. G., Irwin M. J., Hodgkin S. T., 2001, MNRAS, 326, L45
Silverman J. D., et al., 2005, ApJ, 618, 123
Smith J. D., Thompson D., Djorgovski S., 1994, AJ, 107, 24
Smith J. D., et al., 1994, AJ, 108, 1147
Steffen A. T., Barger A. J., Capak P., Cowie L. L., Mushotzky R. F., Yang Y., 2004, AJ, 128, 1483
Stern D., Spinrad H., Eisenhardt P., Bunker A. J., Dawson S., Stanford S. A., Elston R., 2000, ApJ, 533, L75
Storrie-Lombardi L. J., McMahon R. G., Irwin M. J., Hazard C., 1996, ApJ, 468, 121
Storrie-Lombardi L. J., Irwin M. J., McMahon R. G., Hook I. M., 2001, MNRAS, 322, 933
Trichas M., et al., 2012, ApJS, 200, 17
Trouille L., Barger A. J., Cowie L. L., Yang Y., Mushotzky R. F., 2008, ApJS, 179, 1

Trump J. R., et al., 2006, ApJS, 165, 1
Trump J. R., et al., 2009, ApJ, 696, 1195
Venemans B. P., McMahon R. G., Warren S. J., Gonzalez-Solares E. A., Hewett P. C., Mortlock D. J., Dye S., Sharp R. G., 2007, MNRAS, 376, L76
Venemans B. P., et al., 2015, ApJ, 801, L11
Venemans B. P., et al., 2015, MNRAS, 453, 2259
Wang R., et al., 2008, ApJ, 687, 848
Wang F., et al., 2016, ApJ, 819, 24
Wang F., et al., 2017, ApJ, 839, 27
Wang F., et al., 2018, arXiv, arXiv:1810.11926
Willott C. J., et al., 2007, AJ, 134, 2435
Willott C. J., et al., 2009, AJ, 137, 3541
Willott C. J., et al., 2010, AJ, 139, 906
Willott C. J., et al., 2010, AJ, 140, 546
Wu X.-B., et al., 2012, RAA, 12, 1185
Yang J., et al., 2017, AJ, 153, 184
Yang J., et al., 2018, arXiv, arXiv:1810.11927
Yi W., et al., 2017, ApJ, 838, 135
Zeimann G. R., White R. L., Becker R. H., Hodge J. A., Stanford S. A., Richards G. T., 2011, ApJ, 736, 57
Zheng W., et al., 2000, AJ, 120, 1607
